# Supplementary material for: State-Specific Coupled-Cluster Methods for Excited States
Source: arXiv:2401.05048 ancillary file (2024-03-08)
Supplement: Supplementary file 1 [file supp_inf_state_specific_cc.pdf]

# Supporting Information for "State-Specific Coupled-Cluster Methods for Excited States"

Yann Damour,[1, a)] Anthony Scemama,[1] Denis Jacquemin,[2,3] Fábris Kossoski,[1, b)] and Pierre-François Loos[1, c)]
[1)]*Laboratoire de Chimie et Physique Quantiques (UMR 5626), Université de Toulouse, CNRS, UPS, France*
[2)]*Nantes Université, CNRS, CEISAM UMR 6230, F-44000 Nantes, France*
[3)]*Institut Universitaire de France (IUF), F-75005 Paris, France*

## S1. ADDITIONAL GEOMETRIES (IN BOHR)

### A. Borole

```
B  0.00000000   0.00000000   2.44991435
C  0.00000000   2.35991046   0.62561328
C  0.00000000  -2.35991046   0.62561328
C  0.00000000   1.42526648  -1.74135978
C  0.00000000  -1.42526648  -1.74135978
H  0.00000000   0.00000000   4.69246473
H  0.00000000   4.35732912   1.03002724
H  0.00000000  -4.35732912   1.03002724
H  0.00000000   2.51021632  -3.47247633
H  0.00000000  -2.51021632  -3.47247633
```

### B. Oxalyl fluoride

```
C  -1.39903565   0.34476183  0.00000000
C   1.39903565  -0.34476183  0.00000000
O  -2.24825627   2.40855549  0.00000000
O   2.24825627  -2.40855549  0.00000000
F  -2.78737061  -1.74488227  0.00000000
F   2.78737061   1.74488227  0.00000000
```

[a)]Electronic mail: yann.damour@irsamc.ups-tlse.fr
[b)]Electronic mail: fabris.kossoski@irsamc.ups-tlse.fr
[c)]Electronic mail: loos@irsamc.ups-tlse.fr

TABLE S1. Statistical measures associated with the errors in the excitation energies of open-shell singly-excited states, in units of eV, computed with EOM-CC2, EOM-CCSD, HF-ΔCCSD, oo-ΔCCSD, and ΔCISD. Values in parenthesis are obtained by discarding states with four dominant determinants with the exact same weight in the EOM-CCSD vector.

| Method | Character | no. states | MAE | MSE | RMSE | SDE |
|---|---|---|---|---|---|---|
| EOM-CC2 | $n\pi^*$ | 56 | 0.11 | 0.04 | 0.18 | 0.17 |
| | $\pi\pi^*$ | 77 (58) | 0.20 (0.18) | 0.18 ( 0.16) | 0.25 (0.24) | 0.17 (0.18) |
| | $\sigma\pi^*$ | 18 | 0.07 | 0.02 | 0.08 | 0.08 |
| | $n$-Rydberg | 38 | 0.38 | -0.35 | 0.45 | 0.28 |
| | $\pi$-Rydberg | 42 | 0.06 | -0.01 | 0.08 | 0.08 |
| EOM-CCSD | $n\pi^*$ | 56 | 0.08 | 0.04 | 0.16 | 0.16 |
| | $\pi\pi^*$ | 77 (58) | 0.10 (0.10) | 0.05 ( 0.06) | 0.13 (0.14) | 0.12 (0.13) |
| | $\sigma\pi^*$ | 18 | 0.04 | 0.02 | 0.05 | 0.05 |
| | $n$-Rydberg | 38 | 0.07 | 0.01 | 0.09 | 0.09 |
| | $\pi$-Rydberg | 42 | 0.09 | 0.09 | 0.10 | 0.05 |
| HF-ΔCCSD | $n\pi^*$ | 56 | 0.11 | -0.01 | 0.22 | 0.22 |
| | $\pi\pi^*$ | 77 (58) | 0.31 (0.19) | 0.13 ( 0.06) | 0.46 (0.29) | 0.45 (0.28) |
| | $\sigma\pi^*$ | 18 | 0.07 | 0.00 | 0.09 | 0.09 |
| | $n$-Rydberg | 38 | 0.19 | -0.12 | 0.49 | 0.47 |
| | $\pi$-Rydberg | 42 | 0.05 | -0.03 | 0.07 | 0.06 |
| oo-ΔCCSD | $n\pi^*$ | 56 | 0.13 | -0.04 | 0.21 | 0.21 |
| | $\pi\pi^*$ | 77 (58) | 0.23 (0.15) | 0.11 ( 0.00) | 0.39 (0.26) | 0.37 (0.26) |
| | $\sigma\pi^*$ | 18 | 0.07 | -0.01 | 0.09 | 0.09 |
| | $n$-Rydberg | 38 | 0.09 | -0.02 | 0.12 | 0.12 |
| | $\pi$-Rydberg | 42 | 0.09 | -0.00 | 0.18 | 0.18 |
| ΔCISD | $n\pi^*$ | 56 | 0.18 | -0.14 | 0.24 | 0.19 |
| | $\pi\pi^*$ | 77 (58) | 0.25 (0.23) | -0.13 (-0.10) | 0.30 (0.28) | 0.27 (0.26) |
| | $\sigma\pi^*$ | 18 | 0.13 | -0.10 | 0.15 | 0.12 |
| | $n$-Rydberg | 38 | 0.12 | -0.04 | 0.18 | 0.17 |
| | $\pi$-Rydberg | 42 | 0.11 | -0.09 | 0.14 | 0.11 |

TABLE S2. Statistical measures associated with the errors in the excitation energies of open-shell singly-excited states, in units of eV, computed with EOM-CC2, EOM-CCSD, HF-ΔCCSD, oo-ΔCCSD, and ΔCISD. Values in parenthesis are obtained by discarding states with four dominant determinants with the exact same weight in the EOM-CCSD vector.

| Method | System size | no. states | MAE | MSE | RMSE | SDE |
|---|---|---|---|---|---|---|
| EOM-CC2 | 1-2 non-H atoms | 66 ( 54) | 0.22 (0.20) | -0.04 (-0.11) | 0.29 (0.29) | 0.29 (0.27) |
| | 3-4 non-H atoms | 120 (117) | 0.17 (0.16) | 0.01 ( 0.01) | 0.24 (0.24) | 0.24 (0.24) |
| | 5-6 non-H atoms | 45 ( 41) | 0.12 (0.11) | 0.08 ( 0.07) | 0.20 (0.19) | 0.18 (0.18) |
| EOM-CCSD | 1-2 non-H atoms | 66 ( 54) | 0.06 (0.06) | 0.01 ( 0.01) | 0.07 (0.07) | 0.07 (0.07) |
| | 3-4 non-H atoms | 120 (117) | 0.09 (0.09) | 0.05 ( 0.05) | 0.15 (0.15) | 0.14 (0.14) |
| | 5-6 non-H atoms | 45 ( 41) | 0.10 (0.10) | 0.08 ( 0.08) | 0.11 (0.11) | 0.08 (0.08) |
| HF-ΔCCSD | 1-2 non-H atoms | 66 ( 54) | 0.23 (0.14) | -0.04 (-0.09) | 0.49 (0.38) | 0.49 (0.37) |
| | 3-4 non-H atoms | 120 (117) | 0.15 (0.13) | 0.03 ( 0.01) | 0.27 (0.23) | 0.26 (0.23) |
| | 5-6 non-H atoms | 45 ( 41) | 0.16 (0.12) | 0.07 ( 0.02) | 0.31 (0.26) | 0.31 (0.26) |
| oo-ΔCCSD | 1-2 non-H atoms | 66 ( 54) | 0.13 (0.09) | 0.01 (-0.05) | 0.24 (0.11) | 0.24 (0.10) |
| | 3-4 non-H atoms | 120 (117) | 0.15 (0.13) | -0.01 (-0.03) | 0.27 (0.23) | 0.27 (0.23) |
| | 5-6 non-H atoms | 45 ( 41) | 0.16 (0.11) | 0.12 ( 0.08) | 0.27 (0.19) | 0.24 (0.17) |
| ΔCISD | 1-2 non-H atoms | 66 ( 54) | 0.17 (0.12) | -0.15 (-0.09) | 0.22 (0.15) | 0.17 (0.13) |
| | 3-4 non-H atoms | 120 (117) | 0.19 (0.19) | -0.13 (-0.14) | 0.25 (0.25) | 0.21 (0.21) |
| | 5-6 non-H atoms | 45 ( 41) | 0.15 (0.15) | 0.01 (-0.01) | 0.22 (0.21) | 0.22 (0.21) |

## S2. TD-CCSD WITH ACTIVE ORBITALS OF DIFFERENT SPATIAL SYMMETRY

In contrast to the notation employed in the paper, and for the sake of simplicity, the labels without a bar denote spin-up orbitals, while those with a bar denote spin-down orbitals.

### A. $M_i^a$ contributions

$$\begin{aligned} M_i^a =& [- {}^A t_{\bar{n}}^{\bar{a}} \, {}^A t_{m\bar{i}}^{n\bar{m}} - {}^A t_{\bar{i}}^{\bar{m}} \, {}^A t_{m\bar{n}}^{n\bar{a}}] \\ &+ \delta(n, a) \, [- {}^A t_{m\bar{i}}^{n\bar{m}}] \\ &+ \delta(m, i) \, [+ {}^A t_{m\bar{n}}^{n\bar{a}}] \end{aligned} \tag{S1}$$

$$M_i^{\bar{a}} = 0 \tag{S2}$$

$$M_{\bar{i}}^{a} = 0 \tag{S3}$$

$$\begin{aligned} M_{\bar{i}}^{\bar{a}} =& [- {}^A t_{m}^{a} \, {}^A t_{i\bar{n}}^{n\bar{m}} - {}^A t_{i}^{n} \, {}^A t_{m\bar{n}}^{a\bar{m}}] \\ &+ \delta(\bar{m}, \bar{a}) \, [- {}^A t_{i\bar{n}}^{n\bar{m}}] \\ &+ \delta(\bar{n}, \bar{i}) \, [+ {}^A t_{m\bar{n}}^{a\bar{m}}] \end{aligned} \tag{S4}$$

### B. $M_{ij}^{ab}$ connected contributions

$$
\begin{aligned}
M_{ij}^{ab} =&[- {}^{A}t^{\bar{a}\bar{b}}_{\bar{n}\bar{j}}\, {}^{A}t^{n\bar{m}}_{m\bar{i}} + {}^{A}t^{\bar{a}\bar{b}}_{\bar{n}\bar{i}}\, {}^{A}t^{n\bar{m}}_{m\bar{j}} + {}^{A}t^{n\bar{a}}_{m\bar{j}}\, {}^{A}t^{\bar{b}\bar{m}}_{\bar{n}\bar{i}} - {}^{A}t^{n\bar{a}}_{m\bar{i}}\, {}^{A}t^{\bar{b}\bar{m}}_{\bar{n}\bar{j}} + {}^{A}t^{n\bar{a}}_{m\bar{n}}\, {}^{A}t^{\bar{b}\bar{m}}_{\bar{i}\bar{j}} \\
&- {}^{A}t^{\bar{a}\bar{m}}_{\bar{i}\bar{j}}\, {}^{A}t^{n\bar{b}}_{m\bar{n}} + {}^{A}t^{\bar{a}\bar{m}}_{\bar{n}\bar{j}}\, {}^{A}t^{n\bar{b}}_{m\bar{i}} - {}^{A}t^{\bar{a}\bar{m}}_{\bar{n}\bar{i}}\, {}^{A}t^{n\bar{b}}_{m\bar{j}} + {}^{A}t^{\bar{a}}_{\bar{n}}\, {}^{A}t^{\bar{m}}_{\bar{j}}\, {}^{A}t^{n\bar{b}}_{m\bar{i}} - {}^{A}t^{\bar{a}}_{\bar{n}}\, {}^{A}t^{\bar{m}}_{\bar{i}}\, {}^{A}t^{n\bar{b}}_{m\bar{j}} \\
&- {}^{A}t^{\bar{b}}_{\bar{n}}\, {}^{A}t^{\bar{m}}_{\bar{j}}\, {}^{A}t^{n\bar{a}}_{m\bar{i}} + {}^{A}t^{\bar{b}}_{\bar{n}}\, {}^{A}t^{\bar{m}}_{\bar{i}}\, {}^{A}t^{n\bar{a}}_{m\bar{j}}] \\
&+ \delta(n,a)\, [+ {}^{A}t^{\bar{m}}_{\bar{j}}\, {}^{A}t^{n\bar{b}}_{m\bar{i}} - {}^{A}t^{\bar{m}}_{\bar{i}}\, {}^{A}t^{n\bar{b}}_{m\bar{j}}] \\
&+ \delta(n,b)\, [- {}^{A}t^{\bar{m}}_{\bar{j}}\, {}^{A}t^{n\bar{a}}_{m\bar{i}} + {}^{A}t^{\bar{m}}_{\bar{i}}\, {}^{A}t^{n\bar{a}}_{m\bar{j}}] \\
&+ \delta(m,j)\, [- {}^{A}t^{\bar{a}}_{\bar{n}}\, {}^{A}t^{n\bar{b}}_{m\bar{i}} + {}^{A}t^{\bar{b}}_{\bar{n}}\, {}^{A}t^{n\bar{a}}_{m\bar{i}}] \\
&+ \delta(m,i)\, [+ {}^{A}t^{\bar{a}}_{\bar{n}}\, {}^{A}t^{n\bar{b}}_{m\bar{j}} - {}^{A}t^{\bar{b}}_{\bar{n}}\, {}^{A}t^{n\bar{a}}_{m\bar{j}}] \\
&+ \delta(m,j)\, \delta(n,a)\, [- {}^{A}t^{n\bar{b}}_{m\bar{i}}] \\
&+ \delta(m,j)\, \delta(n,b)\, [+ {}^{A}t^{n\bar{a}}_{m\bar{i}}] \\
&+ \delta(m,i)\, \delta(n,a)\, [+ {}^{A}t^{n\bar{b}}_{m\bar{j}}] \\
&+ \delta(m,i)\, \delta(n,b)\, [- {}^{A}t^{n\bar{a}}_{m\bar{j}}]
\end{aligned}
\tag{S5}
$$

$$M_{ij}^{a\bar{b}} = 0 \tag{S6}$$

$$M_{ij}^{\bar{a}b} = 0 \tag{S7}$$

$$M_{ij}^{\bar{a}\bar{b}} = 0 \tag{S8}$$

$$M_{i\bar{j}}^{ab} = 0 \tag{S9}$$

$$
\begin{aligned}
M_{i\bar{j}}^{a\bar{b}} =&[- {}^{A}t^{b\bar{a}}_{j\bar{n}}\, {}^{A}t^{n\bar{m}}_{m\bar{i}} - {}^{A}t^{b\bar{a}}_{m\bar{i}}\, {}^{A}t^{n\bar{m}}_{j\bar{n}} + {}^{A}t^{b\bar{a}}_{m\bar{n}}\, {}^{A}t^{n\bar{m}}_{j\bar{i}} - {}^{A}t^{n\bar{a}}_{j\bar{i}}\, {}^{A}t^{b\bar{m}}_{m\bar{n}} + {}^{A}t^{n\bar{a}}_{j\bar{n}}\, {}^{A}t^{b\bar{m}}_{m\bar{i}} + {}^{A}t^{n\bar{a}}_{m\bar{i}}\, {}^{A}t^{b\bar{m}}_{j\bar{n}} \\
&- {}^{A}t^{n\bar{a}}_{m\bar{n}}\, {}^{A}t^{b\bar{m}}_{j\bar{i}} + {}^{A}t^{\bar{a}\bar{m}}_{\bar{n}\bar{i}}\, {}^{A}t^{bn}_{mj} + {}^{A}t^{\bar{a}}_{\bar{n}}\, {}^{A}t^{b}_{m}\, {}^{A}t^{n\bar{m}}_{j\bar{i}} + {}^{A}t^{\bar{a}}_{\bar{n}}\, {}^{A}t^{n}_{j}\, {}^{A}t^{b\bar{m}}_{m\bar{i}} + {}^{A}t^{\bar{a}}_{\bar{n}}\, {}^{A}t^{\bar{m}}_{\bar{i}}\, {}^{A}t^{bn}_{mj} \\
&+ {}^{A}t^{b}_{m}\, {}^{A}t^{n}_{j}\, {}^{A}t^{\bar{a}\bar{m}}_{\bar{n}\bar{i}} + {}^{A}t^{b}_{m}\, {}^{A}t^{\bar{m}}_{\bar{i}}\, {}^{A}t^{n\bar{a}}_{j\bar{n}} + {}^{A}t^{n}_{j}\, {}^{A}t^{\bar{m}}_{\bar{i}}\, {}^{A}t^{b\bar{a}}_{m\bar{n}} + {}^{A}t^{\bar{a}}_{\bar{n}}\, {}^{A}t^{b}_{m}\, {}^{A}t^{n}_{j}\, {}^{A}t^{\bar{m}}_{\bar{i}}] \\
&+ \delta(n,a)\, [+ {}^{A}t^{b}_{m}\, {}^{A}t^{n\bar{m}}_{j\bar{i}} + {}^{A}t^{n}_{j}\, {}^{A}t^{b\bar{m}}_{m\bar{i}} + {}^{A}t^{\bar{m}}_{\bar{i}}\, {}^{A}t^{bn}_{mj} + {}^{A}t^{b}_{m}\, {}^{A}t^{n}_{j}\, {}^{A}t^{\bar{m}}_{\bar{i}}] \\
&+ \delta(\bar{m},\bar{b})\, [+ {}^{A}t^{\bar{a}}_{\bar{n}}\, {}^{A}t^{n\bar{m}}_{j\bar{i}} + {}^{A}t^{n}_{j}\, {}^{A}t^{\bar{a}\bar{m}}_{\bar{n}\bar{i}} + {}^{A}t^{\bar{m}}_{\bar{i}}\, {}^{A}t^{n\bar{a}}_{j\bar{n}} + {}^{A}t^{\bar{a}}_{\bar{n}}\, {}^{A}t^{n}_{j}\, {}^{A}t^{\bar{m}}_{\bar{i}}] \\
&+ \delta(\bar{n},\bar{j})\, [- {}^{A}t^{\bar{a}}_{\bar{n}}\, {}^{A}t^{b\bar{m}}_{m\bar{i}} - {}^{A}t^{b}_{m}\, {}^{A}t^{\bar{a}\bar{m}}_{\bar{n}\bar{i}} - {}^{A}t^{\bar{m}}_{\bar{i}}\, {}^{A}t^{b\bar{a}}_{m\bar{n}} - {}^{A}t^{\bar{a}}_{\bar{n}}\, {}^{A}t^{b}_{m}\, {}^{A}t^{\bar{m}}_{\bar{i}}] \\
&+ \delta(m,i)\, [- {}^{A}t^{\bar{a}}_{\bar{n}}\, {}^{A}t^{bn}_{mj} - {}^{A}t^{b}_{m}\, {}^{A}t^{n\bar{a}}_{j\bar{n}} - {}^{A}t^{n}_{j}\, {}^{A}t^{b\bar{a}}_{m\bar{n}} - {}^{A}t^{\bar{a}}_{\bar{n}}\, {}^{A}t^{b}_{m}\, {}^{A}t^{n}_{j}] \\
&+ \delta(\bar{m},\bar{b})\, \delta(n,a)\, [+ {}^{A}t^{n\bar{m}}_{j\bar{i}} + {}^{A}t^{n}_{j}\, {}^{A}t^{\bar{m}}_{\bar{i}}] \\
&+ \delta(\bar{n},\bar{j})\, \delta(n,a)\, [- {}^{A}t^{b\bar{m}}_{m\bar{i}} - {}^{A}t^{b}_{m}\, {}^{A}t^{\bar{m}}_{\bar{i}}] \\
&+ \delta(\bar{n},\bar{j})\, \delta(\bar{m},\bar{b})\, [- {}^{A}t^{\bar{a}\bar{m}}_{\bar{n}\bar{i}} - {}^{A}t^{\bar{a}}_{\bar{n}}\, {}^{A}t^{\bar{m}}_{\bar{i}}] \\
&+ \delta(m,i)\, \delta(n,a)\, [- {}^{A}t^{bn}_{mj} - {}^{A}t^{b}_{m}\, {}^{A}t^{n}_{j}] \\
&+ \delta(m,i)\, \delta(\bar{m},\bar{b})\, [- {}^{A}t^{n\bar{a}}_{j\bar{n}} - {}^{A}t^{\bar{a}}_{\bar{n}}\, {}^{A}t^{n}_{j}] \\
&+ \delta(m,i)\, \delta(\bar{n},\bar{j})\, [+ {}^{A}t^{b\bar{a}}_{m\bar{n}} + {}^{A}t^{\bar{a}}_{\bar{n}}\, {}^{A}t^{b}_{m}] \\
&+ \delta(\bar{n},\bar{j})\, \delta(n,a)\, \delta(\bar{m},\bar{b})\, [- {}^{A}t^{\bar{m}}_{\bar{i}}] \\
&+ \delta(m,i)\, \delta(n,a)\, \delta(\bar{m},\bar{b})\, [- {}^{A}t^{n}_{j}] \\
&+ \delta(m,i)\, \delta(\bar{n},\bar{j})\, \delta(n,a)\, [+ {}^{A}t^{b}_{m}] \\
&+ \delta(m,i)\, \delta(\bar{n},\bar{j})\, \delta(\bar{m},\bar{b})\, [+ {}^{A}t^{\bar{a}}_{\bar{n}}]
\end{aligned}
\tag{S10}
$$

$$
\begin{aligned}
M^{\bar a b}_{i\bar j} =[&+ {}^{A}t^{a\bar b}_{j\bar n}\,{}^{A}t^{n\bar m}_{m\bar i} + {}^{A}t^{a\bar b}_{m\bar i}\,{}^{A}t^{n\bar m}_{j\bar n} - {}^{A}t^{a\bar b}_{m\bar n}\,{}^{A}t^{n\bar m}_{j\bar i} - {}^{A}t^{an}_{mj}\,{}^{A}t^{\bar b\bar m}_{\bar n\bar i} + {}^{A}t^{a\bar m}_{j\bar i}\,{}^{A}t^{n\bar b}_{m\bar n} - {}^{A}t^{a\bar m}_{j\bar n}\,{}^{A}t^{n\bar b}_{m\bar i}\\
&- {}^{A}t^{a\bar m}_{m\bar i}\,{}^{A}t^{n\bar b}_{j\bar n} + {}^{A}t^{a\bar m}_{m\bar n}\,{}^{A}t^{n\bar b}_{j\bar i} - {}^{A}t^{a}_{m}\,{}^{A}t^{\bar b}_{\bar n}\,{}^{A}t^{n\bar m}_{j\bar i} - {}^{A}t^{a}_{m}\,{}^{A}t^{n}_{j}\,{}^{A}t^{\bar b\bar m}_{\bar n\bar i} - {}^{A}t^{a}_{m}\,{}^{A}t^{\bar m}_{\bar i}\,{}^{A}t^{n\bar b}_{j\bar n}\\
&- {}^{A}t^{\bar b}_{\bar n}\,{}^{A}t^{n}_{j}\,{}^{A}t^{a\bar m}_{m\bar i} - {}^{A}t^{\bar b}_{\bar n}\,{}^{A}t^{\bar m}_{\bar i}\,{}^{A}t^{an}_{mj} - {}^{A}t^{n}_{j}\,{}^{A}t^{\bar m}_{\bar i}\,{}^{A}t^{a\bar b}_{m\bar n} - {}^{A}t^{a}_{m}\,{}^{A}t^{\bar b}_{\bar n}\,{}^{A}t^{n}_{j}\,{}^{A}t^{\bar m}_{\bar i}]\\
&+ \delta(\bar m,\bar a)\,[- {}^{A}t^{\bar b}_{\bar n}\,{}^{A}t^{n\bar m}_{j\bar i} - {}^{A}t^{n}_{j}\,{}^{A}t^{\bar b\bar m}_{\bar n\bar i} - {}^{A}t^{\bar m}_{\bar i}\,{}^{A}t^{n\bar b}_{j\bar n} - {}^{A}t^{\bar b}_{\bar n}\,{}^{A}t^{n}_{j}\,{}^{A}t^{\bar m}_{\bar i}]\\
&+ \delta(n,b)\,[- {}^{A}t^{a}_{m}\,{}^{A}t^{n\bar m}_{j\bar i} - {}^{A}t^{n}_{j}\,{}^{A}t^{a\bar m}_{m\bar i} - {}^{A}t^{\bar m}_{\bar i}\,{}^{A}t^{an}_{mj} - {}^{A}t^{a}_{m}\,{}^{A}t^{n}_{j}\,{}^{A}t^{\bar m}_{\bar i}]\\
&+ \delta(\bar n,\bar j)\,[+ {}^{A}t^{a}_{m}\,{}^{A}t^{\bar b\bar m}_{\bar n\bar i} + {}^{A}t^{\bar b}_{\bar n}\,{}^{A}t^{a\bar m}_{m\bar i} + {}^{A}t^{\bar m}_{\bar i}\,{}^{A}t^{a\bar b}_{m\bar n} + {}^{A}t^{a}_{m}\,{}^{A}t^{\bar b}_{\bar n}\,{}^{A}t^{\bar m}_{\bar i}]\\
&+ \delta(m,i)\,[+ {}^{A}t^{a}_{m}\,{}^{A}t^{n\bar b}_{j\bar n} + {}^{A}t^{\bar b}_{\bar n}\,{}^{A}t^{an}_{mj} + {}^{A}t^{n}_{j}\,{}^{A}t^{a\bar b}_{m\bar n} + {}^{A}t^{a}_{m}\,{}^{A}t^{\bar b}_{\bar n}\,{}^{A}t^{n}_{j}]\\
&+ \delta(\bar m,\bar a)\,\delta(n,b)\,[- {}^{A}t^{n\bar m}_{j\bar i} - {}^{A}t^{n}_{j}\,{}^{A}t^{\bar m}_{\bar i}]\\
&+ \delta(\bar n,\bar j)\,\delta(\bar m,\bar a)\,[+ {}^{A}t^{\bar b\bar m}_{\bar n\bar i} + {}^{A}t^{\bar b}_{\bar n}\,{}^{A}t^{\bar m}_{\bar i}]\\
&+ \delta(\bar n,\bar j)\,\delta(n,b)\,[+ {}^{A}t^{a\bar m}_{m\bar i} + {}^{A}t^{a}_{m}\,{}^{A}t^{\bar m}_{\bar i}]\\
&+ \delta(m,i)\,\delta(\bar m,\bar a)\,[+ {}^{A}t^{n\bar b}_{j\bar n} + {}^{A}t^{\bar b}_{\bar n}\,{}^{A}t^{n}_{j}]\\
&+ \delta(m,i)\,\delta(n,b)\,[+ {}^{A}t^{an}_{mj} + {}^{A}t^{a}_{m}\,{}^{A}t^{n}_{j}]\\
&+ \delta(m,i)\,\delta(\bar n,\bar j)\,[- {}^{A}t^{a\bar b}_{m\bar n} - {}^{A}t^{a}_{m}\,{}^{A}t^{\bar b}_{\bar n}]\\
&+ \delta(\bar n,\bar j)\,\delta(n,b)\,\delta(\bar m,\bar a)\,[+ {}^{A}t^{\bar m}_{\bar i}]\\
&+ \delta(m,i)\,\delta(n,b)\,\delta(\bar m,\bar a)\,[+ {}^{A}t^{n}_{j}]\\
&+ \delta(m,i)\,\delta(\bar n,\bar j)\,\delta(\bar m,\bar a)\,[- {}^{A}t^{\bar b}_{\bar n}]\\
&+ \delta(m,i)\,\delta(\bar n,\bar j)\,\delta(n,b)\,[- {}^{A}t^{a}_{m}]
\end{aligned}
\tag{S11}
$$

$$
M^{\bar a\bar b}_{i\bar j} = 0 \tag{S12}
$$

$$
M^{ab}_{\bar i j} = 0 \tag{S13}
$$

$$
\begin{aligned}
M^{a\bar b}_{\bar i j} =[&+ {}^{A}t^{b\bar a}_{m\bar j}\,{}^{A}t^{n\bar m}_{i\bar n} + {}^{A}t^{b\bar a}_{i\bar n}\,{}^{A}t^{n\bar m}_{m\bar j} - {}^{A}t^{b\bar a}_{m\bar n}\,{}^{A}t^{n\bar m}_{i\bar j} + {}^{A}t^{n\bar a}_{i\bar j}\,{}^{A}t^{b\bar m}_{m\bar n} - {}^{A}t^{n\bar a}_{m\bar j}\,{}^{A}t^{b\bar m}_{i\bar n} - {}^{A}t^{n\bar a}_{i\bar n}\,{}^{A}t^{b\bar m}_{m\bar j}\\
&+ {}^{A}t^{n\bar a}_{m\bar n}\,{}^{A}t^{b\bar m}_{i\bar j} - {}^{A}t^{\bar a\bar m}_{\bar n\bar j}\,{}^{A}t^{bn}_{mi} - {}^{A}t^{\bar a}_{\bar n}\,{}^{A}t^{b}_{m}\,{}^{A}t^{n\bar m}_{i\bar j} - {}^{A}t^{\bar a}_{\bar n}\,{}^{A}t^{n}_{i}\,{}^{A}t^{b\bar m}_{m\bar j} - {}^{A}t^{\bar a}_{\bar n}\,{}^{A}t^{\bar m}_{\bar j}\,{}^{A}t^{bn}_{mi}\\
&- {}^{A}t^{b}_{m}\,{}^{A}t^{n}_{i}\,{}^{A}t^{\bar a\bar m}_{\bar n\bar j} - {}^{A}t^{b}_{m}\,{}^{A}t^{\bar m}_{\bar j}\,{}^{A}t^{n\bar a}_{i\bar n} - {}^{A}t^{n}_{i}\,{}^{A}t^{\bar m}_{\bar j}\,{}^{A}t^{b\bar a}_{m\bar n} - {}^{A}t^{\bar a}_{\bar n}\,{}^{A}t^{b}_{m}\,{}^{A}t^{n}_{i}\,{}^{A}t^{\bar m}_{\bar j}]\\
&+ \delta(n,a)\,[- {}^{A}t^{b}_{m}\,{}^{A}t^{n\bar m}_{i\bar j} - {}^{A}t^{n}_{i}\,{}^{A}t^{b\bar m}_{m\bar j} - {}^{A}t^{\bar m}_{\bar j}\,{}^{A}t^{bn}_{mi} - {}^{A}t^{b}_{m}\,{}^{A}t^{n}_{i}\,{}^{A}t^{\bar m}_{\bar j}]\\
&+ \delta(\bar m,\bar b)\,[- {}^{A}t^{\bar a}_{\bar n}\,{}^{A}t^{n\bar m}_{i\bar j} - {}^{A}t^{n}_{i}\,{}^{A}t^{\bar a\bar m}_{\bar n\bar j} - {}^{A}t^{\bar m}_{\bar j}\,{}^{A}t^{n\bar a}_{i\bar n} - {}^{A}t^{\bar a}_{\bar n}\,{}^{A}t^{n}_{i}\,{}^{A}t^{\bar m}_{\bar j}]\\
&+ \delta(m,j)\,[+ {}^{A}t^{\bar a}_{\bar n}\,{}^{A}t^{bn}_{mi} + {}^{A}t^{b}_{m}\,{}^{A}t^{n\bar a}_{i\bar n} + {}^{A}t^{n}_{i}\,{}^{A}t^{b\bar a}_{m\bar n} + {}^{A}t^{\bar a}_{\bar n}\,{}^{A}t^{b}_{m}\,{}^{A}t^{n}_{i}]\\
&+ \delta(\bar n,\bar i)\,[+ {}^{A}t^{\bar a}_{\bar n}\,{}^{A}t^{b\bar m}_{m\bar j} + {}^{A}t^{b}_{m}\,{}^{A}t^{\bar a\bar m}_{\bar n\bar j} + {}^{A}t^{\bar m}_{\bar j}\,{}^{A}t^{b\bar a}_{m\bar n} + {}^{A}t^{\bar a}_{\bar n}\,{}^{A}t^{b}_{m}\,{}^{A}t^{\bar m}_{\bar j}]\\
&+ \delta(\bar m,\bar b)\,\delta(n,a)\,[- {}^{A}t^{n\bar m}_{i\bar j} - {}^{A}t^{n}_{i}\,{}^{A}t^{\bar m}_{\bar j}]\\
&+ \delta(m,j)\,\delta(n,a)\,[+ {}^{A}t^{bn}_{mi} + {}^{A}t^{b}_{m}\,{}^{A}t^{n}_{i}]\\
&+ \delta(m,j)\,\delta(\bar m,\bar b)\,[+ {}^{A}t^{n\bar a}_{i\bar n} + {}^{A}t^{\bar a}_{\bar n}\,{}^{A}t^{n}_{i}]\\
&+ \delta(\bar n,\bar i)\,\delta(n,a)\,[+ {}^{A}t^{b\bar m}_{m\bar j} + {}^{A}t^{b}_{m}\,{}^{A}t^{\bar m}_{\bar j}]\\
&+ \delta(\bar n,\bar i)\,\delta(\bar m,\bar b)\,[+ {}^{A}t^{\bar a\bar m}_{\bar n\bar j} + {}^{A}t^{\bar a}_{\bar n}\,{}^{A}t^{\bar m}_{\bar j}]\\
&+ \delta(m,j)\,\delta(\bar n,\bar i)\,[- {}^{A}t^{b\bar a}_{m\bar n} - {}^{A}t^{\bar a}_{\bar n}\,{}^{A}t^{b}_{m}]\\
&+ \delta(m,j)\,\delta(n,a)\,\delta(\bar m,\bar b)\,[+ {}^{A}t^{n}_{i}]\\
&+ \delta(\bar n,\bar i)\,\delta(n,a)\,\delta(\bar m,\bar b)\,[+ {}^{A}t^{\bar m}_{\bar j}]\\
&+ \delta(m,j)\,\delta(\bar n,\bar i)\,\delta(n,a)\,[- {}^{A}t^{b}_{m}]\\
&+ \delta(m,j)\,\delta(\bar n,\bar i)\,\delta(\bar m,\bar b)\,[- {}^{A}t^{\bar a}_{\bar n}]
\end{aligned}
\tag{S14}
$$

$$
\begin{aligned}
M^{\bar{a}b}_{\bar{i}j} =& [- {}^{A}t^{a\bar{b}}_{m\bar{j}}\, {}^{A}t^{n\bar{m}}_{i\bar{n}} - {}^{A}t^{a\bar{b}}_{i\bar{n}}\, {}^{A}t^{n\bar{m}}_{m\bar{j}} + {}^{A}t^{a\bar{b}}_{m\bar{n}}\, {}^{A}t^{n\bar{m}}_{i\bar{j}} + {}^{A}t^{an}_{mi}\, {}^{A}t^{\bar{b}\bar{m}}_{\bar{n}\bar{j}} - {}^{A}t^{a\bar{m}}_{i\bar{j}}\, {}^{A}t^{n\bar{b}}_{m\bar{n}} + {}^{A}t^{a\bar{m}}_{m\bar{j}}\, {}^{A}t^{n\bar{b}}_{i\bar{n}} \\
&+ {}^{A}t^{a\bar{m}}_{i\bar{n}}\, {}^{A}t^{n\bar{b}}_{m\bar{j}} - {}^{A}t^{a\bar{m}}_{m\bar{n}}\, {}^{A}t^{n\bar{b}}_{i\bar{j}} + {}^{A}t^{a}_{m}\, {}^{A}t^{\bar{b}}_{\bar{n}}\, {}^{A}t^{n\bar{m}}_{i\bar{j}} + {}^{A}t^{a}_{m}\, {}^{A}t^{n}_{i}\, {}^{A}t^{\bar{b}\bar{m}}_{\bar{n}\bar{j}} + {}^{A}t^{a}_{m}\, {}^{A}t^{\bar{m}}_{\bar{j}}\, {}^{A}t^{n\bar{b}}_{i\bar{n}} \\
&+ {}^{A}t^{\bar{b}}_{\bar{n}}\, {}^{A}t^{n}_{i}\, {}^{A}t^{a\bar{m}}_{m\bar{j}} + {}^{A}t^{\bar{b}}_{\bar{n}}\, {}^{A}t^{\bar{m}}_{\bar{j}}\, {}^{A}t^{an}_{mi} + {}^{A}t^{n}_{i}\, {}^{A}t^{\bar{m}}_{\bar{j}}\, {}^{A}t^{a\bar{b}}_{m\bar{n}} + {}^{A}t^{a}_{m}\, {}^{A}t^{\bar{b}}_{\bar{n}}\, {}^{A}t^{n}_{i}\, {}^{A}t^{\bar{m}}_{\bar{j}}] \\
&+ \delta(\bar{m},\bar{a})\, [+ {}^{A}t^{\bar{b}}_{\bar{n}}\, {}^{A}t^{n\bar{m}}_{i\bar{j}} + {}^{A}t^{n}_{i}\, {}^{A}t^{\bar{b}\bar{m}}_{\bar{n}\bar{j}} + {}^{A}t^{\bar{m}}_{\bar{j}}\, {}^{A}t^{n\bar{b}}_{i\bar{n}} + {}^{A}t^{\bar{b}}_{\bar{n}}\, {}^{A}t^{n}_{i}\, {}^{A}t^{\bar{m}}_{\bar{j}}] \\
&+ \delta(n,b)\, [+ {}^{A}t^{a}_{m}\, {}^{A}t^{n\bar{m}}_{i\bar{j}} + {}^{A}t^{n}_{i}\, {}^{A}t^{a\bar{m}}_{m\bar{j}} + {}^{A}t^{\bar{m}}_{\bar{j}}\, {}^{A}t^{an}_{mi} + {}^{A}t^{a}_{m}\, {}^{A}t^{n}_{i}\, {}^{A}t^{\bar{m}}_{\bar{j}}] \\
&+ \delta(m,j)\, [- {}^{A}t^{a}_{m}\, {}^{A}t^{n\bar{b}}_{i\bar{n}} - {}^{A}t^{\bar{b}}_{\bar{n}}\, {}^{A}t^{an}_{mi} - {}^{A}t^{n}_{i}\, {}^{A}t^{a\bar{b}}_{m\bar{n}} - {}^{A}t^{a}_{m}\, {}^{A}t^{\bar{b}}_{\bar{n}}\, {}^{A}t^{n}_{i}] \\
&+ \delta(\bar{n},\bar{i})\, [- {}^{A}t^{a}_{m}\, {}^{A}t^{\bar{b}\bar{m}}_{\bar{n}\bar{j}} - {}^{A}t^{\bar{b}}_{\bar{n}}\, {}^{A}t^{a\bar{m}}_{m\bar{j}} - {}^{A}t^{\bar{m}}_{\bar{j}}\, {}^{A}t^{a\bar{b}}_{m\bar{n}} - {}^{A}t^{a}_{m}\, {}^{A}t^{\bar{b}}_{\bar{n}}\, {}^{A}t^{\bar{m}}_{\bar{j}}] \\
&+ \delta(\bar{m},\bar{a})\, \delta(n,b)\, [+ {}^{A}t^{n\bar{m}}_{i\bar{j}} + {}^{A}t^{n}_{i}\, {}^{A}t^{\bar{m}}_{\bar{j}}] \\
&+ \delta(m,j)\, \delta(\bar{m},\bar{a})\, [- {}^{A}t^{n\bar{b}}_{i\bar{n}} - {}^{A}t^{\bar{b}}_{\bar{n}}\, {}^{A}t^{n}_{i}] \\
&+ \delta(m,j)\, \delta(n,b)\, [- {}^{A}t^{an}_{mi} - {}^{A}t^{a}_{m}\, {}^{A}t^{n}_{i}] \\
&+ \delta(\bar{n},\bar{i})\, \delta(\bar{m},\bar{a})\, [- {}^{A}t^{\bar{b}\bar{m}}_{\bar{n}\bar{j}} - {}^{A}t^{\bar{b}}_{\bar{n}}\, {}^{A}t^{\bar{m}}_{\bar{j}}] \\
&+ \delta(\bar{n},\bar{i})\, \delta(n,b)\, [- {}^{A}t^{a\bar{m}}_{m\bar{j}} - {}^{A}t^{a}_{m}\, {}^{A}t^{\bar{m}}_{\bar{j}}] \\
&+ \delta(m,j)\, \delta(\bar{n},\bar{i})\, [+ {}^{A}t^{a\bar{b}}_{m\bar{n}} + {}^{A}t^{a}_{m}\, {}^{A}t^{\bar{b}}_{\bar{n}}] \\
&+ \delta(m,j)\, \delta(n,b)\, \delta(\bar{m},\bar{a})\, [- {}^{A}t^{n}_{i}] \\
&+ \delta(\bar{n},\bar{i})\, \delta(n,b)\, \delta(\bar{m},\bar{a})\, [- {}^{A}t^{\bar{m}}_{\bar{j}}] \\
&+ \delta(m,j)\, \delta(\bar{n},\bar{i})\, \delta(\bar{m},\bar{a})\, [+ {}^{A}t^{\bar{b}}_{\bar{n}}] \\
&+ \delta(m,j)\, \delta(\bar{n},\bar{i})\, \delta(n,b)\, [+ {}^{A}t^{a}_{m}]
\end{aligned}
\tag{S15}
$$

$$M^{\bar{a}\bar{b}}_{\bar{i}j} = 0 \tag{S16}$$

$$M^{ab}_{\bar{i}\bar{j}} = 0 \tag{S17}$$

$$M^{a\bar{b}}_{\bar{i}\bar{j}} = 0 \tag{S18}$$

$$M^{\bar{a}b}_{\bar{i}\bar{j}} = 0 \tag{S19}$$

$$
\begin{aligned}
M^{\bar{a}\bar{b}}_{\bar{i}\bar{j}} =& [- {}^{A}t^{ab}_{mj}\, {}^{A}t^{n\bar{m}}_{i\bar{n}} + {}^{A}t^{ab}_{mi}\, {}^{A}t^{n\bar{m}}_{j\bar{n}} - {}^{A}t^{an}_{ij}\, {}^{A}t^{b\bar{m}}_{m\bar{n}} + {}^{A}t^{an}_{mj}\, {}^{A}t^{b\bar{m}}_{i\bar{n}} - {}^{A}t^{an}_{mi}\, {}^{A}t^{b\bar{m}}_{j\bar{n}} + {}^{A}t^{a\bar{m}}_{j\bar{n}}\, {}^{A}t^{bn}_{mi} - {}^{A}t^{a\bar{m}}_{i\bar{n}}\, {}^{A}t^{bn}_{mj} \\
&+ {}^{A}t^{a\bar{m}}_{m\bar{n}}\, {}^{A}t^{bn}_{ij} + {}^{A}t^{a}_{m}\, {}^{A}t^{n}_{j}\, {}^{A}t^{b\bar{m}}_{i\bar{n}} - {}^{A}t^{a}_{m}\, {}^{A}t^{n}_{i}\, {}^{A}t^{b\bar{m}}_{j\bar{n}} - {}^{A}t^{b}_{m}\, {}^{A}t^{n}_{j}\, {}^{A}t^{a\bar{m}}_{i\bar{n}} + {}^{A}t^{b}_{m}\, {}^{A}t^{n}_{i}\, {}^{A}t^{a\bar{m}}_{j\bar{n}}] \\
&+ \delta(\bar{m},\bar{a})\, [+ {}^{A}t^{n}_{j}\, {}^{A}t^{b\bar{m}}_{i\bar{n}} - {}^{A}t^{n}_{i}\, {}^{A}t^{b\bar{m}}_{j\bar{n}}] \\
&+ \delta(\bar{m},\bar{b})\, [- {}^{A}t^{n}_{j}\, {}^{A}t^{a\bar{m}}_{i\bar{n}} + {}^{A}t^{n}_{i}\, {}^{A}t^{a\bar{m}}_{j\bar{n}}] \\
&+ \delta(\bar{n},\bar{j})\, [- {}^{A}t^{a}_{m}\, {}^{A}t^{b\bar{m}}_{i\bar{n}} + {}^{A}t^{b}_{m}\, {}^{A}t^{a\bar{m}}_{i\bar{n}}] \\
&+ \delta(\bar{n},\bar{i})\, [+ {}^{A}t^{a}_{m}\, {}^{A}t^{b\bar{m}}_{j\bar{n}} - {}^{A}t^{b}_{m}\, {}^{A}t^{a\bar{m}}_{j\bar{n}}] \\
&+ \delta(\bar{n},\bar{j})\, \delta(\bar{m},\bar{a})\, [- {}^{A}t^{b\bar{m}}_{i\bar{n}}] \\
&+ \delta(\bar{n},\bar{j})\, \delta(\bar{m},\bar{b})\, [+ {}^{A}t^{a\bar{m}}_{i\bar{n}}] \\
&+ \delta(\bar{n},\bar{i})\, \delta(\bar{m},\bar{a})\, [+ {}^{A}t^{b\bar{m}}_{j\bar{n}}] \\
&+ \delta(\bar{n},\bar{i})\, \delta(\bar{m},\bar{b})\, [- {}^{A}t^{a\bar{m}}_{j\bar{n}}]
\end{aligned}
\tag{S20}
$$

### C. $M_{ij}^{ab}$ disconnected contributions

$$
\begin{aligned}
M_{ij}^{ab} =& [+ {}^{A}t_{i}^{a}\, {}^{A}t_{\bar{n}}^{\bar{b}}\, {}^{A}t_{m\bar{j}}^{n\bar{m}} + {}^{A}t_{i}^{a}\, {}^{A}t_{\bar{j}}^{\bar{m}}\, {}^{A}t_{m\bar{n}}^{n\bar{b}} - {}^{A}t_{j}^{a}\, {}^{A}t_{\bar{n}}^{\bar{b}}\, {}^{A}t_{m\bar{i}}^{n\bar{m}} - {}^{A}t_{j}^{a}\, {}^{A}t_{\bar{i}}^{\bar{m}}\, {}^{A}t_{m\bar{n}}^{n\bar{b}} - {}^{A}t_{i}^{b}\, {}^{A}t_{\bar{n}}^{\bar{a}}\, {}^{A}t_{m\bar{j}}^{n\bar{m}} \\
& - {}^{A}t_{i}^{b}\, {}^{A}t_{\bar{j}}^{\bar{m}}\, {}^{A}t_{m\bar{n}}^{n\bar{a}} + {}^{A}t_{j}^{b}\, {}^{A}t_{\bar{n}}^{\bar{a}}\, {}^{A}t_{m\bar{i}}^{n\bar{m}} + {}^{A}t_{j}^{b}\, {}^{A}t_{\bar{i}}^{\bar{m}}\, {}^{A}t_{m\bar{n}}^{n\bar{a}} - {}^{A}t_{\bar{i}}^{\bar{a}}\, {}^{A}t_{\bar{n}}^{\bar{b}}\, {}^{A}t_{m\bar{j}}^{n\bar{m}} - {}^{A}t_{\bar{i}}^{\bar{a}}\, {}^{A}t_{\bar{j}}^{\bar{m}}\, {}^{A}t_{m\bar{n}}^{n\bar{b}} \\
& + {}^{A}t_{\bar{j}}^{\bar{a}}\, {}^{A}t_{\bar{n}}^{\bar{b}}\, {}^{A}t_{m\bar{i}}^{n\bar{m}} + {}^{A}t_{\bar{j}}^{\bar{a}}\, {}^{A}t_{\bar{i}}^{\bar{m}}\, {}^{A}t_{m\bar{n}}^{n\bar{b}} + {}^{A}t_{\bar{i}}^{\bar{b}}\, {}^{A}t_{\bar{n}}^{\bar{a}}\, {}^{A}t_{m\bar{j}}^{n\bar{m}} + {}^{A}t_{\bar{i}}^{\bar{b}}\, {}^{A}t_{\bar{j}}^{\bar{m}}\, {}^{A}t_{m\bar{n}}^{n\bar{a}} \\
& - {}^{A}t_{\bar{j}}^{\bar{b}}\, {}^{A}t_{\bar{n}}^{\bar{a}}\, {}^{A}t_{m\bar{i}}^{n\bar{m}} - {}^{A}t_{\bar{j}}^{\bar{b}}\, {}^{A}t_{\bar{i}}^{\bar{m}}\, {}^{A}t_{m\bar{n}}^{n\bar{a}}] \\
& + \delta(n,b)\, [+ {}^{A}t_{i}^{a}\, {}^{A}t_{m\bar{j}}^{n\bar{m}} - {}^{A}t_{j}^{a}\, {}^{A}t_{m\bar{i}}^{n\bar{m}} - {}^{A}t_{i}^{n}\, {}^{A}t_{\bar{n}}^{\bar{a}}\, {}^{A}t_{m\bar{j}}^{n\bar{m}} - {}^{A}t_{i}^{n}\, {}^{A}t_{\bar{j}}^{\bar{m}}\, {}^{A}t_{m\bar{n}}^{n\bar{a}} + {}^{A}t_{j}^{n}\, {}^{A}t_{\bar{n}}^{\bar{a}}\, {}^{A}t_{m\bar{i}}^{n\bar{m}} \\
& + {}^{A}t_{j}^{n}\, {}^{A}t_{\bar{i}}^{\bar{m}}\, {}^{A}t_{m\bar{n}}^{n\bar{a}} - {}^{A}t_{\bar{i}}^{\bar{a}}\, {}^{A}t_{m\bar{j}}^{n\bar{m}} + {}^{A}t_{\bar{j}}^{\bar{a}}\, {}^{A}t_{m\bar{i}}^{n\bar{m}}] \\
& + \delta(m,j)\, [- {}^{A}t_{i}^{a}\, {}^{A}t_{m\bar{n}}^{n\bar{b}} - {}^{A}t_{m}^{a}\, {}^{A}t_{\bar{n}}^{\bar{b}}\, {}^{A}t_{m\bar{i}}^{n\bar{m}} - {}^{A}t_{m}^{a}\, {}^{A}t_{\bar{i}}^{\bar{m}}\, {}^{A}t_{m\bar{n}}^{n\bar{b}} + {}^{A}t_{i}^{b}\, {}^{A}t_{m\bar{n}}^{n\bar{a}} + {}^{A}t_{m}^{b}\, {}^{A}t_{\bar{n}}^{\bar{a}}\, {}^{A}t_{m\bar{i}}^{n\bar{m}} \\
& + {}^{A}t_{m}^{b}\, {}^{A}t_{\bar{i}}^{\bar{m}}\, {}^{A}t_{m\bar{n}}^{n\bar{a}} + {}^{A}t_{\bar{i}}^{\bar{a}}\, {}^{A}t_{m\bar{n}}^{n\bar{b}} - {}^{A}t_{\bar{i}}^{\bar{b}}\, {}^{A}t_{m\bar{n}}^{n\bar{a}}] \\
& + \delta(n,a)\, [+ {}^{A}t_{i}^{n}\, {}^{A}t_{\bar{n}}^{\bar{b}}\, {}^{A}t_{m\bar{j}}^{n\bar{m}} + {}^{A}t_{i}^{n}\, {}^{A}t_{\bar{j}}^{\bar{m}}\, {}^{A}t_{m\bar{n}}^{n\bar{b}} - {}^{A}t_{j}^{n}\, {}^{A}t_{\bar{n}}^{\bar{b}}\, {}^{A}t_{m\bar{i}}^{n\bar{m}} - {}^{A}t_{j}^{n}\, {}^{A}t_{\bar{i}}^{\bar{m}}\, {}^{A}t_{m\bar{n}}^{n\bar{b}} - {}^{A}t_{i}^{b}\, {}^{A}t_{m\bar{j}}^{n\bar{m}} \\
& + {}^{A}t_{j}^{b}\, {}^{A}t_{m\bar{i}}^{n\bar{m}} + {}^{A}t_{\bar{i}}^{\bar{b}}\, {}^{A}t_{m\bar{j}}^{n\bar{m}} - {}^{A}t_{\bar{j}}^{\bar{b}}\, {}^{A}t_{m\bar{i}}^{n\bar{m}}] \\
& + \delta(m,i)\, [+ {}^{A}t_{m}^{a}\, {}^{A}t_{\bar{n}}^{\bar{b}}\, {}^{A}t_{m\bar{j}}^{n\bar{m}} + {}^{A}t_{m}^{a}\, {}^{A}t_{\bar{j}}^{\bar{m}}\, {}^{A}t_{m\bar{n}}^{n\bar{b}} + {}^{A}t_{j}^{a}\, {}^{A}t_{m\bar{n}}^{n\bar{b}} - {}^{A}t_{m}^{b}\, {}^{A}t_{\bar{n}}^{\bar{a}}\, {}^{A}t_{m\bar{j}}^{n\bar{m}} - {}^{A}t_{m}^{b}\, {}^{A}t_{\bar{j}}^{\bar{m}}\, {}^{A}t_{m\bar{n}}^{n\bar{a}} \\
& - {}^{A}t_{j}^{b}\, {}^{A}t_{m\bar{n}}^{n\bar{a}} - {}^{A}t_{\bar{j}}^{\bar{a}}\, {}^{A}t_{m\bar{n}}^{n\bar{b}} + {}^{A}t_{\bar{j}}^{\bar{b}}\, {}^{A}t_{m\bar{n}}^{n\bar{a}}] \\
& + \delta(m,j)\, \delta(n,a)\, [- {}^{A}t_{i}^{n}\, {}^{A}t_{m\bar{n}}^{n\bar{b}} - {}^{A}t_{m}^{n}\, {}^{A}t_{\bar{n}}^{\bar{b}}\, {}^{A}t_{m\bar{i}}^{n\bar{m}} - {}^{A}t_{m}^{n}\, {}^{A}t_{\bar{i}}^{\bar{m}}\, {}^{A}t_{m\bar{n}}^{n\bar{b}} + {}^{A}t_{m}^{b}\, {}^{A}t_{m\bar{i}}^{n\bar{m}}] \\
& + \delta(m,i)\, \delta(n,b)\, [+ {}^{A}t_{m}^{a}\, {}^{A}t_{m\bar{j}}^{n\bar{m}} - {}^{A}t_{m}^{n}\, {}^{A}t_{\bar{n}}^{\bar{a}}\, {}^{A}t_{m\bar{j}}^{n\bar{m}} - {}^{A}t_{m}^{n}\, {}^{A}t_{\bar{j}}^{\bar{m}}\, {}^{A}t_{m\bar{n}}^{n\bar{a}} - {}^{A}t_{j}^{n}\, {}^{A}t_{m\bar{n}}^{n\bar{a}}] \\
& + \delta(m,i)\, \delta(n,a)\, [+ {}^{A}t_{m}^{n}\, {}^{A}t_{\bar{n}}^{\bar{b}}\, {}^{A}t_{m\bar{j}}^{n\bar{m}} + {}^{A}t_{m}^{n}\, {}^{A}t_{\bar{j}}^{\bar{m}}\, {}^{A}t_{m\bar{n}}^{n\bar{b}} + {}^{A}t_{j}^{n}\, {}^{A}t_{m\bar{n}}^{n\bar{b}} - {}^{A}t_{m}^{b}\, {}^{A}t_{m\bar{j}}^{n\bar{m}}] \\
& + \delta(m,j)\, \delta(n,b)\, [- {}^{A}t_{m}^{a}\, {}^{A}t_{m\bar{i}}^{n\bar{m}} + {}^{A}t_{i}^{n}\, {}^{A}t_{m\bar{n}}^{n\bar{a}} + {}^{A}t_{m}^{n}\, {}^{A}t_{\bar{n}}^{\bar{a}}\, {}^{A}t_{m\bar{i}}^{n\bar{m}} + {}^{A}t_{m}^{n}\, {}^{A}t_{\bar{i}}^{\bar{m}}\, {}^{A}t_{m\bar{n}}^{n\bar{a}}]
\end{aligned}
\tag{S21}
$$

$$M_{ij}^{a\bar{b}} = 0 \tag{S22}$$

$$M_{ij}^{\bar{a}b} = 0 \tag{S23}$$

$$M_{ij}^{\bar{a}\bar{b}} = 0 \tag{S24}$$

$$M_{i\bar{j}}^{ab} = 0 \tag{S25}$$

$$
\begin{aligned}
M^{a\bar{b}}_{i\bar{j}} =[&+ {}^{A}t^{a}_{i}\,{}^{A}t^{b}_{m}\,{}^{A}t^{n\bar{m}}_{j\bar{n}} + {}^{A}t^{a}_{i}\,{}^{A}t^{n}_{j}\,{}^{A}t^{b\bar{m}}_{m\bar{n}} + {}^{A}t^{\bar{b}}_{\bar{j}}\,{}^{A}t^{\bar{a}}_{\bar{n}}\,{}^{A}t^{n\bar{m}}_{m\bar{i}} + {}^{A}t^{\bar{b}}_{\bar{j}}\,{}^{A}t^{\bar{m}}_{\bar{i}}\,{}^{A}t^{n\bar{a}}_{m\bar{n}} - {}^{A}t^{\bar{a}}_{\bar{i}}\,{}^{A}t^{b}_{m}\,{}^{A}t^{n\bar{m}}_{j\bar{n}} \\
&- {}^{A}t^{\bar{a}}_{\bar{i}}\,{}^{A}t^{n}_{j}\,{}^{A}t^{b\bar{m}}_{m\bar{n}} - {}^{A}t^{b}_{j}\,{}^{A}t^{\bar{a}}_{\bar{n}}\,{}^{A}t^{n\bar{m}}_{m\bar{i}} - {}^{A}t^{b}_{j}\,{}^{A}t^{\bar{m}}_{\bar{i}}\,{}^{A}t^{n\bar{a}}_{m\bar{n}}] \\
&+ \delta(\bar{m},\bar{b})\,[+ {}^{A}t^{a}_{i}\,{}^{A}t^{n\bar{m}}_{j\bar{n}} + {}^{A}t^{\bar{m}}_{\bar{j}}\,{}^{A}t^{\bar{a}}_{\bar{n}}\,{}^{A}t^{n\bar{m}}_{m\bar{i}} + {}^{A}t^{\bar{m}}_{\bar{j}}\,{}^{A}t^{\bar{m}}_{\bar{i}}\,{}^{A}t^{n\bar{a}}_{m\bar{n}} - {}^{A}t^{\bar{a}}_{\bar{i}}\,{}^{A}t^{n\bar{m}}_{j\bar{n}}] \\
&+ \delta(\bar{n},\bar{j})\,[- {}^{A}t^{a}_{i}\,{}^{A}t^{b\bar{m}}_{m\bar{n}} + {}^{A}t^{\bar{b}}_{\bar{n}}\,{}^{A}t^{\bar{a}}_{\bar{n}}\,{}^{A}t^{n\bar{m}}_{m\bar{i}} + {}^{A}t^{\bar{b}}_{\bar{n}}\,{}^{A}t^{\bar{m}}_{\bar{i}}\,{}^{A}t^{n\bar{a}}_{m\bar{n}} + {}^{A}t^{\bar{a}}_{\bar{i}}\,{}^{A}t^{b\bar{m}}_{m\bar{n}}] \\
&+ \delta(n,a)\,[+ {}^{A}t^{n}_{i}\,{}^{A}t^{b}_{m}\,{}^{A}t^{n\bar{m}}_{j\bar{n}} + {}^{A}t^{n}_{i}\,{}^{A}t^{n}_{j}\,{}^{A}t^{b\bar{m}}_{m\bar{n}} + {}^{A}t^{\bar{b}}_{\bar{j}}\,{}^{A}t^{n\bar{m}}_{m\bar{i}} - {}^{A}t^{b}_{j}\,{}^{A}t^{n\bar{m}}_{m\bar{i}}] \\
&+ \delta(m,i)\,[+ {}^{A}t^{a}_{m}\,{}^{A}t^{b}_{m}\,{}^{A}t^{n\bar{m}}_{j\bar{n}} + {}^{A}t^{a}_{m}\,{}^{A}t^{n}_{j}\,{}^{A}t^{b\bar{m}}_{m\bar{n}} - {}^{A}t^{\bar{b}}_{\bar{j}}\,{}^{A}t^{n\bar{a}}_{m\bar{n}} + {}^{A}t^{b}_{j}\,{}^{A}t^{n\bar{a}}_{m\bar{n}}] \\
&+ \delta(\bar{m},\bar{b})\,\delta(n,a)\,[+ {}^{A}t^{n}_{i}\,{}^{A}t^{n\bar{m}}_{j\bar{n}}] \\
&+ \delta(\bar{n},\bar{j})\,\delta(n,a)\,[- {}^{A}t^{n}_{i}\,{}^{A}t^{b\bar{m}}_{m\bar{n}} + {}^{A}t^{\bar{b}}_{\bar{n}}\,{}^{A}t^{n\bar{m}}_{m\bar{i}}] \\
&+ \delta(m,i)\,\delta(\bar{m},\bar{b})\,[+ {}^{A}t^{a}_{m}\,{}^{A}t^{n\bar{m}}_{j\bar{n}} - {}^{A}t^{\bar{m}}_{\bar{j}}\,{}^{A}t^{n\bar{a}}_{m\bar{n}}] \\
&+ \delta(m,i)\,\delta(\bar{n},\bar{j})\,[- {}^{A}t^{a}_{m}\,{}^{A}t^{b\bar{m}}_{m\bar{n}}] \\
&+ \delta(m,i)\,\delta(n,a)\,[+ {}^{A}t^{n}_{m}\,{}^{A}t^{b}_{m}\,{}^{A}t^{n\bar{m}}_{j\bar{n}} + {}^{A}t^{n}_{m}\,{}^{A}t^{n}_{j}\,{}^{A}t^{b\bar{m}}_{m\bar{n}}] \\
&+ \delta(n,a)\,\delta(\bar{m},\bar{b})\,[+ {}^{A}t^{\bar{m}}_{\bar{j}}\,{}^{A}t^{n\bar{m}}_{m\bar{i}}] \\
&+ \delta(\bar{n},\bar{j})\,\delta(m,i)\,[- {}^{A}t^{\bar{b}}_{\bar{n}}\,{}^{A}t^{n\bar{a}}_{m\bar{n}}] \\
&+ \delta(\bar{n},\bar{j})\,\delta(\bar{m},\bar{b})\,[+ {}^{A}t^{\bar{m}}_{\bar{n}}\,{}^{A}t^{\bar{a}}_{\bar{n}}\,{}^{A}t^{n\bar{m}}_{m\bar{i}} + {}^{A}t^{\bar{m}}_{\bar{n}}\,{}^{A}t^{\bar{m}}_{\bar{i}}\,{}^{A}t^{n\bar{a}}_{m\bar{n}}] \\
&+ \delta(m,i)\,\delta(n,a)\,\delta(\bar{m},\bar{b})\,[+ {}^{A}t^{n}_{m}\,{}^{A}t^{n\bar{m}}_{j\bar{n}}] \\
&+ \delta(m,i)\,\delta(n,a)\,\delta(\bar{n},\bar{j})\,[- {}^{A}t^{n}_{m}\,{}^{A}t^{b\bar{m}}_{m\bar{n}}] \\
&+ \delta(\bar{n},\bar{j})\,\delta(\bar{m},\bar{b})\,\delta(n,a)\,[+ {}^{A}t^{\bar{m}}_{\bar{n}}\,{}^{A}t^{n\bar{m}}_{m\bar{i}}] \\
&+ \delta(\bar{n},\bar{j})\,\delta(\bar{m},\bar{b})\,\delta(m,i)\,[- {}^{A}t^{\bar{m}}_{\bar{n}}\,{}^{A}t^{n\bar{a}}_{m\bar{n}}]
\end{aligned}
\tag{S26}
$$

$$
\begin{aligned}
M^{\bar{a}b}_{i\bar{j}} =[&- {}^{A}t^{\bar{a}}_{\bar{j}}\,{}^{A}t^{\bar{b}}_{\bar{n}}\,{}^{A}t^{n\bar{m}}_{m\bar{i}} - {}^{A}t^{\bar{a}}_{\bar{j}}\,{}^{A}t^{\bar{m}}_{\bar{i}}\,{}^{A}t^{n\bar{b}}_{m\bar{n}} - {}^{A}t^{b}_{i}\,{}^{A}t^{a}_{m}\,{}^{A}t^{n\bar{m}}_{j\bar{n}} - {}^{A}t^{b}_{i}\,{}^{A}t^{n}_{j}\,{}^{A}t^{a\bar{m}}_{m\bar{n}} + {}^{A}t^{a}_{j}\,{}^{A}t^{\bar{b}}_{\bar{n}}\,{}^{A}t^{n\bar{m}}_{m\bar{i}} \\
&+ {}^{A}t^{a}_{j}\,{}^{A}t^{\bar{m}}_{\bar{i}}\,{}^{A}t^{n\bar{b}}_{m\bar{n}} + {}^{A}t^{\bar{b}}_{\bar{i}}\,{}^{A}t^{a}_{m}\,{}^{A}t^{n\bar{m}}_{j\bar{n}} + {}^{A}t^{\bar{b}}_{\bar{i}}\,{}^{A}t^{n}_{j}\,{}^{A}t^{a\bar{m}}_{m\bar{n}}] \\
&+ \delta(n,b)\,[- {}^{A}t^{\bar{a}}_{\bar{j}}\,{}^{A}t^{n\bar{m}}_{m\bar{i}} - {}^{A}t^{n}_{i}\,{}^{A}t^{a}_{m}\,{}^{A}t^{n\bar{m}}_{j\bar{n}} - {}^{A}t^{n}_{i}\,{}^{A}t^{n}_{j}\,{}^{A}t^{a\bar{m}}_{m\bar{n}} + {}^{A}t^{a}_{j}\,{}^{A}t^{n\bar{m}}_{m\bar{i}}] \\
&+ \delta(m,i)\,[+ {}^{A}t^{\bar{a}}_{\bar{j}}\,{}^{A}t^{n\bar{b}}_{m\bar{n}} - {}^{A}t^{b}_{m}\,{}^{A}t^{a}_{m}\,{}^{A}t^{n\bar{m}}_{j\bar{n}} - {}^{A}t^{b}_{m}\,{}^{A}t^{n}_{j}\,{}^{A}t^{a\bar{m}}_{m\bar{n}} - {}^{A}t^{a}_{j}\,{}^{A}t^{n\bar{b}}_{m\bar{n}}] \\
&+ \delta(\bar{m},\bar{a})\,[- {}^{A}t^{\bar{m}}_{\bar{j}}\,{}^{A}t^{\bar{b}}_{\bar{n}}\,{}^{A}t^{n\bar{m}}_{m\bar{i}} - {}^{A}t^{\bar{m}}_{\bar{j}}\,{}^{A}t^{\bar{m}}_{\bar{i}}\,{}^{A}t^{n\bar{b}}_{m\bar{n}} - {}^{A}t^{b}_{i}\,{}^{A}t^{n\bar{m}}_{j\bar{n}} + {}^{A}t^{\bar{b}}_{\bar{i}}\,{}^{A}t^{n\bar{m}}_{j\bar{n}}] \\
&+ \delta(\bar{n},\bar{j})\,[- {}^{A}t^{\bar{a}}_{\bar{n}}\,{}^{A}t^{\bar{b}}_{\bar{n}}\,{}^{A}t^{n\bar{m}}_{m\bar{i}} - {}^{A}t^{\bar{a}}_{\bar{n}}\,{}^{A}t^{\bar{m}}_{\bar{i}}\,{}^{A}t^{n\bar{b}}_{m\bar{n}} + {}^{A}t^{b}_{i}\,{}^{A}t^{a\bar{m}}_{m\bar{n}} - {}^{A}t^{\bar{b}}_{\bar{i}}\,{}^{A}t^{a\bar{m}}_{m\bar{n}}] \\
&+ \delta(n,b)\,\delta(\bar{m},\bar{a})\,[- {}^{A}t^{\bar{m}}_{\bar{j}}\,{}^{A}t^{n\bar{m}}_{m\bar{i}}] \\
&+ \delta(m,i)\,\delta(\bar{m},\bar{a})\,[+ {}^{A}t^{\bar{m}}_{\bar{j}}\,{}^{A}t^{n\bar{b}}_{m\bar{n}} - {}^{A}t^{b}_{m}\,{}^{A}t^{n\bar{m}}_{j\bar{n}}] \\
&+ \delta(\bar{n},\bar{j})\,\delta(n,b)\,[- {}^{A}t^{\bar{a}}_{\bar{n}}\,{}^{A}t^{n\bar{m}}_{m\bar{i}} + {}^{A}t^{n}_{i}\,{}^{A}t^{a\bar{m}}_{m\bar{n}}] \\
&+ \delta(\bar{n},\bar{j})\,\delta(m,i)\,[+ {}^{A}t^{\bar{a}}_{\bar{n}}\,{}^{A}t^{n\bar{b}}_{m\bar{n}}] \\
&+ \delta(\bar{n},\bar{j})\,\delta(\bar{m},\bar{a})\,[- {}^{A}t^{\bar{m}}_{\bar{n}}\,{}^{A}t^{\bar{b}}_{\bar{n}}\,{}^{A}t^{n\bar{m}}_{m\bar{i}} - {}^{A}t^{\bar{m}}_{\bar{n}}\,{}^{A}t^{\bar{m}}_{\bar{i}}\,{}^{A}t^{n\bar{b}}_{m\bar{n}}] \\
&+ \delta(\bar{m},\bar{a})\,\delta(n,b)\,[- {}^{A}t^{n}_{i}\,{}^{A}t^{n\bar{m}}_{j\bar{n}}] \\
&+ \delta(m,i)\,\delta(\bar{n},\bar{j})\,[+ {}^{A}t^{b}_{m}\,{}^{A}t^{a\bar{m}}_{m\bar{n}}] \\
&+ \delta(m,i)\,\delta(n,b)\,[- {}^{A}t^{n}_{m}\,{}^{A}t^{a}_{m}\,{}^{A}t^{n\bar{m}}_{j\bar{n}} - {}^{A}t^{n}_{m}\,{}^{A}t^{n}_{j}\,{}^{A}t^{a\bar{m}}_{m\bar{n}}] \\
&+ \delta(\bar{n},\bar{j})\,\delta(\bar{m},\bar{a})\,\delta(n,b)\,[- {}^{A}t^{\bar{m}}_{\bar{n}}\,{}^{A}t^{n\bar{m}}_{m\bar{i}}] \\
&+ \delta(\bar{n},\bar{j})\,\delta(\bar{m},\bar{a})\,\delta(m,i)\,[+ {}^{A}t^{\bar{m}}_{\bar{n}}\,{}^{A}t^{n\bar{b}}_{m\bar{n}}] \\
&+ \delta(m,i)\,\delta(n,b)\,\delta(\bar{m},\bar{a})\,[- {}^{A}t^{n}_{m}\,{}^{A}t^{n\bar{m}}_{j\bar{n}}] \\
&+ \delta(m,i)\,\delta(n,b)\,\delta(\bar{n},\bar{j})\,[+ {}^{A}t^{n}_{m}\,{}^{A}t^{a\bar{m}}_{m\bar{n}}]
\end{aligned}
\tag{S27}
$$

$$
M^{\bar{a}\bar{b}}_{i\bar{j}} = 0 \tag{S28}
$$

$$M^{ab}_{\bar{i}j} = 0 \tag{S29}$$

$$\begin{aligned}
M^{a\bar{b}}_{\bar{i}j} =& [- {}^{A}t^{a}_{j}\, {}^{A}t^{b}_{m}\, {}^{A}t^{n\bar{m}}_{i\bar{n}} - {}^{A}t^{a}_{j}\, {}^{A}t^{n}_{i}\, {}^{A}t^{b\bar{m}}_{m\bar{n}} - {}^{A}t^{\bar{b}}_{\bar{i}}\, {}^{A}t^{\bar{a}}_{\bar{n}}\, {}^{A}t^{n\bar{m}}_{m\bar{j}} - {}^{A}t^{\bar{b}}_{\bar{i}}\, {}^{A}t^{\bar{m}}_{\bar{j}}\, {}^{A}t^{n\bar{a}}_{m\bar{n}} + {}^{A}t^{\bar{a}}_{\bar{j}}\, {}^{A}t^{b}_{m}\, {}^{A}t^{n\bar{m}}_{i\bar{n}} \\
&+ {}^{A}t^{\bar{a}}_{\bar{j}}\, {}^{A}t^{n}_{i}\, {}^{A}t^{b\bar{m}}_{m\bar{n}} + {}^{A}t^{b}_{i}\, {}^{A}t^{\bar{a}}_{\bar{n}}\, {}^{A}t^{n\bar{m}}_{m\bar{j}} + {}^{A}t^{b}_{i}\, {}^{A}t^{\bar{m}}_{\bar{j}}\, {}^{A}t^{n\bar{a}}_{m\bar{n}}] \\
&+ \delta(\bar{m},\bar{b})\, [- {}^{A}t^{a}_{j}\, {}^{A}t^{n\bar{m}}_{i\bar{n}} - {}^{A}t^{\bar{m}}_{\bar{i}}\, {}^{A}t^{\bar{a}}_{\bar{n}}\, {}^{A}t^{n\bar{m}}_{m\bar{j}} - {}^{A}t^{\bar{m}}_{\bar{i}}\, {}^{A}t^{\bar{m}}_{\bar{j}}\, {}^{A}t^{n\bar{a}}_{m\bar{n}} + {}^{A}t^{\bar{a}}_{\bar{j}}\, {}^{A}t^{n\bar{m}}_{i\bar{n}}] \\
&+ \delta(\bar{n},\bar{i})\, [+ {}^{A}t^{a}_{j}\, {}^{A}t^{b\bar{m}}_{m\bar{n}} - {}^{A}t^{\bar{b}}_{\bar{n}}\, {}^{A}t^{\bar{a}}_{\bar{n}}\, {}^{A}t^{n\bar{m}}_{m\bar{j}} - {}^{A}t^{\bar{b}}_{\bar{n}}\, {}^{A}t^{\bar{m}}_{\bar{j}}\, {}^{A}t^{n\bar{a}}_{m\bar{n}} - {}^{A}t^{\bar{a}}_{\bar{j}}\, {}^{A}t^{b\bar{m}}_{m\bar{n}}] \\
&+ \delta(n,a)\, [- {}^{A}t^{n}_{j}\, {}^{A}t^{b}_{m}\, {}^{A}t^{n\bar{m}}_{i\bar{n}} - {}^{A}t^{n}_{j}\, {}^{A}t^{n}_{i}\, {}^{A}t^{b\bar{m}}_{m\bar{n}} - {}^{A}t^{\bar{b}}_{\bar{i}}\, {}^{A}t^{n\bar{m}}_{m\bar{j}} + {}^{A}t^{b}_{i}\, {}^{A}t^{n\bar{m}}_{m\bar{j}}] \\
&+ \delta(m,j)\, [- {}^{A}t^{a}_{m}\, {}^{A}t^{b}_{m}\, {}^{A}t^{n\bar{m}}_{i\bar{n}} - {}^{A}t^{a}_{m}\, {}^{A}t^{n}_{i}\, {}^{A}t^{b\bar{m}}_{m\bar{n}} + {}^{A}t^{\bar{b}}_{\bar{i}}\, {}^{A}t^{n\bar{a}}_{m\bar{n}} - {}^{A}t^{b}_{i}\, {}^{A}t^{n\bar{a}}_{m\bar{n}}] \\
&+ \delta(\bar{m},\bar{b})\, \delta(n,a)\, [- {}^{A}t^{n}_{j}\, {}^{A}t^{n\bar{m}}_{i\bar{n}}] \\
&+ \delta(\bar{n},\bar{i})\, \delta(n,a)\, [+ {}^{A}t^{n}_{j}\, {}^{A}t^{b\bar{m}}_{m\bar{n}} - {}^{A}t^{\bar{b}}_{\bar{n}}\, {}^{A}t^{n\bar{m}}_{m\bar{j}}] \\
&+ \delta(m,j)\, \delta(\bar{m},\bar{b})\, [- {}^{A}t^{a}_{m}\, {}^{A}t^{n\bar{m}}_{i\bar{n}} + {}^{A}t^{\bar{m}}_{\bar{i}}\, {}^{A}t^{n\bar{a}}_{m\bar{n}}] \\
&+ \delta(m,j)\, \delta(\bar{n},\bar{i})\, [+ {}^{A}t^{a}_{m}\, {}^{A}t^{b\bar{m}}_{m\bar{n}}] \\
&+ \delta(m,j)\, \delta(n,a)\, [- {}^{A}t^{n}_{m}\, {}^{A}t^{b}_{m}\, {}^{A}t^{n\bar{m}}_{i\bar{n}} - {}^{A}t^{n}_{m}\, {}^{A}t^{n}_{i}\, {}^{A}t^{b\bar{m}}_{m\bar{n}}] \\
&+ \delta(n,a)\, \delta(\bar{m},\bar{b})\, [- {}^{A}t^{\bar{m}}_{\bar{i}}\, {}^{A}t^{n\bar{m}}_{m\bar{j}}] \\
&+ \delta(\bar{n},\bar{i})\, \delta(m,j)\, [+ {}^{A}t^{\bar{b}}_{\bar{n}}\, {}^{A}t^{n\bar{a}}_{m\bar{n}}] \\
&+ \delta(\bar{n},\bar{i})\, \delta(\bar{m},\bar{b})\, [- {}^{A}t^{\bar{m}}_{\bar{n}}\, {}^{A}t^{\bar{a}}_{\bar{n}}\, {}^{A}t^{n\bar{m}}_{m\bar{j}} - {}^{A}t^{\bar{m}}_{\bar{n}}\, {}^{A}t^{\bar{m}}_{\bar{j}}\, {}^{A}t^{n\bar{a}}_{m\bar{n}}] \\
&+ \delta(m,j)\, \delta(n,a)\, \delta(\bar{m},\bar{b})\, [- {}^{A}t^{n}_{m}\, {}^{A}t^{n\bar{m}}_{i\bar{n}}] \\
&+ \delta(m,j)\, \delta(n,a)\, \delta(\bar{n},\bar{i})\, [+ {}^{A}t^{n}_{m}\, {}^{A}t^{b\bar{m}}_{m\bar{n}}] \\
&+ \delta(\bar{n},\bar{i})\, \delta(\bar{m},\bar{b})\, \delta(n,a)\, [- {}^{A}t^{\bar{m}}_{\bar{n}}\, {}^{A}t^{n\bar{m}}_{m\bar{j}}] \\
&+ \delta(\bar{n},\bar{i})\, \delta(\bar{m},\bar{b})\, \delta(m,j)\, [+ {}^{A}t^{\bar{m}}_{\bar{n}}\, {}^{A}t^{n\bar{a}}_{m\bar{n}}]
\end{aligned} \tag{S30}$$

$$\begin{aligned}
M^{\bar{a}b}_{\bar{i}j} =& [+ {}^{A}t^{\bar{a}}_{\bar{i}}\, {}^{A}t^{\bar{b}}_{\bar{n}}\, {}^{A}t^{n\bar{m}}_{m\bar{j}} + {}^{A}t^{\bar{a}}_{\bar{i}}\, {}^{A}t^{\bar{m}}_{\bar{j}}\, {}^{A}t^{n\bar{b}}_{m\bar{n}} + {}^{A}t^{b}_{j}\, {}^{A}t^{a}_{m}\, {}^{A}t^{n\bar{m}}_{i\bar{n}} + {}^{A}t^{b}_{j}\, {}^{A}t^{n}_{i}\, {}^{A}t^{a\bar{m}}_{m\bar{n}} - {}^{A}t^{a}_{i}\, {}^{A}t^{\bar{b}}_{\bar{n}}\, {}^{A}t^{n\bar{m}}_{m\bar{j}} \\
&- {}^{A}t^{a}_{i}\, {}^{A}t^{\bar{m}}_{\bar{j}}\, {}^{A}t^{n\bar{b}}_{m\bar{n}} - {}^{A}t^{\bar{b}}_{\bar{j}}\, {}^{A}t^{a}_{m}\, {}^{A}t^{n\bar{m}}_{i\bar{n}} - {}^{A}t^{\bar{b}}_{\bar{j}}\, {}^{A}t^{n}_{i}\, {}^{A}t^{a\bar{m}}_{m\bar{n}}] \\
&+ \delta(n,b)\, [+ {}^{A}t^{\bar{a}}_{\bar{i}}\, {}^{A}t^{n\bar{m}}_{m\bar{j}} + {}^{A}t^{n}_{j}\, {}^{A}t^{a}_{m}\, {}^{A}t^{n\bar{m}}_{i\bar{n}} + {}^{A}t^{n}_{j}\, {}^{A}t^{n}_{i}\, {}^{A}t^{a\bar{m}}_{m\bar{n}} - {}^{A}t^{a}_{i}\, {}^{A}t^{n\bar{m}}_{m\bar{j}}] \\
&+ \delta(m,j)\, [- {}^{A}t^{\bar{a}}_{\bar{i}}\, {}^{A}t^{n\bar{b}}_{m\bar{n}} + {}^{A}t^{b}_{m}\, {}^{A}t^{a}_{m}\, {}^{A}t^{n\bar{m}}_{i\bar{n}} + {}^{A}t^{b}_{m}\, {}^{A}t^{n}_{i}\, {}^{A}t^{a\bar{m}}_{m\bar{n}} + {}^{A}t^{a}_{i}\, {}^{A}t^{n\bar{b}}_{m\bar{n}}] \\
&+ \delta(\bar{m},\bar{a})\, [+ {}^{A}t^{\bar{m}}_{\bar{i}}\, {}^{A}t^{\bar{b}}_{\bar{n}}\, {}^{A}t^{n\bar{m}}_{m\bar{j}} + {}^{A}t^{\bar{m}}_{\bar{i}}\, {}^{A}t^{\bar{m}}_{\bar{j}}\, {}^{A}t^{n\bar{b}}_{m\bar{n}} + {}^{A}t^{b}_{j}\, {}^{A}t^{n\bar{m}}_{i\bar{n}} - {}^{A}t^{\bar{b}}_{\bar{j}}\, {}^{A}t^{n\bar{m}}_{i\bar{n}}] \\
&+ \delta(\bar{n},\bar{i})\, [+ {}^{A}t^{\bar{a}}_{\bar{n}}\, {}^{A}t^{\bar{b}}_{\bar{n}}\, {}^{A}t^{n\bar{m}}_{m\bar{j}} + {}^{A}t^{\bar{a}}_{\bar{n}}\, {}^{A}t^{\bar{m}}_{\bar{j}}\, {}^{A}t^{n\bar{b}}_{m\bar{n}} - {}^{A}t^{b}_{j}\, {}^{A}t^{a\bar{m}}_{m\bar{n}} + {}^{A}t^{\bar{b}}_{\bar{j}}\, {}^{A}t^{a\bar{m}}_{m\bar{n}}] \\
&+ \delta(n,b)\, \delta(\bar{m},\bar{a})\, [+ {}^{A}t^{\bar{m}}_{\bar{i}}\, {}^{A}t^{n\bar{m}}_{m\bar{j}}] \\
&+ \delta(m,j)\, \delta(\bar{m},\bar{a})\, [- {}^{A}t^{\bar{m}}_{\bar{i}}\, {}^{A}t^{n\bar{b}}_{m\bar{n}} + {}^{A}t^{b}_{m}\, {}^{A}t^{n\bar{m}}_{i\bar{n}}] \\
&+ \delta(\bar{n},\bar{i})\, \delta(n,b)\, [+ {}^{A}t^{\bar{a}}_{\bar{n}}\, {}^{A}t^{n\bar{m}}_{m\bar{j}} - {}^{A}t^{n}_{j}\, {}^{A}t^{a\bar{m}}_{m\bar{n}}] \\
&+ \delta(\bar{n},\bar{i})\, \delta(m,j)\, [- {}^{A}t^{\bar{a}}_{\bar{n}}\, {}^{A}t^{n\bar{b}}_{m\bar{n}}] \\
&+ \delta(\bar{n},\bar{i})\, \delta(\bar{m},\bar{a})\, [+ {}^{A}t^{\bar{m}}_{\bar{n}}\, {}^{A}t^{\bar{b}}_{\bar{n}}\, {}^{A}t^{n\bar{m}}_{m\bar{j}} + {}^{A}t^{\bar{m}}_{\bar{n}}\, {}^{A}t^{\bar{m}}_{\bar{j}}\, {}^{A}t^{n\bar{b}}_{m\bar{n}}] \\
&+ \delta(\bar{m},\bar{a})\, \delta(n,b)\, [+ {}^{A}t^{n}_{j}\, {}^{A}t^{n\bar{m}}_{i\bar{n}}] \\
&+ \delta(m,j)\, \delta(\bar{n},\bar{i})\, [- {}^{A}t^{b}_{m}\, {}^{A}t^{a\bar{m}}_{m\bar{n}}] \\
&+ \delta(m,j)\, \delta(n,b)\, [+ {}^{A}t^{n}_{m}\, {}^{A}t^{a}_{m}\, {}^{A}t^{n\bar{m}}_{i\bar{n}} + {}^{A}t^{n}_{m}\, {}^{A}t^{n}_{i}\, {}^{A}t^{a\bar{m}}_{m\bar{n}}] \\
&+ \delta(\bar{n},\bar{i})\, \delta(\bar{m},\bar{a})\, \delta(n,b)\, [+ {}^{A}t^{\bar{m}}_{\bar{n}}\, {}^{A}t^{n\bar{m}}_{m\bar{j}}] \\
&+ \delta(\bar{n},\bar{i})\, \delta(\bar{m},\bar{a})\, \delta(m,j)\, [- {}^{A}t^{\bar{m}}_{\bar{n}}\, {}^{A}t^{n\bar{b}}_{m\bar{n}}] \\
&+ \delta(m,j)\, \delta(n,b)\, \delta(\bar{m},\bar{a})\, [+ {}^{A}t^{n}_{m}\, {}^{A}t^{n\bar{m}}_{i\bar{n}}] \\
&+ \delta(m,j)\, \delta(n,b)\, \delta(\bar{n},\bar{i})\, [- {}^{A}t^{n}_{m}\, {}^{A}t^{a\bar{m}}_{m\bar{n}}]
\end{aligned} \tag{S31}$$

$$M^{\bar{a}\bar{b}}_{\bar{i}j} = 0 \tag{S32}$$

$$M^{ab}_{\bar{i}\bar{j}} = 0 \tag{S33}$$

$$M^{a\bar{b}}_{\bar{i}\bar{j}} = 0 \tag{S34}$$

$$M^{\bar{a}b}_{\bar{i}\bar{j}} = 0 \tag{S35}$$

$$\begin{aligned}
M^{\bar{a}\bar{b}}_{\bar{i}\bar{j}} =& [+ {}^{A}t^{\bar{a}}_{\bar{i}}\, {}^{A}t^{b}_{m}\, {}^{A}t^{n\bar{m}}_{j\bar{n}} + {}^{A}t^{\bar{a}}_{\bar{i}}\, {}^{A}t^{n}_{j}\, {}^{A}t^{b\bar{m}}_{m\bar{n}} - {}^{A}t^{\bar{a}}_{\bar{j}}\, {}^{A}t^{b}_{m}\, {}^{A}t^{n\bar{m}}_{i\bar{n}} - {}^{A}t^{\bar{a}}_{\bar{j}}\, {}^{A}t^{n}_{i}\, {}^{A}t^{b\bar{m}}_{m\bar{n}} - {}^{A}t^{\bar{b}}_{\bar{i}}\, {}^{A}t^{a}_{m}\, {}^{A}t^{n\bar{m}}_{j\bar{n}} \\
& - {}^{A}t^{\bar{b}}_{\bar{i}}\, {}^{A}t^{n}_{j}\, {}^{A}t^{a\bar{m}}_{m\bar{n}} + {}^{A}t^{\bar{b}}_{\bar{j}}\, {}^{A}t^{a}_{m}\, {}^{A}t^{n\bar{m}}_{i\bar{n}} + {}^{A}t^{\bar{b}}_{\bar{j}}\, {}^{A}t^{n}_{i}\, {}^{A}t^{a\bar{m}}_{m\bar{n}} - {}^{A}t^{a}_{i}\, {}^{A}t^{b}_{m}\, {}^{A}t^{n\bar{m}}_{j\bar{n}} - {}^{A}t^{a}_{i}\, {}^{A}t^{n}_{j}\, {}^{A}t^{b\bar{m}}_{m\bar{n}} \\
& + {}^{A}t^{a}_{j}\, {}^{A}t^{b}_{m}\, {}^{A}t^{n\bar{m}}_{i\bar{n}} + {}^{A}t^{a}_{j}\, {}^{A}t^{n}_{i}\, {}^{A}t^{b\bar{m}}_{m\bar{n}} + {}^{A}t^{b}_{i}\, {}^{A}t^{a}_{m}\, {}^{A}t^{n\bar{m}}_{j\bar{n}} + {}^{A}t^{b}_{i}\, {}^{A}t^{n}_{j}\, {}^{A}t^{a\bar{m}}_{m\bar{n}} - {}^{A}t^{b}_{j}\, {}^{A}t^{a}_{m}\, {}^{A}t^{n\bar{m}}_{i\bar{n}} - {}^{A}t^{b}_{j}\, {}^{A}t^{n}_{i}\, {}^{A}t^{a\bar{m}}_{m\bar{n}}] \\
& + \delta(\bar{m},\bar{b})\, [+ {}^{A}t^{\bar{a}}_{\bar{i}}\, {}^{A}t^{n\bar{m}}_{j\bar{n}} - {}^{A}t^{\bar{a}}_{\bar{j}}\, {}^{A}t^{n\bar{m}}_{i\bar{n}} - {}^{A}t^{\bar{m}}_{\bar{i}}\, {}^{A}t^{a}_{m}\, {}^{A}t^{n\bar{m}}_{j\bar{n}} - {}^{A}t^{\bar{m}}_{\bar{i}}\, {}^{A}t^{n}_{j}\, {}^{A}t^{a\bar{m}}_{m\bar{n}} + {}^{A}t^{\bar{m}}_{\bar{j}}\, {}^{A}t^{a}_{m}\, {}^{A}t^{n\bar{m}}_{i\bar{n}} \\
& + {}^{A}t^{\bar{m}}_{\bar{j}}\, {}^{A}t^{n}_{i}\, {}^{A}t^{a\bar{m}}_{m\bar{n}} - {}^{A}t^{a}_{i}\, {}^{A}t^{n\bar{m}}_{j\bar{n}} + {}^{A}t^{a}_{j}\, {}^{A}t^{n\bar{m}}_{i\bar{n}}] \\
& + \delta(\bar{n},\bar{j})\, [- {}^{A}t^{\bar{a}}_{\bar{i}}\, {}^{A}t^{b\bar{m}}_{m\bar{n}} - {}^{A}t^{\bar{a}}_{\bar{n}}\, {}^{A}t^{b}_{m}\, {}^{A}t^{n\bar{m}}_{i\bar{n}} - {}^{A}t^{\bar{a}}_{\bar{n}}\, {}^{A}t^{n}_{i}\, {}^{A}t^{b\bar{m}}_{m\bar{n}} + {}^{A}t^{\bar{b}}_{\bar{i}}\, {}^{A}t^{a\bar{m}}_{m\bar{n}} + {}^{A}t^{\bar{b}}_{\bar{n}}\, {}^{A}t^{a}_{m}\, {}^{A}t^{n\bar{m}}_{i\bar{n}} \\
& + {}^{A}t^{\bar{b}}_{\bar{n}}\, {}^{A}t^{n}_{i}\, {}^{A}t^{a\bar{m}}_{m\bar{n}} + {}^{A}t^{a}_{i}\, {}^{A}t^{b\bar{m}}_{m\bar{n}} - {}^{A}t^{b}_{i}\, {}^{A}t^{a\bar{m}}_{m\bar{n}}] \\
& + \delta(\bar{m},\bar{a})\, [+ {}^{A}t^{\bar{m}}_{\bar{i}}\, {}^{A}t^{b}_{m}\, {}^{A}t^{n\bar{m}}_{j\bar{n}} + {}^{A}t^{\bar{m}}_{\bar{i}}\, {}^{A}t^{n}_{j}\, {}^{A}t^{b\bar{m}}_{m\bar{n}} - {}^{A}t^{\bar{m}}_{\bar{j}}\, {}^{A}t^{b}_{m}\, {}^{A}t^{n\bar{m}}_{i\bar{n}} - {}^{A}t^{\bar{m}}_{\bar{j}}\, {}^{A}t^{n}_{i}\, {}^{A}t^{b\bar{m}}_{m\bar{n}} - {}^{A}t^{\bar{b}}_{\bar{i}}\, {}^{A}t^{n\bar{m}}_{j\bar{n}} \\
& + {}^{A}t^{\bar{b}}_{\bar{j}}\, {}^{A}t^{n\bar{m}}_{i\bar{n}} + {}^{A}t^{b}_{i}\, {}^{A}t^{n\bar{m}}_{j\bar{n}} - {}^{A}t^{b}_{j}\, {}^{A}t^{n\bar{m}}_{i\bar{n}}] \\
& + \delta(\bar{n},\bar{i})\, [+ {}^{A}t^{\bar{a}}_{\bar{n}}\, {}^{A}t^{b}_{m}\, {}^{A}t^{n\bar{m}}_{j\bar{n}} + {}^{A}t^{\bar{a}}_{\bar{n}}\, {}^{A}t^{n}_{j}\, {}^{A}t^{b\bar{m}}_{m\bar{n}} + {}^{A}t^{\bar{a}}_{\bar{j}}\, {}^{A}t^{b\bar{m}}_{m\bar{n}} - {}^{A}t^{\bar{b}}_{\bar{n}}\, {}^{A}t^{a}_{m}\, {}^{A}t^{n\bar{m}}_{j\bar{n}} - {}^{A}t^{\bar{b}}_{\bar{n}}\, {}^{A}t^{n}_{j}\, {}^{A}t^{a\bar{m}}_{m\bar{n}} \\
& - {}^{A}t^{\bar{b}}_{\bar{j}}\, {}^{A}t^{a\bar{m}}_{m\bar{n}} - {}^{A}t^{a}_{j}\, {}^{A}t^{b\bar{m}}_{m\bar{n}} + {}^{A}t^{b}_{j}\, {}^{A}t^{a\bar{m}}_{m\bar{n}}] \\
& + \delta(\bar{n},\bar{j})\, \delta(\bar{m},\bar{a})\, [- {}^{A}t^{\bar{m}}_{\bar{i}}\, {}^{A}t^{b\bar{m}}_{m\bar{n}} - {}^{A}t^{\bar{m}}_{\bar{n}}\, {}^{A}t^{b}_{m}\, {}^{A}t^{n\bar{m}}_{i\bar{n}} - {}^{A}t^{\bar{m}}_{\bar{n}}\, {}^{A}t^{n}_{i}\, {}^{A}t^{b\bar{m}}_{m\bar{n}} + {}^{A}t^{\bar{b}}_{\bar{n}}\, {}^{A}t^{n\bar{m}}_{i\bar{n}}] \\
& + \delta(\bar{n},\bar{i})\, \delta(\bar{m},\bar{b})\, [+ {}^{A}t^{\bar{a}}_{\bar{n}}\, {}^{A}t^{n\bar{m}}_{j\bar{n}} - {}^{A}t^{\bar{m}}_{\bar{n}}\, {}^{A}t^{a}_{m}\, {}^{A}t^{n\bar{m}}_{j\bar{n}} - {}^{A}t^{\bar{m}}_{\bar{n}}\, {}^{A}t^{n}_{j}\, {}^{A}t^{a\bar{m}}_{m\bar{n}} - {}^{A}t^{\bar{m}}_{\bar{j}}\, {}^{A}t^{a\bar{m}}_{m\bar{n}}] \\
& + \delta(\bar{n},\bar{i})\, \delta(\bar{m},\bar{a})\, [+ {}^{A}t^{\bar{m}}_{\bar{n}}\, {}^{A}t^{b}_{m}\, {}^{A}t^{n\bar{m}}_{j\bar{n}} + {}^{A}t^{\bar{m}}_{\bar{n}}\, {}^{A}t^{n}_{j}\, {}^{A}t^{b\bar{m}}_{m\bar{n}} + {}^{A}t^{\bar{m}}_{\bar{j}}\, {}^{A}t^{b\bar{m}}_{m\bar{n}} - {}^{A}t^{\bar{b}}_{\bar{n}}\, {}^{A}t^{n\bar{m}}_{j\bar{n}}] \\
& + \delta(\bar{n},\bar{j})\, \delta(\bar{m},\bar{b})\, [- {}^{A}t^{\bar{a}}_{\bar{n}}\, {}^{A}t^{n\bar{m}}_{i\bar{n}} + {}^{A}t^{\bar{m}}_{\bar{i}}\, {}^{A}t^{a\bar{m}}_{m\bar{n}} + {}^{A}t^{\bar{m}}_{\bar{n}}\, {}^{A}t^{a}_{m}\, {}^{A}t^{n\bar{m}}_{i\bar{n}} + {}^{A}t^{\bar{m}}_{\bar{n}}\, {}^{A}t^{n}_{i}\, {}^{A}t^{a\bar{m}}_{m\bar{n}}]
\end{aligned} \tag{S36}$$

## S3. TD-CCSD WITH ACTIVE ORBITALS OF SAME SPATIAL SYMMETRY

### A. $M_i^a$ contributions

$$\begin{aligned} M_i^a =& [- {}^A t_{\bar{n}}^{\bar{a}} \, {}^A t_{m\bar{i}}^{n\bar{m}} - {}^A t_m^n \, {}^A t_{\bar{n}\bar{i}}^{\bar{a}\bar{m}} - {}^A t_{\bar{i}}^{\bar{m}} \, {}^A t_{m\bar{n}}^{n\bar{a}} + {}^A t_{\bar{n}}^{\bar{m}} \, {}^A t_{m\bar{i}}^{n\bar{a}} - {}^A t_{\bar{n}}^{\bar{a}} \, {}^A t_m^n \, {}^A t_{\bar{i}}^{\bar{m}}] \\ & + \delta(n,a) \, [- {}^A t_{m\bar{i}}^{n\bar{m}} - {}^A t_m^n \, {}^A t_{\bar{i}}^{\bar{m}}] \\ & + \delta(m,i) \, [+ {}^A t_{m\bar{n}}^{n\bar{a}} + {}^A t_{\bar{n}}^{\bar{a}} \, {}^A t_m^n] \\ & + \delta(m,i) \, \delta(n,a) \, [+ {}^A t_m^n] \end{aligned} \tag{S37}$$

$$M_i^{\bar{a}} = 0 \tag{S38}$$

$$M_{\bar{i}}^a = 0 \tag{S39}$$

$$\begin{aligned} M_{\bar{i}}^{\bar{a}} =& [- {}^A t_m^a \, {}^A t_{i\bar{n}}^{n\bar{m}} - {}^A t_i^n \, {}^A t_{m\bar{n}}^{a\bar{m}} + {}^A t_m^n \, {}^A t_{i\bar{n}}^{a\bar{m}} - {}^A t_{\bar{n}}^{\bar{m}} \, {}^A t_{mi}^{an} - {}^A t_m^a \, {}^A t_i^n \, {}^A t_{\bar{n}}^{\bar{m}}] \\ & + \delta(\bar{m},\bar{a}) \, [- {}^A t_{i\bar{n}}^{n\bar{m}} - {}^A t_i^n \, {}^A t_{\bar{n}}^{\bar{m}}] \\ & + \delta(\bar{n},\bar{i}) \, [+ {}^A t_{m\bar{n}}^{a\bar{m}} + {}^A t_m^a \, {}^A t_{\bar{n}}^{\bar{m}}] \\ & + \delta(\bar{n},\bar{i}) \, \delta(\bar{m},\bar{a}) \, [+ {}^A t_{\bar{n}}^{\bar{m}}] \end{aligned} \tag{S40}$$

### B. $M^{ab}_{ij}$ connected contributions

$$
\begin{aligned}
M^{ab}_{ij} =[&- {}^{A}t^{\bar a\bar b}_{\bar n\bar j}\,{}^{A}t^{n\bar m}_{m\bar i} + {}^{A}t^{\bar a\bar b}_{\bar n\bar i}\,{}^{A}t^{n\bar m}_{m\bar j} + {}^{A}t^{n\bar a}_{m\bar j}\,{}^{A}t^{\bar b\bar m}_{\bar n\bar i} - {}^{A}t^{n\bar a}_{m\bar i}\,{}^{A}t^{\bar b\bar m}_{\bar n\bar j} + {}^{A}t^{n\bar a}_{m\bar n}\,{}^{A}t^{\bar b\bar m}_{\bar i\bar j}\\
&- {}^{A}t^{\bar a\bar m}_{\bar i\bar j}\,{}^{A}t^{n\bar b}_{m\bar n} + {}^{A}t^{\bar a\bar m}_{\bar n\bar j}\,{}^{A}t^{n\bar b}_{m\bar i} - {}^{A}t^{\bar a\bar m}_{\bar n\bar i}\,{}^{A}t^{n\bar b}_{m\bar j} + {}^{A}t^{\bar a}_{\bar n}\,{}^{A}t^{n}_{m}\,{}^{A}t^{\bar b\bar m}_{\bar i\bar j} + {}^{A}t^{\bar a}_{\bar n}\,{}^{A}t^{\bar m}_{\bar j}\,{}^{A}t^{n\bar b}_{m\bar i}\\
&- {}^{A}t^{\bar a}_{\bar n}\,{}^{A}t^{\bar m}_{\bar i}\,{}^{A}t^{n\bar b}_{m\bar j} - {}^{A}t^{\bar b}_{\bar n}\,{}^{A}t^{n}_{m}\,{}^{A}t^{\bar a\bar m}_{\bar i\bar j} - {}^{A}t^{\bar b}_{\bar n}\,{}^{A}t^{\bar m}_{\bar j}\,{}^{A}t^{n\bar a}_{m\bar i} + {}^{A}t^{\bar b}_{\bar n}\,{}^{A}t^{\bar m}_{\bar i}\,{}^{A}t^{n\bar a}_{m\bar j}\\
&+ {}^{A}t^{n}_{m}\,{}^{A}t^{\bar m}_{\bar j}\,{}^{A}t^{\bar a\bar b}_{\bar n\bar i} - {}^{A}t^{n}_{m}\,{}^{A}t^{\bar m}_{\bar i}\,{}^{A}t^{\bar a\bar b}_{\bar n\bar j}]\\
&+ \delta(n,a)\,[+ {}^{A}t^{n}_{m}\,{}^{A}t^{\bar b\bar m}_{\bar i\bar j} + {}^{A}t^{\bar m}_{\bar j}\,{}^{A}t^{n\bar b}_{m\bar i} - {}^{A}t^{\bar m}_{\bar i}\,{}^{A}t^{n\bar b}_{m\bar j}]\\
&+ \delta(n,b)\,[- {}^{A}t^{n}_{m}\,{}^{A}t^{\bar a\bar m}_{\bar i\bar j} - {}^{A}t^{\bar m}_{\bar j}\,{}^{A}t^{n\bar a}_{m\bar i} + {}^{A}t^{\bar m}_{\bar i}\,{}^{A}t^{n\bar a}_{m\bar j}]\\
&+ \delta(m,j)\,[- {}^{A}t^{\bar a}_{\bar n}\,{}^{A}t^{n\bar b}_{m\bar i} + {}^{A}t^{\bar b}_{\bar n}\,{}^{A}t^{n\bar a}_{m\bar i} - {}^{A}t^{n}_{m}\,{}^{A}t^{\bar a\bar b}_{\bar n\bar i}]\\
&+ \delta(m,i)\,[+ {}^{A}t^{\bar a}_{\bar n}\,{}^{A}t^{n\bar b}_{m\bar j} - {}^{A}t^{\bar b}_{\bar n}\,{}^{A}t^{n\bar a}_{m\bar j} + {}^{A}t^{n}_{m}\,{}^{A}t^{\bar a\bar b}_{\bar n\bar j}]\\
&+ \delta(m,j)\,\delta(n,a)\,[- {}^{A}t^{n\bar b}_{m\bar i}]\\
&+ \delta(m,j)\,\delta(n,b)\,[+ {}^{A}t^{n\bar a}_{m\bar i}]\\
&+ \delta(m,i)\,\delta(n,a)\,[+ {}^{A}t^{n\bar b}_{m\bar j}]\\
&+ \delta(m,i)\,\delta(n,b)\,[- {}^{A}t^{n\bar a}_{m\bar j}]
\end{aligned}
\tag{S41}
$$

$$M^{a\bar b}_{ij} = 0 \tag{S42}$$

$$M^{\bar a b}_{ij} = 0 \tag{S43}$$

$$M^{\bar a\bar b}_{ij} = 0 \tag{S44}$$

$$M^{ab}_{i\bar j} = 0 \tag{S45}$$

$$
\begin{aligned}
M^{a\bar b}_{i\bar j} =[&- {}^{A}t^{b\bar a}_{j\bar n}\,{}^{A}t^{n\bar m}_{m\bar i} - {}^{A}t^{b\bar a}_{m\bar i}\,{}^{A}t^{n\bar m}_{j\bar n} + {}^{A}t^{b\bar a}_{m\bar n}\,{}^{A}t^{n\bar m}_{j\bar i} - {}^{A}t^{n\bar a}_{j\bar i}\,{}^{A}t^{b\bar m}_{m\bar n} + {}^{A}t^{n\bar a}_{j\bar n}\,{}^{A}t^{b\bar m}_{m\bar i} + {}^{A}t^{n\bar a}_{m\bar i}\,{}^{A}t^{b\bar m}_{j\bar n}\\
&- {}^{A}t^{n\bar a}_{m\bar n}\,{}^{A}t^{b\bar m}_{j\bar i} + {}^{A}t^{\bar a\bar m}_{\bar n\bar i}\,{}^{A}t^{bn}_{mj} + {}^{A}t^{\bar a}_{\bar n}\,{}^{A}t^{b}_{m}\,{}^{A}t^{n\bar m}_{j\bar i} + {}^{A}t^{\bar a}_{\bar n}\,{}^{A}t^{n}_{j}\,{}^{A}t^{b\bar m}_{m\bar i} - {}^{A}t^{\bar a}_{\bar n}\,{}^{A}t^{n}_{m}\,{}^{A}t^{b\bar m}_{j\bar i}\\
&+ {}^{A}t^{\bar a}_{\bar n}\,{}^{A}t^{\bar m}_{\bar i}\,{}^{A}t^{bn}_{mj} + {}^{A}t^{b}_{m}\,{}^{A}t^{n}_{j}\,{}^{A}t^{\bar a\bar m}_{\bar n\bar i} + {}^{A}t^{b}_{m}\,{}^{A}t^{\bar m}_{\bar i}\,{}^{A}t^{n\bar a}_{j\bar n} - {}^{A}t^{b}_{m}\,{}^{A}t^{\bar m}_{\bar n}\,{}^{A}t^{n\bar a}_{j\bar i} + {}^{A}t^{n}_{j}\,{}^{A}t^{\bar m}_{\bar i}\,{}^{A}t^{b\bar a}_{m\bar n}\\
&- {}^{A}t^{n}_{j}\,{}^{A}t^{\bar m}_{\bar n}\,{}^{A}t^{b\bar a}_{m\bar i} - {}^{A}t^{n}_{m}\,{}^{A}t^{\bar m}_{\bar i}\,{}^{A}t^{b\bar a}_{j\bar n} + {}^{A}t^{\bar a}_{\bar n}\,{}^{A}t^{b}_{m}\,{}^{A}t^{n}_{j}\,{}^{A}t^{\bar m}_{\bar i}]\\
&+ \delta(n,a)\,[+ {}^{A}t^{b}_{m}\,{}^{A}t^{n\bar m}_{j\bar i} + {}^{A}t^{n}_{j}\,{}^{A}t^{b\bar m}_{m\bar i} - {}^{A}t^{n}_{m}\,{}^{A}t^{b\bar m}_{j\bar i} + {}^{A}t^{\bar m}_{\bar i}\,{}^{A}t^{bn}_{mj} + {}^{A}t^{b}_{m}\,{}^{A}t^{n}_{j}\,{}^{A}t^{\bar m}_{\bar i}]\\
&+ \delta(\bar m,\bar b)\,[+ {}^{A}t^{\bar a}_{\bar n}\,{}^{A}t^{n\bar m}_{j\bar i} + {}^{A}t^{n}_{j}\,{}^{A}t^{\bar a\bar m}_{\bar n\bar i} + {}^{A}t^{\bar m}_{\bar i}\,{}^{A}t^{n\bar a}_{j\bar n} - {}^{A}t^{\bar m}_{\bar n}\,{}^{A}t^{n\bar a}_{j\bar i} + {}^{A}t^{\bar a}_{\bar n}\,{}^{A}t^{n}_{j}\,{}^{A}t^{\bar m}_{\bar i}]\\
&+ \delta(\bar n,\bar j)\,[- {}^{A}t^{\bar a}_{\bar n}\,{}^{A}t^{b\bar m}_{m\bar i} - {}^{A}t^{b}_{m}\,{}^{A}t^{\bar a\bar m}_{\bar n\bar i} - {}^{A}t^{\bar m}_{\bar i}\,{}^{A}t^{b\bar a}_{m\bar n} + {}^{A}t^{\bar m}_{\bar n}\,{}^{A}t^{b\bar a}_{m\bar i} - {}^{A}t^{\bar a}_{\bar n}\,{}^{A}t^{b}_{m}\,{}^{A}t^{\bar m}_{\bar i}]\\
&+ \delta(m,i)\,[- {}^{A}t^{\bar a}_{\bar n}\,{}^{A}t^{bn}_{mj} - {}^{A}t^{b}_{m}\,{}^{A}t^{n\bar a}_{j\bar n} - {}^{A}t^{n}_{j}\,{}^{A}t^{b\bar a}_{m\bar n} + {}^{A}t^{n}_{m}\,{}^{A}t^{b\bar a}_{j\bar n} - {}^{A}t^{\bar a}_{\bar n}\,{}^{A}t^{b}_{m}\,{}^{A}t^{n}_{j}]\\
&+ \delta(\bar m,\bar b)\,\delta(n,a)\,[+ {}^{A}t^{n\bar m}_{j\bar i} + {}^{A}t^{n}_{j}\,{}^{A}t^{\bar m}_{\bar i}]\\
&+ \delta(\bar n,\bar j)\,\delta(n,a)\,[- {}^{A}t^{b\bar m}_{m\bar i} - {}^{A}t^{b}_{m}\,{}^{A}t^{\bar m}_{\bar i}]\\
&+ \delta(\bar n,\bar j)\,\delta(\bar m,\bar b)\,[- {}^{A}t^{\bar a\bar m}_{\bar n\bar i} - {}^{A}t^{\bar a}_{\bar n}\,{}^{A}t^{\bar m}_{\bar i}]\\
&+ \delta(m,i)\,\delta(n,a)\,[- {}^{A}t^{bn}_{mj} - {}^{A}t^{b}_{m}\,{}^{A}t^{n}_{j}]\\
&+ \delta(m,i)\,\delta(\bar m,\bar b)\,[- {}^{A}t^{n\bar a}_{j\bar n} - {}^{A}t^{\bar a}_{\bar n}\,{}^{A}t^{n}_{j}]\\
&+ \delta(m,i)\,\delta(\bar n,\bar j)\,[+ {}^{A}t^{b\bar a}_{m\bar n} + {}^{A}t^{\bar a}_{\bar n}\,{}^{A}t^{b}_{m}]\\
&+ \delta(\bar n,\bar j)\,\delta(n,a)\,\delta(\bar m,\bar b)\,[- {}^{A}t^{\bar m}_{\bar i}]\\
&+ \delta(m,i)\,\delta(n,a)\,\delta(\bar m,\bar b)\,[- {}^{A}t^{n}_{j}]\\
&+ \delta(m,i)\,\delta(\bar n,\bar j)\,\delta(n,a)\,[+ {}^{A}t^{b}_{m}]\\
&+ \delta(m,i)\,\delta(\bar n,\bar j)\,\delta(\bar m,\bar b)\,[+ {}^{A}t^{\bar a}_{\bar n}]
\end{aligned}
\tag{S46}
$$

$$
\begin{aligned}
M^{\bar{a}b}_{i\bar{j}} =\big[&+ {}^{A}t^{a\bar{b}}_{j\bar{n}}\,{}^{A}t^{n\bar{m}}_{m\bar{i}} + {}^{A}t^{a\bar{b}}_{m\bar{i}}\,{}^{A}t^{n\bar{m}}_{j\bar{n}} - {}^{A}t^{a\bar{b}}_{m\bar{n}}\,{}^{A}t^{n\bar{m}}_{j\bar{i}} - {}^{A}t^{an}_{mj}\,{}^{A}t^{\bar{b}\bar{m}}_{\bar{n}\bar{i}} + {}^{A}t^{a\bar{m}}_{j\bar{i}}\,{}^{A}t^{n\bar{b}}_{m\bar{n}} - {}^{A}t^{a\bar{m}}_{j\bar{n}}\,{}^{A}t^{n\bar{b}}_{m\bar{i}} \\
&- {}^{A}t^{a\bar{m}}_{m\bar{i}}\,{}^{A}t^{n\bar{b}}_{j\bar{n}} + {}^{A}t^{a\bar{m}}_{m\bar{n}}\,{}^{A}t^{n\bar{b}}_{j\bar{i}} - {}^{A}t^{a}_{m}\,{}^{A}t^{\bar{b}}_{\bar{n}}\,{}^{A}t^{n\bar{m}}_{j\bar{i}} - {}^{A}t^{a}_{m}\,{}^{A}t^{n}_{j}\,{}^{A}t^{\bar{b}\bar{m}}_{\bar{n}\bar{i}} - {}^{A}t^{a}_{m}\,{}^{A}t^{\bar{m}}_{\bar{i}}\,{}^{A}t^{n\bar{b}}_{j\bar{n}} \\
&+ {}^{A}t^{a}_{m}\,{}^{A}t^{\bar{m}}_{\bar{n}}\,{}^{A}t^{n\bar{b}}_{j\bar{i}} - {}^{A}t^{\bar{b}}_{\bar{n}}\,{}^{A}t^{n}_{j}\,{}^{A}t^{a\bar{m}}_{m\bar{i}} + {}^{A}t^{\bar{b}}_{\bar{n}}\,{}^{A}t^{n}_{m}\,{}^{A}t^{a\bar{m}}_{j\bar{i}} - {}^{A}t^{\bar{b}}_{\bar{n}}\,{}^{A}t^{\bar{m}}_{\bar{i}}\,{}^{A}t^{an}_{mj} - {}^{A}t^{n}_{j}\,{}^{A}t^{\bar{m}}_{\bar{i}}\,{}^{A}t^{a\bar{b}}_{m\bar{n}} \\
&+ {}^{A}t^{n}_{j}\,{}^{A}t^{\bar{m}}_{\bar{n}}\,{}^{A}t^{a\bar{b}}_{m\bar{i}} + {}^{A}t^{n}_{m}\,{}^{A}t^{\bar{m}}_{\bar{i}}\,{}^{A}t^{a\bar{b}}_{j\bar{n}} - {}^{A}t^{a}_{m}\,{}^{A}t^{\bar{b}}_{\bar{n}}\,{}^{A}t^{n}_{j}\,{}^{A}t^{\bar{m}}_{\bar{i}}\big] \\
&+ \delta(\bar{m},\bar{a})\,\big[- {}^{A}t^{\bar{b}}_{\bar{n}}\,{}^{A}t^{n\bar{m}}_{j\bar{i}} - {}^{A}t^{n}_{j}\,{}^{A}t^{\bar{b}\bar{m}}_{\bar{n}\bar{i}} - {}^{A}t^{\bar{m}}_{\bar{i}}\,{}^{A}t^{n\bar{b}}_{j\bar{n}} + {}^{A}t^{\bar{m}}_{\bar{n}}\,{}^{A}t^{n\bar{b}}_{j\bar{i}} - {}^{A}t^{\bar{b}}_{\bar{n}}\,{}^{A}t^{n}_{j}\,{}^{A}t^{\bar{m}}_{\bar{i}}\big] \\
&+ \delta(n,b)\,\big[- {}^{A}t^{a}_{m}\,{}^{A}t^{n\bar{m}}_{j\bar{i}} - {}^{A}t^{n}_{j}\,{}^{A}t^{a\bar{m}}_{m\bar{i}} + {}^{A}t^{n}_{m}\,{}^{A}t^{a\bar{m}}_{j\bar{i}} - {}^{A}t^{\bar{m}}_{\bar{i}}\,{}^{A}t^{an}_{mj} - {}^{A}t^{a}_{m}\,{}^{A}t^{n}_{j}\,{}^{A}t^{\bar{m}}_{\bar{i}}\big] \\
&+ \delta(\bar{n},\bar{j})\,\big[+ {}^{A}t^{a}_{m}\,{}^{A}t^{\bar{b}\bar{m}}_{\bar{n}\bar{i}} + {}^{A}t^{\bar{b}}_{\bar{n}}\,{}^{A}t^{a\bar{m}}_{m\bar{i}} + {}^{A}t^{\bar{m}}_{\bar{i}}\,{}^{A}t^{a\bar{b}}_{m\bar{n}} - {}^{A}t^{\bar{m}}_{\bar{n}}\,{}^{A}t^{a\bar{b}}_{m\bar{i}} + {}^{A}t^{a}_{m}\,{}^{A}t^{\bar{b}}_{\bar{n}}\,{}^{A}t^{\bar{m}}_{\bar{i}}\big] \\
&+ \delta(m,i)\,\big[+ {}^{A}t^{a}_{m}\,{}^{A}t^{n\bar{b}}_{j\bar{n}} + {}^{A}t^{\bar{b}}_{\bar{n}}\,{}^{A}t^{an}_{mj} + {}^{A}t^{n}_{j}\,{}^{A}t^{a\bar{b}}_{m\bar{n}} - {}^{A}t^{n}_{m}\,{}^{A}t^{a\bar{b}}_{j\bar{n}} + {}^{A}t^{a}_{m}\,{}^{A}t^{\bar{b}}_{\bar{n}}\,{}^{A}t^{n}_{j}\big] \\
&+ \delta(\bar{m},\bar{a})\,\delta(n,b)\,\big[- {}^{A}t^{n\bar{m}}_{j\bar{i}} - {}^{A}t^{n}_{j}\,{}^{A}t^{\bar{m}}_{\bar{i}}\big] \\
&+ \delta(\bar{n},\bar{j})\,\delta(\bar{m},\bar{a})\,\big[+ {}^{A}t^{\bar{b}\bar{m}}_{\bar{n}\bar{i}} + {}^{A}t^{\bar{b}}_{\bar{n}}\,{}^{A}t^{\bar{m}}_{\bar{i}}\big] \\
&+ \delta(\bar{n},\bar{j})\,\delta(n,b)\,\big[+ {}^{A}t^{a\bar{m}}_{m\bar{i}} + {}^{A}t^{a}_{m}\,{}^{A}t^{\bar{m}}_{\bar{i}}\big] \\
&+ \delta(m,i)\,\delta(\bar{m},\bar{a})\,\big[+ {}^{A}t^{n\bar{b}}_{j\bar{n}} + {}^{A}t^{\bar{b}}_{\bar{n}}\,{}^{A}t^{n}_{j}\big] \\
&+ \delta(m,i)\,\delta(n,b)\,\big[+ {}^{A}t^{an}_{mj} + {}^{A}t^{a}_{m}\,{}^{A}t^{n}_{j}\big] \\
&+ \delta(m,i)\,\delta(\bar{n},\bar{j})\,\big[- {}^{A}t^{a\bar{b}}_{m\bar{n}} - {}^{A}t^{a}_{m}\,{}^{A}t^{\bar{b}}_{\bar{n}}\big] \\
&+ \delta(\bar{n},\bar{j})\,\delta(n,b)\,\delta(\bar{m},\bar{a})\,\big[+ {}^{A}t^{\bar{m}}_{\bar{i}}\big] \\
&+ \delta(m,i)\,\delta(n,b)\,\delta(\bar{m},\bar{a})\,\big[+ {}^{A}t^{n}_{j}\big] \\
&+ \delta(m,i)\,\delta(\bar{n},\bar{j})\,\delta(\bar{m},\bar{a})\,\big[- {}^{A}t^{\bar{b}}_{\bar{n}}\big] \\
&+ \delta(m,i)\,\delta(\bar{n},\bar{j})\,\delta(n,b)\,\big[- {}^{A}t^{a}_{m}\big]
\end{aligned}
\tag{S47}
$$

$$
M^{\bar{a}\bar{b}}_{i\bar{j}} = 0 \tag{S48}
$$

$$
M^{ab}_{\bar{i}j} = 0 \tag{S49}
$$

$$
\begin{aligned}
M^{a\bar b}_{\bar i j} =&[+ {}^{A}t^{b\bar a}_{m\bar j}\,{}^{A}t^{n\bar m}_{i\bar n} + {}^{A}t^{b\bar a}_{i\bar n}\,{}^{A}t^{n\bar m}_{m\bar j} - {}^{A}t^{b\bar a}_{m\bar n}\,{}^{A}t^{n\bar m}_{i\bar j} + {}^{A}t^{n\bar a}_{i\bar j}\,{}^{A}t^{b\bar m}_{m\bar n} - {}^{A}t^{n\bar a}_{m\bar j}\,{}^{A}t^{b\bar m}_{i\bar n} - {}^{A}t^{n\bar a}_{i\bar n}\,{}^{A}t^{b\bar m}_{m\bar j}\\
&+ {}^{A}t^{n\bar a}_{m\bar n}\,{}^{A}t^{b\bar m}_{i\bar j} - {}^{A}t^{\bar a\bar m}_{\bar n\bar j}\,{}^{A}t^{bn}_{mi} - {}^{A}t^{\bar a}_{\bar n}\,{}^{A}t^{b}_{m}\,{}^{A}t^{n\bar m}_{i\bar j} - {}^{A}t^{\bar a}_{\bar n}\,{}^{A}t^{n}_{i}\,{}^{A}t^{b\bar m}_{m\bar j} + {}^{A}t^{\bar a}_{\bar n}\,{}^{A}t^{n}_{m}\,{}^{A}t^{b\bar m}_{i\bar j}\\
&- {}^{A}t^{\bar a}_{\bar n}\,{}^{A}t^{\bar m}_{\bar j}\,{}^{A}t^{bn}_{mi} - {}^{A}t^{b}_{m}\,{}^{A}t^{n}_{i}\,{}^{A}t^{\bar a\bar m}_{\bar n\bar j} - {}^{A}t^{b}_{m}\,{}^{A}t^{\bar m}_{\bar j}\,{}^{A}t^{n\bar a}_{i\bar n} + {}^{A}t^{b}_{m}\,{}^{A}t^{\bar m}_{\bar n}\,{}^{A}t^{n\bar a}_{i\bar j} - {}^{A}t^{n}_{i}\,{}^{A}t^{\bar m}_{\bar j}\,{}^{A}t^{b\bar a}_{m\bar n}\\
&+ {}^{A}t^{n}_{i}\,{}^{A}t^{\bar m}_{\bar n}\,{}^{A}t^{b\bar a}_{m\bar j} + {}^{A}t^{n}_{m}\,{}^{A}t^{\bar m}_{\bar j}\,{}^{A}t^{b\bar a}_{i\bar n} - {}^{A}t^{\bar a}_{\bar n}\,{}^{A}t^{b}_{m}\,{}^{A}t^{n}_{i}\,{}^{A}t^{\bar m}_{\bar j}]\\
&+ \delta(n,a)\,[- {}^{A}t^{b}_{m}\,{}^{A}t^{n\bar m}_{i\bar j} - {}^{A}t^{n}_{i}\,{}^{A}t^{b\bar m}_{m\bar j} + {}^{A}t^{n}_{m}\,{}^{A}t^{b\bar m}_{i\bar j} - {}^{A}t^{\bar m}_{\bar j}\,{}^{A}t^{bn}_{mi} - {}^{A}t^{b}_{m}\,{}^{A}t^{n}_{i}\,{}^{A}t^{\bar m}_{\bar j}]\\
&+ \delta(\bar m,\bar b)\,[- {}^{A}t^{\bar a}_{\bar n}\,{}^{A}t^{n\bar m}_{i\bar j} - {}^{A}t^{n}_{i}\,{}^{A}t^{\bar a\bar m}_{\bar n\bar j} - {}^{A}t^{\bar m}_{\bar j}\,{}^{A}t^{n\bar a}_{i\bar n} + {}^{A}t^{\bar m}_{\bar n}\,{}^{A}t^{n\bar a}_{i\bar j} - {}^{A}t^{\bar a}_{\bar n}\,{}^{A}t^{n}_{i}\,{}^{A}t^{\bar m}_{\bar j}]\\
&+ \delta(m,j)\,[+ {}^{A}t^{\bar a}_{\bar n}\,{}^{A}t^{bn}_{mi} + {}^{A}t^{b}_{m}\,{}^{A}t^{n\bar a}_{i\bar n} + {}^{A}t^{n}_{i}\,{}^{A}t^{b\bar a}_{m\bar n} - {}^{A}t^{n}_{m}\,{}^{A}t^{b\bar a}_{i\bar n} + {}^{A}t^{\bar a}_{\bar n}\,{}^{A}t^{b}_{m}\,{}^{A}t^{n}_{i}]\\
&+ \delta(\bar n,\bar i)\,[+ {}^{A}t^{\bar a}_{\bar n}\,{}^{A}t^{b\bar m}_{m\bar j} + {}^{A}t^{b}_{m}\,{}^{A}t^{\bar a\bar m}_{\bar n\bar j} + {}^{A}t^{\bar m}_{\bar j}\,{}^{A}t^{b\bar a}_{m\bar n} - {}^{A}t^{\bar m}_{\bar n}\,{}^{A}t^{b\bar a}_{m\bar j} + {}^{A}t^{\bar a}_{\bar n}\,{}^{A}t^{b}_{m}\,{}^{A}t^{\bar m}_{\bar j}]\\
&+ \delta(\bar m,\bar b)\,\delta(n,a)\,[- {}^{A}t^{n\bar m}_{i\bar j} - {}^{A}t^{n}_{i}\,{}^{A}t^{\bar m}_{\bar j}]\\
&+ \delta(m,j)\,\delta(n,a)\,[+ {}^{A}t^{bn}_{mi} + {}^{A}t^{b}_{m}\,{}^{A}t^{n}_{i}]\\
&+ \delta(m,j)\,\delta(\bar m,\bar b)\,[+ {}^{A}t^{n\bar a}_{i\bar n} + {}^{A}t^{\bar a}_{\bar n}\,{}^{A}t^{n}_{i}]\\
&+ \delta(\bar n,\bar i)\,\delta(n,a)\,[+ {}^{A}t^{b\bar m}_{m\bar j} + {}^{A}t^{b}_{m}\,{}^{A}t^{\bar m}_{\bar j}]\\
&+ \delta(\bar n,\bar i)\,\delta(\bar m,\bar b)\,[+ {}^{A}t^{\bar a\bar m}_{\bar n\bar j} + {}^{A}t^{\bar a}_{\bar n}\,{}^{A}t^{\bar m}_{\bar j}]\\
&+ \delta(m,j)\,\delta(\bar n,\bar i)\,[- {}^{A}t^{b\bar a}_{m\bar n} - {}^{A}t^{\bar a}_{\bar n}\,{}^{A}t^{b}_{m}]\\
&+ \delta(m,j)\,\delta(n,a)\,\delta(\bar m,\bar b)\,[+ {}^{A}t^{n}_{i}]\\
&+ \delta(\bar n,\bar i)\,\delta(n,a)\,\delta(\bar m,\bar b)\,[+ {}^{A}t^{\bar m}_{\bar j}]\\
&+ \delta(m,j)\,\delta(\bar n,\bar i)\,\delta(n,a)\,[- {}^{A}t^{b}_{m}]\\
&+ \delta(m,j)\,\delta(\bar n,\bar i)\,\delta(\bar m,\bar b)\,[- {}^{A}t^{\bar a}_{\bar n}]
\end{aligned}
\tag{S50}
$$

$$
\begin{aligned}
M^{\bar a b}_{\bar i j} =&[- {}^{A}t^{a\bar b}_{m\bar j}\,{}^{A}t^{n\bar m}_{i\bar n} - {}^{A}t^{a\bar b}_{i\bar n}\,{}^{A}t^{n\bar m}_{m\bar j} + {}^{A}t^{a\bar b}_{m\bar n}\,{}^{A}t^{n\bar m}_{i\bar j} + {}^{A}t^{an}_{mi}\,{}^{A}t^{\bar b\bar m}_{\bar n\bar j} - {}^{A}t^{a\bar m}_{i\bar j}\,{}^{A}t^{n\bar b}_{m\bar n} + {}^{A}t^{a\bar m}_{m\bar j}\,{}^{A}t^{n\bar b}_{i\bar n}\\
&+ {}^{A}t^{a\bar m}_{i\bar n}\,{}^{A}t^{n\bar b}_{m\bar j} - {}^{A}t^{a\bar m}_{m\bar n}\,{}^{A}t^{n\bar b}_{i\bar j} + {}^{A}t^{a}_{m}\,{}^{A}t^{\bar b}_{\bar n}\,{}^{A}t^{n\bar m}_{i\bar j} + {}^{A}t^{a}_{m}\,{}^{A}t^{n}_{i}\,{}^{A}t^{\bar b\bar m}_{\bar n\bar j} + {}^{A}t^{a}_{m}\,{}^{A}t^{\bar m}_{\bar j}\,{}^{A}t^{n\bar b}_{i\bar n}\\
&- {}^{A}t^{a}_{m}\,{}^{A}t^{\bar m}_{\bar n}\,{}^{A}t^{n\bar b}_{i\bar j} + {}^{A}t^{\bar b}_{\bar n}\,{}^{A}t^{n}_{i}\,{}^{A}t^{a\bar m}_{m\bar j} - {}^{A}t^{\bar b}_{\bar n}\,{}^{A}t^{n}_{m}\,{}^{A}t^{a\bar m}_{i\bar j} + {}^{A}t^{\bar b}_{\bar n}\,{}^{A}t^{\bar m}_{\bar j}\,{}^{A}t^{an}_{mi} + {}^{A}t^{n}_{i}\,{}^{A}t^{\bar m}_{\bar j}\,{}^{A}t^{a\bar b}_{m\bar n}\\
&- {}^{A}t^{n}_{i}\,{}^{A}t^{\bar m}_{\bar n}\,{}^{A}t^{a\bar b}_{m\bar j} - {}^{A}t^{n}_{m}\,{}^{A}t^{\bar m}_{\bar j}\,{}^{A}t^{a\bar b}_{i\bar n} + {}^{A}t^{a}_{m}\,{}^{A}t^{\bar b}_{\bar n}\,{}^{A}t^{n}_{i}\,{}^{A}t^{\bar m}_{\bar j}]\\
&+ \delta(\bar m,\bar a)\,[+ {}^{A}t^{\bar b}_{\bar n}\,{}^{A}t^{n\bar m}_{i\bar j} + {}^{A}t^{n}_{i}\,{}^{A}t^{\bar b\bar m}_{\bar n\bar j} + {}^{A}t^{\bar m}_{\bar j}\,{}^{A}t^{n\bar b}_{i\bar n} - {}^{A}t^{\bar m}_{\bar n}\,{}^{A}t^{n\bar b}_{i\bar j} + {}^{A}t^{\bar b}_{\bar n}\,{}^{A}t^{n}_{i}\,{}^{A}t^{\bar m}_{\bar j}]\\
&+ \delta(n,b)\,[+ {}^{A}t^{a}_{m}\,{}^{A}t^{n\bar m}_{i\bar j} + {}^{A}t^{n}_{i}\,{}^{A}t^{a\bar m}_{m\bar j} - {}^{A}t^{n}_{m}\,{}^{A}t^{a\bar m}_{i\bar j} + {}^{A}t^{\bar m}_{\bar j}\,{}^{A}t^{an}_{mi} + {}^{A}t^{a}_{m}\,{}^{A}t^{n}_{i}\,{}^{A}t^{\bar m}_{\bar j}]\\
&+ \delta(m,j)\,[- {}^{A}t^{a}_{m}\,{}^{A}t^{n\bar b}_{i\bar n} - {}^{A}t^{\bar b}_{\bar n}\,{}^{A}t^{an}_{mi} - {}^{A}t^{n}_{i}\,{}^{A}t^{a\bar b}_{m\bar n} + {}^{A}t^{n}_{m}\,{}^{A}t^{a\bar b}_{i\bar n} - {}^{A}t^{a}_{m}\,{}^{A}t^{\bar b}_{\bar n}\,{}^{A}t^{n}_{i}]\\
&+ \delta(\bar n,\bar i)\,[- {}^{A}t^{a}_{m}\,{}^{A}t^{\bar b\bar m}_{\bar n\bar j} - {}^{A}t^{\bar b}_{\bar n}\,{}^{A}t^{a\bar m}_{m\bar j} - {}^{A}t^{\bar m}_{\bar j}\,{}^{A}t^{a\bar b}_{m\bar n} + {}^{A}t^{\bar m}_{\bar n}\,{}^{A}t^{a\bar b}_{m\bar j} - {}^{A}t^{a}_{m}\,{}^{A}t^{\bar b}_{\bar n}\,{}^{A}t^{\bar m}_{\bar j}]\\
&+ \delta(\bar m,\bar a)\,\delta(n,b)\,[+ {}^{A}t^{n\bar m}_{i\bar j} + {}^{A}t^{n}_{i}\,{}^{A}t^{\bar m}_{\bar j}]\\
&+ \delta(m,j)\,\delta(\bar m,\bar a)\,[- {}^{A}t^{n\bar b}_{i\bar n} - {}^{A}t^{\bar b}_{\bar n}\,{}^{A}t^{n}_{i}]\\
&+ \delta(m,j)\,\delta(n,b)\,[- {}^{A}t^{an}_{mi} - {}^{A}t^{a}_{m}\,{}^{A}t^{n}_{i}]\\
&+ \delta(\bar n,\bar i)\,\delta(\bar m,\bar a)\,[- {}^{A}t^{\bar b\bar m}_{\bar n\bar j} - {}^{A}t^{\bar b}_{\bar n}\,{}^{A}t^{\bar m}_{\bar j}]\\
&+ \delta(\bar n,\bar i)\,\delta(n,b)\,[- {}^{A}t^{a\bar m}_{m\bar j} - {}^{A}t^{a}_{m}\,{}^{A}t^{\bar m}_{\bar j}]\\
&+ \delta(m,j)\,\delta(\bar n,\bar i)\,[+ {}^{A}t^{a\bar b}_{m\bar n} + {}^{A}t^{a}_{m}\,{}^{A}t^{\bar b}_{\bar n}]\\
&+ \delta(m,j)\,\delta(n,b)\,\delta(\bar m,\bar a)\,[- {}^{A}t^{n}_{i}]\\
&+ \delta(\bar n,\bar i)\,\delta(n,b)\,\delta(\bar m,\bar a)\,[- {}^{A}t^{\bar m}_{\bar j}]\\
&+ \delta(m,j)\,\delta(\bar n,\bar i)\,\delta(\bar m,\bar a)\,[+ {}^{A}t^{\bar b}_{\bar n}]\\
&+ \delta(m,j)\,\delta(\bar n,\bar i)\,\delta(n,b)\,[+ {}^{A}t^{a}_{m}]
\end{aligned}
\tag{S51}
$$

$$
M^{\bar a\bar b}_{\bar i j} = 0 \tag{S52}
$$

$$M_{\bar{i}\bar{j}}^{ab} = 0 \tag{S53}$$

$$M_{\bar{i}\bar{j}}^{a\bar{b}} = 0 \tag{S54}$$

$$M_{\bar{i}\bar{j}}^{\bar{a}b} = 0 \tag{S55}$$

$$\begin{aligned}
M_{\bar{i}\bar{j}}^{\bar{a}\bar{b}} =&[- {}^{A}t_{mj}^{ab}\, {}^{A}t_{i\bar{n}}^{n\bar{m}} + {}^{A}t_{mi}^{ab}\, {}^{A}t_{j\bar{n}}^{n\bar{m}} - {}^{A}t_{ij}^{an}\, {}^{A}t_{m\bar{n}}^{b\bar{m}} + {}^{A}t_{mj}^{an}\, {}^{A}t_{i\bar{n}}^{b\bar{m}} - {}^{A}t_{mi}^{an}\, {}^{A}t_{j\bar{n}}^{b\bar{m}} + {}^{A}t_{j\bar{n}}^{a\bar{m}}\, {}^{A}t_{mi}^{bn} - {}^{A}t_{i\bar{n}}^{a\bar{m}}\, {}^{A}t_{mj}^{bn} \\
& + {}^{A}t_{m\bar{n}}^{a\bar{m}}\, {}^{A}t_{ij}^{bn} + {}^{A}t_{m}^{a}\, {}^{A}t_{j}^{n}\, {}^{A}t_{i\bar{n}}^{b\bar{m}} - {}^{A}t_{m}^{a}\, {}^{A}t_{i}^{n}\, {}^{A}t_{j\bar{n}}^{b\bar{m}} + {}^{A}t_{m}^{a}\, {}^{A}t_{\bar{n}}^{\bar{m}}\, {}^{A}t_{ij}^{bn} - {}^{A}t_{m}^{b}\, {}^{A}t_{j}^{n}\, {}^{A}t_{i\bar{n}}^{a\bar{m}} + {}^{A}t_{m}^{b}\, {}^{A}t_{i}^{n}\, {}^{A}t_{j\bar{n}}^{a\bar{m}} \\
& - {}^{A}t_{m}^{b}\, {}^{A}t_{\bar{n}}^{\bar{m}}\, {}^{A}t_{ij}^{an} + {}^{A}t_{j}^{n}\, {}^{A}t_{\bar{n}}^{\bar{m}}\, {}^{A}t_{mi}^{ab} - {}^{A}t_{i}^{n}\, {}^{A}t_{\bar{n}}^{\bar{m}}\, {}^{A}t_{mj}^{ab}] \\
& + \delta(\bar{m},\bar{a})\, [+ {}^{A}t_{j}^{n}\, {}^{A}t_{i\bar{n}}^{b\bar{m}} - {}^{A}t_{i}^{n}\, {}^{A}t_{j\bar{n}}^{b\bar{m}} + {}^{A}t_{\bar{n}}^{\bar{m}}\, {}^{A}t_{ij}^{bn}] \\
& + \delta(\bar{m},\bar{b})\, [- {}^{A}t_{j}^{n}\, {}^{A}t_{i\bar{n}}^{a\bar{m}} + {}^{A}t_{i}^{n}\, {}^{A}t_{j\bar{n}}^{a\bar{m}} - {}^{A}t_{\bar{n}}^{\bar{m}}\, {}^{A}t_{ij}^{an}] \\
& + \delta(\bar{n},\bar{j})\, [- {}^{A}t_{m}^{a}\, {}^{A}t_{i\bar{n}}^{b\bar{m}} + {}^{A}t_{m}^{b}\, {}^{A}t_{i\bar{n}}^{a\bar{m}} - {}^{A}t_{\bar{n}}^{\bar{m}}\, {}^{A}t_{mi}^{ab}] \\
& + \delta(\bar{n},\bar{i})\, [+ {}^{A}t_{m}^{a}\, {}^{A}t_{j\bar{n}}^{b\bar{m}} - {}^{A}t_{m}^{b}\, {}^{A}t_{j\bar{n}}^{a\bar{m}} + {}^{A}t_{\bar{n}}^{\bar{m}}\, {}^{A}t_{mj}^{ab}] \\
& + \delta(\bar{n},\bar{j})\, \delta(\bar{m},\bar{a})\, [- {}^{A}t_{i\bar{n}}^{b\bar{m}}] \\
& + \delta(\bar{n},\bar{j})\, \delta(\bar{m},\bar{b})\, [+ {}^{A}t_{i\bar{n}}^{a\bar{m}}] \\
& + \delta(\bar{n},\bar{i})\, \delta(\bar{m},\bar{a})\, [+ {}^{A}t_{j\bar{n}}^{b\bar{m}}] \\
& + \delta(\bar{n},\bar{i})\, \delta(\bar{m},\bar{b})\, [- {}^{A}t_{j\bar{n}}^{a\bar{m}}]
\end{aligned} \tag{S56}$$

### C. $M_{ij}^{ab}$ disconnected contributions

$$
\begin{aligned}
M_{ij}^{ab} =\big[ & + {}^{A}t_{i}^{a}\, {}^{A}t_{\bar{n}}^{\bar{b}}\, {}^{A}t_{m\bar{j}}^{n\bar{m}} + {}^{A}t_{i}^{a}\, {}^{A}t_{m}^{n}\, {}^{A}t_{\bar{n}\bar{j}}^{\bar{b}\bar{m}} + {}^{A}t_{i}^{a}\, {}^{A}t_{\bar{j}}^{\bar{m}}\, {}^{A}t_{m\bar{n}}^{n\bar{b}} - {}^{A}t_{i}^{a}\, {}^{A}t_{\bar{n}}^{\bar{m}}\, {}^{A}t_{m\bar{j}}^{n\bar{b}} + {}^{A}t_{i}^{a}\, {}^{A}t_{\bar{n}}^{\bar{b}}\, {}^{A}t_{m}^{n}\, {}^{A}t_{\bar{j}}^{\bar{m}} \\
& - {}^{A}t_{j}^{a}\, {}^{A}t_{\bar{n}}^{\bar{b}}\, {}^{A}t_{m\bar{i}}^{n\bar{m}} - {}^{A}t_{j}^{a}\, {}^{A}t_{m}^{n}\, {}^{A}t_{\bar{n}\bar{i}}^{\bar{b}\bar{m}} - {}^{A}t_{j}^{a}\, {}^{A}t_{\bar{i}}^{\bar{m}}\, {}^{A}t_{m\bar{n}}^{n\bar{b}} + {}^{A}t_{j}^{a}\, {}^{A}t_{\bar{n}}^{\bar{m}}\, {}^{A}t_{m\bar{i}}^{n\bar{b}} - {}^{A}t_{j}^{a}\, {}^{A}t_{\bar{n}}^{\bar{b}}\, {}^{A}t_{m}^{n}\, {}^{A}t_{\bar{i}}^{\bar{m}} \\
& - {}^{A}t_{i}^{b}\, {}^{A}t_{\bar{n}}^{\bar{a}}\, {}^{A}t_{m\bar{j}}^{n\bar{m}} - {}^{A}t_{i}^{b}\, {}^{A}t_{m}^{n}\, {}^{A}t_{\bar{n}\bar{j}}^{\bar{a}\bar{m}} - {}^{A}t_{i}^{b}\, {}^{A}t_{\bar{j}}^{\bar{m}}\, {}^{A}t_{m\bar{n}}^{n\bar{a}} + {}^{A}t_{i}^{b}\, {}^{A}t_{\bar{n}}^{\bar{m}}\, {}^{A}t_{m\bar{j}}^{n\bar{a}} - {}^{A}t_{i}^{b}\, {}^{A}t_{\bar{n}}^{\bar{a}}\, {}^{A}t_{m}^{n}\, {}^{A}t_{\bar{j}}^{\bar{m}} \\
& + {}^{A}t_{j}^{b}\, {}^{A}t_{\bar{n}}^{\bar{a}}\, {}^{A}t_{m\bar{i}}^{n\bar{m}} + {}^{A}t_{j}^{b}\, {}^{A}t_{m}^{n}\, {}^{A}t_{\bar{n}\bar{i}}^{\bar{a}\bar{m}} + {}^{A}t_{j}^{b}\, {}^{A}t_{\bar{i}}^{\bar{m}}\, {}^{A}t_{m\bar{n}}^{n\bar{a}} - {}^{A}t_{j}^{b}\, {}^{A}t_{\bar{n}}^{\bar{m}}\, {}^{A}t_{m\bar{i}}^{n\bar{a}} + {}^{A}t_{j}^{b}\, {}^{A}t_{\bar{n}}^{\bar{a}}\, {}^{A}t_{m}^{n}\, {}^{A}t_{\bar{i}}^{\bar{m}} \\
& - {}^{A}t_{\bar{i}}^{\bar{a}}\, {}^{A}t_{\bar{n}}^{\bar{b}}\, {}^{A}t_{m\bar{j}}^{n\bar{m}} - {}^{A}t_{\bar{i}}^{\bar{a}}\, {}^{A}t_{m}^{n}\, {}^{A}t_{\bar{n}\bar{j}}^{\bar{b}\bar{m}} - {}^{A}t_{\bar{i}}^{\bar{a}}\, {}^{A}t_{\bar{j}}^{\bar{m}}\, {}^{A}t_{m\bar{n}}^{n\bar{b}} + {}^{A}t_{\bar{i}}^{\bar{a}}\, {}^{A}t_{\bar{n}}^{\bar{m}}\, {}^{A}t_{m\bar{j}}^{n\bar{b}} \\
& - {}^{A}t_{\bar{i}}^{\bar{a}}\, {}^{A}t_{\bar{n}}^{\bar{b}}\, {}^{A}t_{m}^{n}\, {}^{A}t_{\bar{j}}^{\bar{m}} + {}^{A}t_{\bar{j}}^{\bar{a}}\, {}^{A}t_{\bar{n}}^{\bar{b}}\, {}^{A}t_{m\bar{i}}^{n\bar{m}} + {}^{A}t_{\bar{j}}^{\bar{a}}\, {}^{A}t_{m}^{n}\, {}^{A}t_{\bar{n}\bar{i}}^{\bar{b}\bar{m}} + {}^{A}t_{\bar{j}}^{\bar{a}}\, {}^{A}t_{\bar{i}}^{\bar{m}}\, {}^{A}t_{m\bar{n}}^{n\bar{b}} \\
& - {}^{A}t_{\bar{j}}^{\bar{a}}\, {}^{A}t_{\bar{n}}^{\bar{m}}\, {}^{A}t_{m\bar{i}}^{n\bar{b}} + {}^{A}t_{\bar{j}}^{\bar{a}}\, {}^{A}t_{\bar{n}}^{\bar{b}}\, {}^{A}t_{m}^{n}\, {}^{A}t_{\bar{i}}^{\bar{m}} + {}^{A}t_{\bar{i}}^{\bar{b}}\, {}^{A}t_{\bar{n}}^{\bar{a}}\, {}^{A}t_{m\bar{j}}^{n\bar{m}} + {}^{A}t_{\bar{i}}^{\bar{b}}\, {}^{A}t_{m}^{n}\, {}^{A}t_{\bar{n}\bar{j}}^{\bar{a}\bar{m}} \\
& + {}^{A}t_{\bar{i}}^{\bar{b}}\, {}^{A}t_{\bar{j}}^{\bar{m}}\, {}^{A}t_{m\bar{n}}^{n\bar{a}} - {}^{A}t_{\bar{i}}^{\bar{b}}\, {}^{A}t_{\bar{n}}^{\bar{m}}\, {}^{A}t_{m\bar{j}}^{n\bar{a}} + {}^{A}t_{\bar{i}}^{\bar{b}}\, {}^{A}t_{\bar{n}}^{\bar{a}}\, {}^{A}t_{m}^{n}\, {}^{A}t_{\bar{j}}^{\bar{m}} - {}^{A}t_{\bar{j}}^{\bar{b}}\, {}^{A}t_{\bar{n}}^{\bar{a}}\, {}^{A}t_{m\bar{i}}^{n\bar{m}} \\
& - {}^{A}t_{\bar{j}}^{\bar{b}}\, {}^{A}t_{m}^{n}\, {}^{A}t_{\bar{n}\bar{i}}^{\bar{a}\bar{m}} - {}^{A}t_{\bar{j}}^{\bar{b}}\, {}^{A}t_{\bar{i}}^{\bar{m}}\, {}^{A}t_{m\bar{n}}^{n\bar{a}} + {}^{A}t_{\bar{j}}^{\bar{b}}\, {}^{A}t_{\bar{n}}^{\bar{m}}\, {}^{A}t_{m\bar{i}}^{n\bar{a}} - {}^{A}t_{\bar{j}}^{\bar{b}}\, {}^{A}t_{\bar{n}}^{\bar{a}}\, {}^{A}t_{m}^{n}\, {}^{A}t_{\bar{i}}^{\bar{m}} \big] \\
& + \delta(n,b)\, \big[ + {}^{A}t_{i}^{a}\, {}^{A}t_{m\bar{j}}^{n\bar{m}} + {}^{A}t_{i}^{a}\, {}^{A}t_{m}^{n}\, {}^{A}t_{\bar{j}}^{\bar{m}} - {}^{A}t_{j}^{a}\, {}^{A}t_{m\bar{i}}^{n\bar{m}} - {}^{A}t_{j}^{a}\, {}^{A}t_{m}^{n}\, {}^{A}t_{\bar{i}}^{\bar{m}} - {}^{A}t_{i}^{n}\, {}^{A}t_{\bar{n}}^{\bar{a}}\, {}^{A}t_{m\bar{j}}^{n\bar{m}} - {}^{A}t_{i}^{n}\, {}^{A}t_{m}^{n}\, {}^{A}t_{\bar{n}\bar{j}}^{\bar{a}\bar{m}} \\
& - {}^{A}t_{i}^{n}\, {}^{A}t_{\bar{j}}^{\bar{m}}\, {}^{A}t_{m\bar{n}}^{n\bar{a}} + {}^{A}t_{i}^{n}\, {}^{A}t_{\bar{n}}^{\bar{m}}\, {}^{A}t_{m\bar{j}}^{n\bar{a}} - {}^{A}t_{i}^{n}\, {}^{A}t_{\bar{n}}^{\bar{a}}\, {}^{A}t_{m}^{n}\, {}^{A}t_{\bar{j}}^{\bar{m}} + {}^{A}t_{j}^{n}\, {}^{A}t_{\bar{n}}^{\bar{a}}\, {}^{A}t_{m\bar{i}}^{n\bar{m}} \\
& + {}^{A}t_{j}^{n}\, {}^{A}t_{m}^{n}\, {}^{A}t_{\bar{n}\bar{i}}^{\bar{a}\bar{m}} + {}^{A}t_{j}^{n}\, {}^{A}t_{\bar{i}}^{\bar{m}}\, {}^{A}t_{m\bar{n}}^{n\bar{a}} - {}^{A}t_{j}^{n}\, {}^{A}t_{\bar{n}}^{\bar{m}}\, {}^{A}t_{m\bar{i}}^{n\bar{a}} + {}^{A}t_{j}^{n}\, {}^{A}t_{\bar{n}}^{\bar{a}}\, {}^{A}t_{m}^{n}\, {}^{A}t_{\bar{i}}^{\bar{m}} \\
& - {}^{A}t_{\bar{i}}^{\bar{a}}\, {}^{A}t_{m\bar{j}}^{n\bar{m}} - {}^{A}t_{\bar{i}}^{\bar{a}}\, {}^{A}t_{m}^{n}\, {}^{A}t_{\bar{j}}^{\bar{m}} + {}^{A}t_{\bar{j}}^{\bar{a}}\, {}^{A}t_{m\bar{i}}^{n\bar{m}} + {}^{A}t_{\bar{j}}^{\bar{a}}\, {}^{A}t_{m}^{n}\, {}^{A}t_{\bar{i}}^{\bar{m}} \big] \\
& + \delta(m,j)\, \big[ - {}^{A}t_{i}^{a}\, {}^{A}t_{m\bar{n}}^{n\bar{b}} - {}^{A}t_{i}^{a}\, {}^{A}t_{\bar{n}}^{\bar{b}}\, {}^{A}t_{m}^{n} - {}^{A}t_{m}^{a}\, {}^{A}t_{\bar{n}}^{\bar{b}}\, {}^{A}t_{m\bar{i}}^{n\bar{m}} - {}^{A}t_{m}^{a}\, {}^{A}t_{m}^{n}\, {}^{A}t_{\bar{n}\bar{i}}^{\bar{b}\bar{m}} - {}^{A}t_{m}^{a}\, {}^{A}t_{\bar{i}}^{\bar{m}}\, {}^{A}t_{m\bar{n}}^{n\bar{b}} \\
& + {}^{A}t_{m}^{a}\, {}^{A}t_{\bar{n}}^{\bar{m}}\, {}^{A}t_{m\bar{i}}^{n\bar{b}} - {}^{A}t_{m}^{a}\, {}^{A}t_{\bar{n}}^{\bar{b}}\, {}^{A}t_{m}^{n}\, {}^{A}t_{\bar{i}}^{\bar{m}} + {}^{A}t_{i}^{b}\, {}^{A}t_{m\bar{n}}^{n\bar{a}} + {}^{A}t_{i}^{b}\, {}^{A}t_{\bar{n}}^{\bar{a}}\, {}^{A}t_{m}^{n} + {}^{A}t_{m}^{b}\, {}^{A}t_{\bar{n}}^{\bar{a}}\, {}^{A}t_{m\bar{i}}^{n\bar{m}} \\
& + {}^{A}t_{m}^{b}\, {}^{A}t_{m}^{n}\, {}^{A}t_{\bar{n}\bar{i}}^{\bar{a}\bar{m}} + {}^{A}t_{m}^{b}\, {}^{A}t_{\bar{i}}^{\bar{m}}\, {}^{A}t_{m\bar{n}}^{n\bar{a}} - {}^{A}t_{m}^{b}\, {}^{A}t_{\bar{n}}^{\bar{m}}\, {}^{A}t_{m\bar{i}}^{n\bar{a}} + {}^{A}t_{m}^{b}\, {}^{A}t_{\bar{n}}^{\bar{a}}\, {}^{A}t_{m}^{n}\, {}^{A}t_{\bar{i}}^{\bar{m}} \\
& + {}^{A}t_{\bar{i}}^{\bar{a}}\, {}^{A}t_{m\bar{n}}^{n\bar{b}} + {}^{A}t_{\bar{i}}^{\bar{a}}\, {}^{A}t_{\bar{n}}^{\bar{b}}\, {}^{A}t_{m}^{n} - {}^{A}t_{\bar{i}}^{\bar{b}}\, {}^{A}t_{m\bar{n}}^{n\bar{a}} - {}^{A}t_{\bar{i}}^{\bar{b}}\, {}^{A}t_{\bar{n}}^{\bar{a}}\, {}^{A}t_{m}^{n} \big] \\
& + \delta(n,a)\, \big[ + {}^{A}t_{i}^{n}\, {}^{A}t_{\bar{n}}^{\bar{b}}\, {}^{A}t_{m\bar{j}}^{n\bar{m}} + {}^{A}t_{i}^{n}\, {}^{A}t_{m}^{n}\, {}^{A}t_{\bar{n}\bar{j}}^{\bar{b}\bar{m}} + {}^{A}t_{i}^{n}\, {}^{A}t_{\bar{j}}^{\bar{m}}\, {}^{A}t_{m\bar{n}}^{n\bar{b}} - {}^{A}t_{i}^{n}\, {}^{A}t_{\bar{n}}^{\bar{m}}\, {}^{A}t_{m\bar{j}}^{n\bar{b}} + {}^{A}t_{i}^{n}\, {}^{A}t_{\bar{n}}^{\bar{b}}\, {}^{A}t_{m}^{n}\, {}^{A}t_{\bar{j}}^{\bar{m}} \\
& - {}^{A}t_{j}^{n}\, {}^{A}t_{\bar{n}}^{\bar{b}}\, {}^{A}t_{m\bar{i}}^{n\bar{m}} - {}^{A}t_{j}^{n}\, {}^{A}t_{m}^{n}\, {}^{A}t_{\bar{n}\bar{i}}^{\bar{b}\bar{m}} - {}^{A}t_{j}^{n}\, {}^{A}t_{\bar{i}}^{\bar{m}}\, {}^{A}t_{m\bar{n}}^{n\bar{b}} + {}^{A}t_{j}^{n}\, {}^{A}t_{\bar{n}}^{\bar{m}}\, {}^{A}t_{m\bar{i}}^{n\bar{b}} - {}^{A}t_{j}^{n}\, {}^{A}t_{\bar{n}}^{\bar{b}}\, {}^{A}t_{m}^{n}\, {}^{A}t_{\bar{i}}^{\bar{m}} \\
& - {}^{A}t_{i}^{b}\, {}^{A}t_{m\bar{j}}^{n\bar{m}} - {}^{A}t_{i}^{b}\, {}^{A}t_{m}^{n}\, {}^{A}t_{\bar{j}}^{\bar{m}} + {}^{A}t_{j}^{b}\, {}^{A}t_{m\bar{i}}^{n\bar{m}} + {}^{A}t_{j}^{b}\, {}^{A}t_{m}^{n}\, {}^{A}t_{\bar{i}}^{\bar{m}} + {}^{A}t_{\bar{i}}^{\bar{b}}\, {}^{A}t_{m\bar{j}}^{n\bar{m}} + {}^{A}t_{\bar{i}}^{\bar{b}}\, {}^{A}t_{m}^{n}\, {}^{A}t_{\bar{j}}^{\bar{m}} \\
& - {}^{A}t_{\bar{j}}^{\bar{b}}\, {}^{A}t_{m\bar{i}}^{n\bar{m}} - {}^{A}t_{\bar{j}}^{\bar{b}}\, {}^{A}t_{m}^{n}\, {}^{A}t_{\bar{i}}^{\bar{m}} \big] \\
& + \delta(m,i)\, \big[ + {}^{A}t_{m}^{a}\, {}^{A}t_{\bar{n}}^{\bar{b}}\, {}^{A}t_{m\bar{j}}^{n\bar{m}} + {}^{A}t_{m}^{a}\, {}^{A}t_{m}^{n}\, {}^{A}t_{\bar{n}\bar{j}}^{\bar{b}\bar{m}} + {}^{A}t_{m}^{a}\, {}^{A}t_{\bar{j}}^{\bar{m}}\, {}^{A}t_{m\bar{n}}^{n\bar{b}} - {}^{A}t_{m}^{a}\, {}^{A}t_{\bar{n}}^{\bar{m}}\, {}^{A}t_{m\bar{j}}^{n\bar{b}} + {}^{A}t_{m}^{a}\, {}^{A}t_{\bar{n}}^{\bar{b}}\, {}^{A}t_{m}^{n}\, {}^{A}t_{\bar{j}}^{\bar{m}} \\
& + {}^{A}t_{j}^{a}\, {}^{A}t_{m\bar{n}}^{n\bar{b}} + {}^{A}t_{j}^{a}\, {}^{A}t_{\bar{n}}^{\bar{b}}\, {}^{A}t_{m}^{n} - {}^{A}t_{m}^{b}\, {}^{A}t_{\bar{n}}^{\bar{a}}\, {}^{A}t_{m\bar{j}}^{n\bar{m}} - {}^{A}t_{m}^{b}\, {}^{A}t_{m}^{n}\, {}^{A}t_{\bar{n}\bar{j}}^{\bar{a}\bar{m}} - {}^{A}t_{m}^{b}\, {}^{A}t_{\bar{j}}^{\bar{m}}\, {}^{A}t_{m\bar{n}}^{n\bar{a}} \\
& + {}^{A}t_{m}^{b}\, {}^{A}t_{\bar{n}}^{\bar{m}}\, {}^{A}t_{m\bar{j}}^{n\bar{a}} - {}^{A}t_{m}^{b}\, {}^{A}t_{\bar{n}}^{\bar{a}}\, {}^{A}t_{m}^{n}\, {}^{A}t_{\bar{j}}^{\bar{m}} - {}^{A}t_{j}^{b}\, {}^{A}t_{m\bar{n}}^{n\bar{a}} - {}^{A}t_{j}^{b}\, {}^{A}t_{\bar{n}}^{\bar{a}}\, {}^{A}t_{m}^{n} - {}^{A}t_{\bar{j}}^{\bar{a}}\, {}^{A}t_{m\bar{n}}^{n\bar{b}} \\
& - {}^{A}t_{\bar{j}}^{\bar{a}}\, {}^{A}t_{\bar{n}}^{\bar{b}}\, {}^{A}t_{m}^{n} + {}^{A}t_{\bar{j}}^{\bar{b}}\, {}^{A}t_{m\bar{n}}^{n\bar{a}} + {}^{A}t_{\bar{j}}^{\bar{b}}\, {}^{A}t_{\bar{n}}^{\bar{a}}\, {}^{A}t_{m}^{n} \big] \\
& + \delta(m,j)\, \delta(n,b)\, \big[ - {}^{A}t_{i}^{a}\, {}^{A}t_{m}^{n} - {}^{A}t_{m}^{a}\, {}^{A}t_{m\bar{i}}^{n\bar{m}} - {}^{A}t_{m}^{a}\, {}^{A}t_{m}^{n}\, {}^{A}t_{\bar{i}}^{\bar{m}} + {}^{A}t_{i}^{n}\, {}^{A}t_{m\bar{n}}^{n\bar{a}} + {}^{A}t_{i}^{n}\, {}^{A}t_{\bar{n}}^{\bar{a}}\, {}^{A}t_{m}^{n} + {}^{A}t_{m}^{n}\, {}^{A}t_{\bar{n}}^{\bar{a}}\, {}^{A}t_{m\bar{i}}^{n\bar{m}} \\
& + {}^{A}t_{m}^{n}\, {}^{A}t_{m}^{n}\, {}^{A}t_{\bar{n}\bar{i}}^{\bar{a}\bar{m}} + {}^{A}t_{m}^{n}\, {}^{A}t_{\bar{i}}^{\bar{m}}\, {}^{A}t_{m\bar{n}}^{n\bar{a}} - {}^{A}t_{m}^{n}\, {}^{A}t_{\bar{n}}^{\bar{m}}\, {}^{A}t_{m\bar{i}}^{n\bar{a}} + {}^{A}t_{m}^{n}\, {}^{A}t_{\bar{n}}^{\bar{a}}\, {}^{A}t_{m}^{n}\, {}^{A}t_{\bar{i}}^{\bar{m}} \\
& + {}^{A}t_{\bar{i}}^{\bar{a}}\, {}^{A}t_{m}^{n} \big] \\
& + \delta(m,j)\, \delta(n,a)\, \big[ - {}^{A}t_{i}^{n}\, {}^{A}t_{m\bar{n}}^{n\bar{b}} - {}^{A}t_{i}^{n}\, {}^{A}t_{\bar{n}}^{\bar{b}}\, {}^{A}t_{m}^{n} - {}^{A}t_{m}^{n}\, {}^{A}t_{\bar{n}}^{\bar{b}}\, {}^{A}t_{m\bar{i}}^{n\bar{m}} - {}^{A}t_{m}^{n}\, {}^{A}t_{m}^{n}\, {}^{A}t_{\bar{n}\bar{i}}^{\bar{b}\bar{m}} - {}^{A}t_{m}^{n}\, {}^{A}t_{\bar{i}}^{\bar{m}}\, {}^{A}t_{m\bar{n}}^{n\bar{b}} \\
& + {}^{A}t_{m}^{n}\, {}^{A}t_{\bar{n}}^{\bar{m}}\, {}^{A}t_{m\bar{i}}^{n\bar{b}} - {}^{A}t_{m}^{n}\, {}^{A}t_{\bar{n}}^{\bar{b}}\, {}^{A}t_{m}^{n}\, {}^{A}t_{\bar{i}}^{\bar{m}} + {}^{A}t_{i}^{b}\, {}^{A}t_{m}^{n} + {}^{A}t_{m}^{b}\, {}^{A}t_{m\bar{i}}^{n\bar{m}} + {}^{A}t_{m}^{b}\, {}^{A}t_{m}^{n}\, {}^{A}t_{\bar{i}}^{\bar{m}} - {}^{A}t_{\bar{i}}^{\bar{b}}\, {}^{A}t_{m}^{n} \big] \\
& + \delta(m,i)\, \delta(n,b)\, \big[ + {}^{A}t_{m}^{a}\, {}^{A}t_{m\bar{j}}^{n\bar{m}} + {}^{A}t_{m}^{a}\, {}^{A}t_{m}^{n}\, {}^{A}t_{\bar{j}}^{\bar{m}} + {}^{A}t_{j}^{a}\, {}^{A}t_{m}^{n} - {}^{A}t_{m}^{n}\, {}^{A}t_{\bar{n}}^{\bar{a}}\, {}^{A}t_{m\bar{j}}^{n\bar{m}} - {}^{A}t_{m}^{n}\, {}^{A}t_{m}^{n}\, {}^{A}t_{\bar{n}\bar{j}}^{\bar{a}\bar{m}} - {}^{A}t_{m}^{n}\, {}^{A}t_{\bar{j}}^{\bar{m}}\, {}^{A}t_{m\bar{n}}^{n\bar{a}} \\
& + {}^{A}t_{m}^{n}\, {}^{A}t_{\bar{n}}^{\bar{m}}\, {}^{A}t_{m\bar{j}}^{n\bar{a}} - {}^{A}t_{m}^{n}\, {}^{A}t_{\bar{n}}^{\bar{a}}\, {}^{A}t_{m}^{n}\, {}^{A}t_{\bar{j}}^{\bar{m}} - {}^{A}t_{j}^{n}\, {}^{A}t_{m\bar{n}}^{n\bar{a}} - {}^{A}t_{j}^{n}\, {}^{A}t_{\bar{n}}^{\bar{a}}\, {}^{A}t_{m}^{n} - {}^{A}t_{\bar{j}}^{\bar{a}}\, {}^{A}t_{m}^{n} \big] \\
& + \delta(m,i)\, \delta(n,a)\, \big[ + {}^{A}t_{m}^{n}\, {}^{A}t_{\bar{n}}^{\bar{b}}\, {}^{A}t_{m\bar{j}}^{n\bar{m}} + {}^{A}t_{m}^{n}\, {}^{A}t_{m}^{n}\, {}^{A}t_{\bar{n}\bar{j}}^{\bar{b}\bar{m}} + {}^{A}t_{m}^{n}\, {}^{A}t_{\bar{j}}^{\bar{m}}\, {}^{A}t_{m\bar{n}}^{n\bar{b}} - {}^{A}t_{m}^{n}\, {}^{A}t_{\bar{n}}^{\bar{m}}\, {}^{A}t_{m\bar{j}}^{n\bar{b}} + {}^{A}t_{m}^{n}\, {}^{A}t_{\bar{n}}^{\bar{b}}\, {}^{A}t_{m}^{n}\, {}^{A}t_{\bar{j}}^{\bar{m}} \\
& + {}^{A}t_{j}^{n}\, {}^{A}t_{m\bar{n}}^{n\bar{b}} + {}^{A}t_{j}^{n}\, {}^{A}t_{\bar{n}}^{\bar{b}}\, {}^{A}t_{m}^{n} - {}^{A}t_{m}^{b}\, {}^{A}t_{m\bar{j}}^{n\bar{m}} - {}^{A}t_{m}^{b}\, {}^{A}t_{m}^{n}\, {}^{A}t_{\bar{j}}^{\bar{m}} - {}^{A}t_{j}^{b}\, {}^{A}t_{m}^{n} + {}^{A}t_{\bar{j}}^{\bar{b}}\, {}^{A}t_{m}^{n} \big]
\end{aligned}
\tag{S57}
$$

$$M^{a\bar b}_{ij} = 0 \tag{S58}$$

$$M^{\bar a b}_{ij} = 0 \tag{S59}$$

$$M^{\bar a\bar b}_{ij} = 0 \tag{S60}$$

$$M^{ab}_{i\bar j} = 0 \tag{S61}$$

$$\begin{aligned}
M^{a\bar b}_{i\bar j} =&[+ {}^{A}t^{a}_{i}\,{}^{A}t^{b}_{m}\,{}^{A}t^{n\bar m}_{j\bar n} + {}^{A}t^{a}_{i}\,{}^{A}t^{n}_{j}\,{}^{A}t^{b\bar m}_{m\bar n} - {}^{A}t^{a}_{i}\,{}^{A}t^{n}_{m}\,{}^{A}t^{b\bar m}_{j\bar n} + {}^{A}t^{a}_{i}\,{}^{A}t^{\bar m}_{\bar n}\,{}^{A}t^{bn}_{mj} + {}^{A}t^{a}_{i}\,{}^{A}t^{b}_{m}\,{}^{A}t^{n}_{j}\,{}^{A}t^{\bar m}_{\bar n} \\
&+ {}^{A}t^{\bar b}_{\bar j}\,{}^{A}t^{\bar a}_{\bar n}\,{}^{A}t^{n\bar m}_{m\bar i} + {}^{A}t^{\bar b}_{\bar j}\,{}^{A}t^{n}_{m}\,{}^{A}t^{\bar a\bar m}_{\bar n\bar i} + {}^{A}t^{\bar b}_{\bar j}\,{}^{A}t^{\bar m}_{\bar i}\,{}^{A}t^{n\bar a}_{m\bar n} - {}^{A}t^{\bar b}_{\bar j}\,{}^{A}t^{\bar m}_{\bar n}\,{}^{A}t^{n\bar a}_{m\bar i} \\
&+ {}^{A}t^{\bar b}_{\bar j}\,{}^{A}t^{\bar a}_{\bar n}\,{}^{A}t^{n}_{m}\,{}^{A}t^{\bar m}_{\bar i} - {}^{A}t^{\bar a}_{\bar i}\,{}^{A}t^{b}_{m}\,{}^{A}t^{n\bar m}_{j\bar n} - {}^{A}t^{\bar a}_{\bar i}\,{}^{A}t^{n}_{j}\,{}^{A}t^{b\bar m}_{m\bar n} + {}^{A}t^{\bar a}_{\bar i}\,{}^{A}t^{n}_{m}\,{}^{A}t^{b\bar m}_{j\bar n} \\
&- {}^{A}t^{\bar a}_{\bar i}\,{}^{A}t^{\bar m}_{\bar n}\,{}^{A}t^{bn}_{mj} - {}^{A}t^{\bar a}_{\bar i}\,{}^{A}t^{b}_{m}\,{}^{A}t^{n}_{j}\,{}^{A}t^{\bar m}_{\bar n} - {}^{A}t^{b}_{j}\,{}^{A}t^{\bar a}_{\bar n}\,{}^{A}t^{n\bar m}_{m\bar i} - {}^{A}t^{b}_{j}\,{}^{A}t^{n}_{m}\,{}^{A}t^{\bar a\bar m}_{\bar n\bar i} \\
&- {}^{A}t^{b}_{j}\,{}^{A}t^{\bar m}_{\bar i}\,{}^{A}t^{n\bar a}_{m\bar n} + {}^{A}t^{b}_{j}\,{}^{A}t^{\bar m}_{\bar n}\,{}^{A}t^{n\bar a}_{m\bar i} - {}^{A}t^{b}_{j}\,{}^{A}t^{\bar a}_{\bar n}\,{}^{A}t^{n}_{m}\,{}^{A}t^{\bar m}_{\bar i}] \\
&+ \delta(\bar m,\bar b)\,[+ {}^{A}t^{a}_{i}\,{}^{A}t^{n\bar m}_{j\bar n} + {}^{A}t^{a}_{i}\,{}^{A}t^{n}_{j}\,{}^{A}t^{\bar m}_{\bar n} + {}^{A}t^{\bar m}_{\bar j}\,{}^{A}t^{\bar a}_{\bar n}\,{}^{A}t^{n\bar m}_{m\bar i} + {}^{A}t^{\bar m}_{\bar j}\,{}^{A}t^{n}_{m}\,{}^{A}t^{\bar a\bar m}_{\bar n\bar i} + {}^{A}t^{\bar m}_{\bar j}\,{}^{A}t^{\bar m}_{\bar i}\,{}^{A}t^{n\bar a}_{m\bar n} \\
&- {}^{A}t^{\bar m}_{\bar j}\,{}^{A}t^{\bar m}_{\bar n}\,{}^{A}t^{n\bar a}_{m\bar i} + {}^{A}t^{\bar m}_{\bar j}\,{}^{A}t^{\bar a}_{\bar n}\,{}^{A}t^{n}_{m}\,{}^{A}t^{\bar m}_{\bar i} - {}^{A}t^{\bar a}_{\bar i}\,{}^{A}t^{n\bar m}_{j\bar n} - {}^{A}t^{\bar a}_{\bar i}\,{}^{A}t^{n}_{j}\,{}^{A}t^{\bar m}_{\bar n}] \\
&+ \delta(\bar n,\bar j)\,[- {}^{A}t^{a}_{i}\,{}^{A}t^{b\bar m}_{m\bar n} - {}^{A}t^{a}_{i}\,{}^{A}t^{b}_{m}\,{}^{A}t^{\bar m}_{\bar n} + {}^{A}t^{\bar b}_{\bar n}\,{}^{A}t^{\bar a}_{\bar n}\,{}^{A}t^{n\bar m}_{m\bar i} + {}^{A}t^{\bar b}_{\bar n}\,{}^{A}t^{n}_{m}\,{}^{A}t^{\bar a\bar m}_{\bar n\bar i} + {}^{A}t^{\bar b}_{\bar n}\,{}^{A}t^{\bar m}_{\bar i}\,{}^{A}t^{n\bar a}_{m\bar n} \\
&- {}^{A}t^{\bar b}_{\bar n}\,{}^{A}t^{\bar m}_{\bar n}\,{}^{A}t^{n\bar a}_{m\bar i} + {}^{A}t^{\bar b}_{\bar n}\,{}^{A}t^{\bar a}_{\bar n}\,{}^{A}t^{n}_{m}\,{}^{A}t^{\bar m}_{\bar i} + {}^{A}t^{\bar a}_{\bar i}\,{}^{A}t^{b\bar m}_{m\bar n} + {}^{A}t^{\bar a}_{\bar i}\,{}^{A}t^{b}_{m}\,{}^{A}t^{\bar m}_{\bar n}] \\
&+ \delta(n,a)\,[+ {}^{A}t^{n}_{i}\,{}^{A}t^{b}_{m}\,{}^{A}t^{n\bar m}_{j\bar n} + {}^{A}t^{n}_{i}\,{}^{A}t^{n}_{j}\,{}^{A}t^{b\bar m}_{m\bar n} - {}^{A}t^{n}_{i}\,{}^{A}t^{n}_{m}\,{}^{A}t^{b\bar m}_{j\bar n} + {}^{A}t^{n}_{i}\,{}^{A}t^{\bar m}_{\bar n}\,{}^{A}t^{bn}_{mj} + {}^{A}t^{n}_{i}\,{}^{A}t^{b}_{m}\,{}^{A}t^{n}_{j}\,{}^{A}t^{\bar m}_{\bar n} \\
&+ {}^{A}t^{\bar b}_{\bar j}\,{}^{A}t^{n\bar m}_{m\bar i} + {}^{A}t^{\bar b}_{\bar j}\,{}^{A}t^{n}_{m}\,{}^{A}t^{\bar m}_{\bar i} - {}^{A}t^{b}_{j}\,{}^{A}t^{n\bar m}_{m\bar i} - {}^{A}t^{b}_{j}\,{}^{A}t^{n}_{m}\,{}^{A}t^{\bar m}_{\bar i}] \\
&+ \delta(m,i)\,[+ {}^{A}t^{a}_{m}\,{}^{A}t^{b}_{m}\,{}^{A}t^{n\bar m}_{j\bar n} + {}^{A}t^{a}_{m}\,{}^{A}t^{n}_{j}\,{}^{A}t^{b\bar m}_{m\bar n} - {}^{A}t^{a}_{m}\,{}^{A}t^{n}_{m}\,{}^{A}t^{b\bar m}_{j\bar n} + {}^{A}t^{a}_{m}\,{}^{A}t^{\bar m}_{\bar n}\,{}^{A}t^{bn}_{mj} + {}^{A}t^{a}_{m}\,{}^{A}t^{b}_{m}\,{}^{A}t^{n}_{j}\,{}^{A}t^{\bar m}_{\bar n} \\
&- {}^{A}t^{\bar b}_{\bar j}\,{}^{A}t^{n\bar a}_{m\bar n} - {}^{A}t^{\bar b}_{\bar j}\,{}^{A}t^{\bar a}_{\bar n}\,{}^{A}t^{n}_{m} + {}^{A}t^{b}_{j}\,{}^{A}t^{n\bar a}_{m\bar n} + {}^{A}t^{b}_{j}\,{}^{A}t^{\bar a}_{\bar n}\,{}^{A}t^{n}_{m}] \\
&+ \delta(\bar n,\bar j)\,\delta(\bar m,\bar b)\,[- {}^{A}t^{a}_{i}\,{}^{A}t^{\bar m}_{\bar n} + {}^{A}t^{\bar m}_{\bar n}\,{}^{A}t^{\bar a}_{\bar n}\,{}^{A}t^{n\bar m}_{m\bar i} + {}^{A}t^{\bar m}_{\bar n}\,{}^{A}t^{n}_{m}\,{}^{A}t^{\bar a\bar m}_{\bar n\bar i} + {}^{A}t^{\bar m}_{\bar n}\,{}^{A}t^{\bar m}_{\bar i}\,{}^{A}t^{n\bar a}_{m\bar n} - {}^{A}t^{\bar m}_{\bar n}\,{}^{A}t^{\bar m}_{\bar n}\,{}^{A}t^{n\bar a}_{m\bar i} \\
&+ {}^{A}t^{\bar m}_{\bar n}\,{}^{A}t^{\bar a}_{\bar n}\,{}^{A}t^{n}_{m}\,{}^{A}t^{\bar m}_{\bar i} + {}^{A}t^{\bar a}_{\bar i}\,{}^{A}t^{\bar m}_{\bar n}] \\
&+ \delta(\bar m,\bar b)\,\delta(n,a)\,[+ {}^{A}t^{n}_{i}\,{}^{A}t^{n\bar m}_{j\bar n} + {}^{A}t^{n}_{i}\,{}^{A}t^{n}_{j}\,{}^{A}t^{\bar m}_{\bar n}] \\
&+ \delta(\bar n,\bar j)\,\delta(n,a)\,[- {}^{A}t^{n}_{i}\,{}^{A}t^{b\bar m}_{m\bar n} - {}^{A}t^{n}_{i}\,{}^{A}t^{b}_{m}\,{}^{A}t^{\bar m}_{\bar n} + {}^{A}t^{\bar b}_{\bar n}\,{}^{A}t^{n\bar m}_{m\bar i} + {}^{A}t^{\bar b}_{\bar n}\,{}^{A}t^{n}_{m}\,{}^{A}t^{\bar m}_{\bar i}] \\
&+ \delta(m,i)\,\delta(\bar m,\bar b)\,[+ {}^{A}t^{a}_{m}\,{}^{A}t^{n\bar m}_{j\bar n} + {}^{A}t^{a}_{m}\,{}^{A}t^{n}_{j}\,{}^{A}t^{\bar m}_{\bar n} - {}^{A}t^{\bar m}_{\bar j}\,{}^{A}t^{n\bar a}_{m\bar n} - {}^{A}t^{\bar m}_{\bar j}\,{}^{A}t^{\bar a}_{\bar n}\,{}^{A}t^{n}_{m}] \\
&+ \delta(m,i)\,\delta(\bar n,\bar j)\,[- {}^{A}t^{a}_{m}\,{}^{A}t^{b\bar m}_{m\bar n} - {}^{A}t^{a}_{m}\,{}^{A}t^{b}_{m}\,{}^{A}t^{\bar m}_{\bar n}] \\
&+ \delta(m,i)\,\delta(n,a)\,[+ {}^{A}t^{n}_{m}\,{}^{A}t^{b}_{m}\,{}^{A}t^{n\bar m}_{j\bar n} + {}^{A}t^{n}_{m}\,{}^{A}t^{n}_{j}\,{}^{A}t^{b\bar m}_{m\bar n} - {}^{A}t^{n}_{m}\,{}^{A}t^{n}_{m}\,{}^{A}t^{b\bar m}_{j\bar n} + {}^{A}t^{n}_{m}\,{}^{A}t^{\bar m}_{\bar n}\,{}^{A}t^{bn}_{mj} + {}^{A}t^{n}_{m}\,{}^{A}t^{b}_{m}\,{}^{A}t^{n}_{j}\,{}^{A}t^{\bar m}_{\bar n} \\
&- {}^{A}t^{\bar b}_{\bar j}\,{}^{A}t^{n}_{m} + {}^{A}t^{b}_{j}\,{}^{A}t^{n}_{m}] \\
&+ \delta(n,a)\,\delta(\bar m,\bar b)\,[+ {}^{A}t^{\bar m}_{\bar j}\,{}^{A}t^{n\bar m}_{m\bar i} + {}^{A}t^{\bar m}_{\bar j}\,{}^{A}t^{n}_{m}\,{}^{A}t^{\bar m}_{\bar i}] \\
&+ \delta(\bar n,\bar j)\,\delta(m,i)\,[- {}^{A}t^{\bar b}_{\bar n}\,{}^{A}t^{n\bar a}_{m\bar n} - {}^{A}t^{\bar b}_{\bar n}\,{}^{A}t^{\bar a}_{\bar n}\,{}^{A}t^{n}_{m}] \\
&+ \delta(\bar n,\bar j)\,\delta(n,a)\,\delta(\bar m,\bar b)\,[- {}^{A}t^{n}_{i}\,{}^{A}t^{\bar m}_{\bar n}] \\
&+ \delta(m,i)\,\delta(\bar m,\bar b)\,\delta(\bar n,\bar j)\,[- {}^{A}t^{a}_{m}\,{}^{A}t^{\bar m}_{\bar n}] \\
&+ \delta(m,i)\,\delta(n,a)\,\delta(\bar m,\bar b)\,[+ {}^{A}t^{n}_{m}\,{}^{A}t^{n\bar m}_{j\bar n} + {}^{A}t^{n}_{m}\,{}^{A}t^{n}_{j}\,{}^{A}t^{\bar m}_{\bar n}] \\
&+ \delta(m,i)\,\delta(n,a)\,\delta(\bar n,\bar j)\,[- {}^{A}t^{n}_{m}\,{}^{A}t^{b\bar m}_{m\bar n} - {}^{A}t^{n}_{m}\,{}^{A}t^{b}_{m}\,{}^{A}t^{\bar m}_{\bar n}] \\
&+ \delta(m,i)\,\delta(\bar m,\bar b)\,\delta(n,a)\,[- {}^{A}t^{\bar m}_{\bar j}\,{}^{A}t^{n}_{m}] \\
&+ \delta(\bar n,\bar j)\,\delta(n,a)\,\delta(m,i)\,[- {}^{A}t^{\bar b}_{\bar n}\,{}^{A}t^{n}_{m}] \\
&+ \delta(\bar n,\bar j)\,\delta(\bar m,\bar b)\,\delta(n,a)\,[+ {}^{A}t^{\bar m}_{\bar n}\,{}^{A}t^{n\bar m}_{m\bar i} + {}^{A}t^{\bar m}_{\bar n}\,{}^{A}t^{n}_{m}\,{}^{A}t^{\bar m}_{\bar i}] \\
&+ \delta(\bar n,\bar j)\,\delta(\bar m,\bar b)\,\delta(m,i)\,[- {}^{A}t^{\bar m}_{\bar n}\,{}^{A}t^{n\bar a}_{m\bar n} - {}^{A}t^{\bar m}_{\bar n}\,{}^{A}t^{\bar a}_{\bar n}\,{}^{A}t^{n}_{m}] \\
&+ \delta(m,i)\,\delta(n,a)\,\delta(\bar m,\bar b)\,\delta(\bar n,\bar j)\,[- {}^{A}t^{n}_{m}\,{}^{A}t^{\bar m}_{\bar n}] \\
&+ \delta(\bar n,\bar j)\,\delta(\bar m,\bar b)\,\delta(n,a)\,\delta(m,i)\,[- {}^{A}t^{\bar m}_{\bar n}\,{}^{A}t^{n}_{m}]
\end{aligned} \tag{S62}$$

$$
\begin{aligned}
M^{\bar a b}_{i\bar j} =& [- {}^{A}t^{\bar a}_{\bar j}\, {}^{A}t^{\bar b}_{\bar n}\, {}^{A}t^{n\bar m}_{m\bar i} - {}^{A}t^{\bar a}_{\bar j}\, {}^{A}t^{n}_{m}\, {}^{A}t^{\bar b\bar m}_{\bar n\bar i} - {}^{A}t^{\bar a}_{\bar j}\, {}^{A}t^{\bar m}_{\bar i}\, {}^{A}t^{n\bar b}_{m\bar n} + {}^{A}t^{\bar a}_{\bar j}\, {}^{A}t^{\bar m}_{\bar n}\, {}^{A}t^{n\bar b}_{m\bar i} \\
& - {}^{A}t^{\bar a}_{\bar j}\, {}^{A}t^{\bar b}_{\bar n}\, {}^{A}t^{n}_{m}\, {}^{A}t^{\bar m}_{\bar i} - {}^{A}t^{b}_{i}\, {}^{A}t^{a}_{m}\, {}^{A}t^{n\bar m}_{j\bar n} - {}^{A}t^{b}_{i}\, {}^{A}t^{n}_{j}\, {}^{A}t^{a\bar m}_{m\bar n} + {}^{A}t^{b}_{i}\, {}^{A}t^{n}_{m}\, {}^{A}t^{a\bar m}_{j\bar n} - {}^{A}t^{b}_{i}\, {}^{A}t^{\bar m}_{\bar n}\, {}^{A}t^{an}_{mj} \\
& - {}^{A}t^{b}_{i}\, {}^{A}t^{a}_{m}\, {}^{A}t^{n}_{j}\, {}^{A}t^{\bar m}_{\bar n} + {}^{A}t^{a}_{j}\, {}^{A}t^{\bar b}_{\bar n}\, {}^{A}t^{n\bar m}_{m\bar i} + {}^{A}t^{a}_{j}\, {}^{A}t^{n}_{m}\, {}^{A}t^{\bar b\bar m}_{\bar n\bar i} + {}^{A}t^{a}_{j}\, {}^{A}t^{\bar m}_{\bar i}\, {}^{A}t^{n\bar b}_{m\bar n} - {}^{A}t^{a}_{j}\, {}^{A}t^{\bar m}_{\bar n}\, {}^{A}t^{n\bar b}_{m\bar i} \\
& + {}^{A}t^{a}_{j}\, {}^{A}t^{\bar b}_{\bar n}\, {}^{A}t^{n}_{m}\, {}^{A}t^{\bar m}_{\bar i} + {}^{A}t^{\bar b}_{\bar i}\, {}^{A}t^{a}_{m}\, {}^{A}t^{n\bar m}_{j\bar n} + {}^{A}t^{\bar b}_{\bar i}\, {}^{A}t^{n}_{j}\, {}^{A}t^{a\bar m}_{m\bar n} - {}^{A}t^{\bar b}_{\bar i}\, {}^{A}t^{n}_{m}\, {}^{A}t^{a\bar m}_{j\bar n} \\
& + {}^{A}t^{\bar b}_{\bar i}\, {}^{A}t^{\bar m}_{\bar n}\, {}^{A}t^{an}_{mj} + {}^{A}t^{\bar b}_{\bar i}\, {}^{A}t^{a}_{m}\, {}^{A}t^{n}_{j}\, {}^{A}t^{\bar m}_{\bar n}] \\
& + \delta(n,b)\, [- {}^{A}t^{\bar a}_{\bar j}\, {}^{A}t^{n\bar m}_{m\bar i} - {}^{A}t^{\bar a}_{\bar j}\, {}^{A}t^{n}_{m}\, {}^{A}t^{\bar m}_{\bar i} - {}^{A}t^{n}_{i}\, {}^{A}t^{a}_{m}\, {}^{A}t^{n\bar m}_{j\bar n} - {}^{A}t^{n}_{i}\, {}^{A}t^{n}_{j}\, {}^{A}t^{a\bar m}_{m\bar n} + {}^{A}t^{n}_{i}\, {}^{A}t^{n}_{m}\, {}^{A}t^{a\bar m}_{j\bar n} \\
& - {}^{A}t^{n}_{i}\, {}^{A}t^{\bar m}_{\bar n}\, {}^{A}t^{an}_{mj} - {}^{A}t^{n}_{i}\, {}^{A}t^{a}_{m}\, {}^{A}t^{n}_{j}\, {}^{A}t^{\bar m}_{\bar n} + {}^{A}t^{a}_{j}\, {}^{A}t^{n\bar m}_{m\bar i} + {}^{A}t^{a}_{j}\, {}^{A}t^{n}_{m}\, {}^{A}t^{\bar m}_{\bar i}] \\
& + \delta(m,i)\, [+ {}^{A}t^{\bar a}_{\bar j}\, {}^{A}t^{n\bar b}_{m\bar n} + {}^{A}t^{\bar a}_{\bar j}\, {}^{A}t^{\bar b}_{\bar n}\, {}^{A}t^{n}_{m} - {}^{A}t^{b}_{m}\, {}^{A}t^{a}_{m}\, {}^{A}t^{n\bar m}_{j\bar n} - {}^{A}t^{b}_{m}\, {}^{A}t^{n}_{j}\, {}^{A}t^{a\bar m}_{m\bar n} + {}^{A}t^{b}_{m}\, {}^{A}t^{n}_{m}\, {}^{A}t^{a\bar m}_{j\bar n} \\
& - {}^{A}t^{b}_{m}\, {}^{A}t^{\bar m}_{\bar n}\, {}^{A}t^{an}_{mj} - {}^{A}t^{b}_{m}\, {}^{A}t^{a}_{m}\, {}^{A}t^{n}_{j}\, {}^{A}t^{\bar m}_{\bar n} - {}^{A}t^{a}_{j}\, {}^{A}t^{n\bar b}_{m\bar n} - {}^{A}t^{a}_{j}\, {}^{A}t^{\bar b}_{\bar n}\, {}^{A}t^{n}_{m}] \\
& + \delta(\bar m,\bar a)\, [- {}^{A}t^{\bar m}_{\bar j}\, {}^{A}t^{\bar b}_{\bar n}\, {}^{A}t^{n\bar m}_{m\bar i} - {}^{A}t^{\bar m}_{\bar j}\, {}^{A}t^{n}_{m}\, {}^{A}t^{\bar b\bar m}_{\bar n\bar i} - {}^{A}t^{\bar m}_{\bar j}\, {}^{A}t^{\bar m}_{\bar i}\, {}^{A}t^{n\bar b}_{m\bar n} + {}^{A}t^{\bar m}_{\bar j}\, {}^{A}t^{\bar m}_{\bar n}\, {}^{A}t^{n\bar b}_{m\bar i} \\
& - {}^{A}t^{\bar m}_{\bar j}\, {}^{A}t^{\bar b}_{\bar n}\, {}^{A}t^{n}_{m}\, {}^{A}t^{\bar m}_{\bar i} - {}^{A}t^{b}_{i}\, {}^{A}t^{n\bar m}_{j\bar n} - {}^{A}t^{b}_{i}\, {}^{A}t^{n}_{j}\, {}^{A}t^{\bar m}_{\bar n} + {}^{A}t^{\bar b}_{\bar i}\, {}^{A}t^{n\bar m}_{j\bar n} + {}^{A}t^{\bar b}_{\bar i}\, {}^{A}t^{n}_{j}\, {}^{A}t^{\bar m}_{\bar n}] \\
& + \delta(\bar n,\bar j)\, [- {}^{A}t^{\bar a}_{\bar n}\, {}^{A}t^{\bar b}_{\bar n}\, {}^{A}t^{n\bar m}_{m\bar i} - {}^{A}t^{\bar a}_{\bar n}\, {}^{A}t^{n}_{m}\, {}^{A}t^{\bar b\bar m}_{\bar n\bar i} - {}^{A}t^{\bar a}_{\bar n}\, {}^{A}t^{\bar m}_{\bar i}\, {}^{A}t^{n\bar b}_{m\bar n} + {}^{A}t^{\bar a}_{\bar n}\, {}^{A}t^{\bar m}_{\bar n}\, {}^{A}t^{n\bar b}_{m\bar i} \\
& - {}^{A}t^{\bar a}_{\bar n}\, {}^{A}t^{\bar b}_{\bar n}\, {}^{A}t^{n}_{m}\, {}^{A}t^{\bar m}_{\bar i} + {}^{A}t^{b}_{i}\, {}^{A}t^{a\bar m}_{m\bar n} + {}^{A}t^{b}_{i}\, {}^{A}t^{a}_{m}\, {}^{A}t^{\bar m}_{\bar n} - {}^{A}t^{\bar b}_{\bar i}\, {}^{A}t^{a\bar m}_{m\bar n} - {}^{A}t^{\bar b}_{\bar i}\, {}^{A}t^{a}_{m}\, {}^{A}t^{\bar m}_{\bar n}] \\
& + \delta(m,i)\, \delta(n,b)\, [+ {}^{A}t^{\bar a}_{\bar j}\, {}^{A}t^{n}_{m} - {}^{A}t^{n}_{m}\, {}^{A}t^{a}_{m}\, {}^{A}t^{n\bar m}_{j\bar n} - {}^{A}t^{n}_{m}\, {}^{A}t^{n}_{j}\, {}^{A}t^{a\bar m}_{m\bar n} + {}^{A}t^{n}_{m}\, {}^{A}t^{n}_{m}\, {}^{A}t^{a\bar m}_{j\bar n} - {}^{A}t^{n}_{m}\, {}^{A}t^{\bar m}_{\bar n}\, {}^{A}t^{an}_{mj} - {}^{A}t^{n}_{m}\, {}^{A}t^{a}_{m}\, {}^{A}t^{n}_{j}\, {}^{A}t^{\bar m}_{\bar n} \\
& - {}^{A}t^{a}_{j}\, {}^{A}t^{n}_{m}] \\
& + \delta(n,b)\, \delta(\bar m,\bar a)\, [- {}^{A}t^{\bar m}_{\bar j}\, {}^{A}t^{n\bar m}_{m\bar i} - {}^{A}t^{\bar m}_{\bar j}\, {}^{A}t^{n}_{m}\, {}^{A}t^{\bar m}_{\bar i}] \\
& + \delta(m,i)\, \delta(\bar m,\bar a)\, [+ {}^{A}t^{\bar m}_{\bar j}\, {}^{A}t^{n\bar b}_{m\bar n} + {}^{A}t^{\bar m}_{\bar j}\, {}^{A}t^{\bar b}_{\bar n}\, {}^{A}t^{n}_{m} - {}^{A}t^{b}_{m}\, {}^{A}t^{n\bar m}_{j\bar n} - {}^{A}t^{b}_{m}\, {}^{A}t^{n}_{j}\, {}^{A}t^{\bar m}_{\bar n}] \\
& + \delta(\bar n,\bar j)\, \delta(n,b)\, [- {}^{A}t^{\bar a}_{\bar n}\, {}^{A}t^{n\bar m}_{m\bar i} - {}^{A}t^{\bar a}_{\bar n}\, {}^{A}t^{n}_{m}\, {}^{A}t^{\bar m}_{\bar i} + {}^{A}t^{n}_{i}\, {}^{A}t^{a\bar m}_{m\bar n} + {}^{A}t^{n}_{i}\, {}^{A}t^{a}_{m}\, {}^{A}t^{\bar m}_{\bar n}] \\
& + \delta(\bar n,\bar j)\, \delta(m,i)\, [+ {}^{A}t^{\bar a}_{\bar n}\, {}^{A}t^{n\bar b}_{m\bar n} + {}^{A}t^{\bar a}_{\bar n}\, {}^{A}t^{\bar b}_{\bar n}\, {}^{A}t^{n}_{m}] \\
& + \delta(\bar n,\bar j)\, \delta(\bar m,\bar a)\, [- {}^{A}t^{\bar m}_{\bar n}\, {}^{A}t^{\bar b}_{\bar n}\, {}^{A}t^{n\bar m}_{m\bar i} - {}^{A}t^{\bar m}_{\bar n}\, {}^{A}t^{n}_{m}\, {}^{A}t^{\bar b\bar m}_{\bar n\bar i} - {}^{A}t^{\bar m}_{\bar n}\, {}^{A}t^{\bar m}_{\bar i}\, {}^{A}t^{n\bar b}_{m\bar n} + {}^{A}t^{\bar m}_{\bar n}\, {}^{A}t^{\bar m}_{\bar n}\, {}^{A}t^{n\bar b}_{m\bar i} \\
& - {}^{A}t^{\bar m}_{\bar n}\, {}^{A}t^{\bar b}_{\bar n}\, {}^{A}t^{n}_{m}\, {}^{A}t^{\bar m}_{\bar i} + {}^{A}t^{b}_{i}\, {}^{A}t^{\bar m}_{\bar n} - {}^{A}t^{\bar b}_{\bar i}\, {}^{A}t^{\bar m}_{\bar n}] \\
& + \delta(\bar m,\bar a)\, \delta(n,b)\, [- {}^{A}t^{n}_{i}\, {}^{A}t^{n\bar m}_{j\bar n} - {}^{A}t^{n}_{i}\, {}^{A}t^{n}_{j}\, {}^{A}t^{\bar m}_{\bar n}] \\
& + \delta(m,i)\, \delta(\bar n,\bar j)\, [+ {}^{A}t^{b}_{m}\, {}^{A}t^{a\bar m}_{m\bar n} + {}^{A}t^{b}_{m}\, {}^{A}t^{a}_{m}\, {}^{A}t^{\bar m}_{\bar n}] \\
& + \delta(m,i)\, \delta(\bar m,\bar a)\, \delta(n,b)\, [+ {}^{A}t^{\bar m}_{\bar j}\, {}^{A}t^{n}_{m}] \\
& + \delta(\bar n,\bar j)\, \delta(n,b)\, \delta(m,i)\, [+ {}^{A}t^{\bar a}_{\bar n}\, {}^{A}t^{n}_{m}] \\
& + \delta(\bar n,\bar j)\, \delta(\bar m,\bar a)\, \delta(n,b)\, [- {}^{A}t^{\bar m}_{\bar n}\, {}^{A}t^{n\bar m}_{m\bar i} - {}^{A}t^{\bar m}_{\bar n}\, {}^{A}t^{n}_{m}\, {}^{A}t^{\bar m}_{\bar i}] \\
& + \delta(\bar n,\bar j)\, \delta(\bar m,\bar a)\, \delta(m,i)\, [+ {}^{A}t^{\bar m}_{\bar n}\, {}^{A}t^{n\bar b}_{m\bar n} + {}^{A}t^{\bar m}_{\bar n}\, {}^{A}t^{\bar b}_{\bar n}\, {}^{A}t^{n}_{m}] \\
& + \delta(\bar n,\bar j)\, \delta(n,b)\, \delta(\bar m,\bar a)\, [+ {}^{A}t^{n}_{i}\, {}^{A}t^{\bar m}_{\bar n}] \\
& + \delta(m,i)\, \delta(\bar m,\bar a)\, \delta(\bar n,\bar j)\, [+ {}^{A}t^{b}_{m}\, {}^{A}t^{\bar m}_{\bar n}] \\
& + \delta(m,i)\, \delta(n,b)\, \delta(\bar m,\bar a)\, [- {}^{A}t^{n}_{m}\, {}^{A}t^{n\bar m}_{j\bar n} - {}^{A}t^{n}_{m}\, {}^{A}t^{n}_{j}\, {}^{A}t^{\bar m}_{\bar n}] \\
& + \delta(m,i)\, \delta(n,b)\, \delta(\bar n,\bar j)\, [+ {}^{A}t^{n}_{m}\, {}^{A}t^{a\bar m}_{m\bar n} + {}^{A}t^{n}_{m}\, {}^{A}t^{a}_{m}\, {}^{A}t^{\bar m}_{\bar n}] \\
& + \delta(\bar n,\bar j)\, \delta(\bar m,\bar a)\, \delta(n,b)\, \delta(m,i)\, [+ {}^{A}t^{\bar m}_{\bar n}\, {}^{A}t^{n}_{m}] \\
& + \delta(m,i)\, \delta(n,b)\, \delta(\bar m,\bar a)\, \delta(\bar n,\bar j)\, [+ {}^{A}t^{n}_{m}\, {}^{A}t^{\bar m}_{\bar n}]
\end{aligned}
\tag{S63}
$$

$$
M^{\bar a\bar b}_{i\bar j} = 0 \tag{S64}
$$

$$
M^{ab}_{\bar i j} = 0 \tag{S65}
$$

$$
\begin{aligned}
M^{a\bar{b}}_{\bar{i}j} =&[- {}^{A}t^{a}_{j}\,{}^{A}t^{b}_{m}\,{}^{A}t^{n\bar{m}}_{i\bar{n}} - {}^{A}t^{a}_{j}\,{}^{A}t^{n}_{i}\,{}^{A}t^{b\bar{m}}_{m\bar{n}} + {}^{A}t^{a}_{j}\,{}^{A}t^{n}_{m}\,{}^{A}t^{b\bar{m}}_{i\bar{n}} - {}^{A}t^{a}_{j}\,{}^{A}t^{\bar{m}}_{\bar{n}}\,{}^{A}t^{bn}_{mi} - {}^{A}t^{a}_{j}\,{}^{A}t^{b}_{m}\,{}^{A}t^{n}_{i}\,{}^{A}t^{\bar{m}}_{\bar{n}} \\
&- {}^{A}t^{\bar{b}}_{\bar{i}}\,{}^{A}t^{\bar{a}}_{\bar{n}}\,{}^{A}t^{n\bar{m}}_{m\bar{j}} - {}^{A}t^{\bar{b}}_{\bar{i}}\,{}^{A}t^{n}_{m}\,{}^{A}t^{\bar{a}\bar{m}}_{\bar{n}\bar{j}} - {}^{A}t^{\bar{b}}_{\bar{i}}\,{}^{A}t^{\bar{m}}_{\bar{j}}\,{}^{A}t^{n\bar{a}}_{m\bar{n}} + {}^{A}t^{\bar{b}}_{\bar{i}}\,{}^{A}t^{\bar{m}}_{\bar{n}}\,{}^{A}t^{n\bar{a}}_{m\bar{j}} \\
&- {}^{A}t^{\bar{b}}_{\bar{i}}\,{}^{A}t^{\bar{a}}_{\bar{n}}\,{}^{A}t^{n}_{m}\,{}^{A}t^{\bar{m}}_{\bar{j}} + {}^{A}t^{\bar{a}}_{\bar{j}}\,{}^{A}t^{b}_{m}\,{}^{A}t^{n\bar{m}}_{i\bar{n}} + {}^{A}t^{\bar{a}}_{\bar{j}}\,{}^{A}t^{n}_{i}\,{}^{A}t^{b\bar{m}}_{m\bar{n}} - {}^{A}t^{\bar{a}}_{\bar{j}}\,{}^{A}t^{n}_{m}\,{}^{A}t^{b\bar{m}}_{i\bar{n}} \\
&+ {}^{A}t^{\bar{a}}_{\bar{j}}\,{}^{A}t^{\bar{m}}_{\bar{n}}\,{}^{A}t^{bn}_{mi} + {}^{A}t^{\bar{a}}_{\bar{j}}\,{}^{A}t^{b}_{m}\,{}^{A}t^{n}_{i}\,{}^{A}t^{\bar{m}}_{\bar{n}} + {}^{A}t^{b}_{i}\,{}^{A}t^{\bar{a}}_{\bar{n}}\,{}^{A}t^{n\bar{m}}_{m\bar{j}} + {}^{A}t^{b}_{i}\,{}^{A}t^{n}_{m}\,{}^{A}t^{\bar{a}\bar{m}}_{\bar{n}\bar{j}} \\
&+ {}^{A}t^{b}_{i}\,{}^{A}t^{\bar{m}}_{\bar{j}}\,{}^{A}t^{n\bar{a}}_{m\bar{n}} - {}^{A}t^{b}_{i}\,{}^{A}t^{\bar{m}}_{\bar{n}}\,{}^{A}t^{n\bar{a}}_{m\bar{j}} + {}^{A}t^{b}_{i}\,{}^{A}t^{\bar{a}}_{\bar{n}}\,{}^{A}t^{n}_{m}\,{}^{A}t^{\bar{m}}_{\bar{j}}] \\
&+ \delta(\bar{m},\bar{b})\,[- {}^{A}t^{a}_{j}\,{}^{A}t^{n\bar{m}}_{i\bar{n}} - {}^{A}t^{a}_{j}\,{}^{A}t^{n}_{i}\,{}^{A}t^{\bar{m}}_{\bar{n}} - {}^{A}t^{\bar{m}}_{\bar{i}}\,{}^{A}t^{\bar{a}}_{\bar{n}}\,{}^{A}t^{n\bar{m}}_{m\bar{j}} - {}^{A}t^{\bar{m}}_{\bar{i}}\,{}^{A}t^{n}_{m}\,{}^{A}t^{\bar{a}\bar{m}}_{\bar{n}\bar{j}} - {}^{A}t^{\bar{m}}_{\bar{i}}\,{}^{A}t^{\bar{m}}_{\bar{j}}\,{}^{A}t^{n\bar{a}}_{m\bar{n}} \\
&+ {}^{A}t^{\bar{m}}_{\bar{i}}\,{}^{A}t^{\bar{m}}_{\bar{n}}\,{}^{A}t^{n\bar{a}}_{m\bar{j}} - {}^{A}t^{\bar{m}}_{\bar{i}}\,{}^{A}t^{\bar{a}}_{\bar{n}}\,{}^{A}t^{n}_{m}\,{}^{A}t^{\bar{m}}_{\bar{j}} + {}^{A}t^{\bar{a}}_{\bar{j}}\,{}^{A}t^{n\bar{m}}_{i\bar{n}} + {}^{A}t^{\bar{a}}_{\bar{j}}\,{}^{A}t^{n}_{i}\,{}^{A}t^{\bar{m}}_{\bar{n}}] \\
&+ \delta(\bar{n},\bar{i})\,[+ {}^{A}t^{a}_{j}\,{}^{A}t^{b\bar{m}}_{m\bar{n}} + {}^{A}t^{a}_{j}\,{}^{A}t^{b}_{m}\,{}^{A}t^{\bar{m}}_{\bar{n}} - {}^{A}t^{\bar{b}}_{\bar{n}}\,{}^{A}t^{\bar{a}}_{\bar{n}}\,{}^{A}t^{n\bar{m}}_{m\bar{j}} - {}^{A}t^{\bar{b}}_{\bar{n}}\,{}^{A}t^{n}_{m}\,{}^{A}t^{\bar{a}\bar{m}}_{\bar{n}\bar{j}} - {}^{A}t^{\bar{b}}_{\bar{n}}\,{}^{A}t^{\bar{m}}_{\bar{j}}\,{}^{A}t^{n\bar{a}}_{m\bar{n}} \\
&+ {}^{A}t^{\bar{b}}_{\bar{n}}\,{}^{A}t^{\bar{m}}_{\bar{n}}\,{}^{A}t^{n\bar{a}}_{m\bar{j}} - {}^{A}t^{\bar{b}}_{\bar{n}}\,{}^{A}t^{\bar{a}}_{\bar{n}}\,{}^{A}t^{n}_{m}\,{}^{A}t^{\bar{m}}_{\bar{j}} - {}^{A}t^{\bar{a}}_{\bar{j}}\,{}^{A}t^{b\bar{m}}_{m\bar{n}} - {}^{A}t^{\bar{a}}_{\bar{j}}\,{}^{A}t^{b}_{m}\,{}^{A}t^{\bar{m}}_{\bar{n}}] \\
&+ \delta(n,a)\,[- {}^{A}t^{n}_{j}\,{}^{A}t^{b}_{m}\,{}^{A}t^{n\bar{m}}_{i\bar{n}} - {}^{A}t^{n}_{j}\,{}^{A}t^{n}_{i}\,{}^{A}t^{b\bar{m}}_{m\bar{n}} + {}^{A}t^{n}_{j}\,{}^{A}t^{n}_{m}\,{}^{A}t^{b\bar{m}}_{i\bar{n}} - {}^{A}t^{n}_{j}\,{}^{A}t^{\bar{m}}_{\bar{n}}\,{}^{A}t^{bn}_{mi} - {}^{A}t^{n}_{j}\,{}^{A}t^{b}_{m}\,{}^{A}t^{n}_{i}\,{}^{A}t^{\bar{m}}_{\bar{n}} \\
&- {}^{A}t^{\bar{b}}_{\bar{i}}\,{}^{A}t^{n\bar{m}}_{m\bar{j}} - {}^{A}t^{\bar{b}}_{\bar{i}}\,{}^{A}t^{n}_{m}\,{}^{A}t^{\bar{m}}_{\bar{j}} + {}^{A}t^{b}_{i}\,{}^{A}t^{n\bar{m}}_{m\bar{j}} + {}^{A}t^{b}_{i}\,{}^{A}t^{n}_{m}\,{}^{A}t^{\bar{m}}_{\bar{j}}] \\
&+ \delta(m,j)\,[- {}^{A}t^{a}_{m}\,{}^{A}t^{b}_{m}\,{}^{A}t^{n\bar{m}}_{i\bar{n}} - {}^{A}t^{a}_{m}\,{}^{A}t^{n}_{i}\,{}^{A}t^{b\bar{m}}_{m\bar{n}} + {}^{A}t^{a}_{m}\,{}^{A}t^{n}_{m}\,{}^{A}t^{b\bar{m}}_{i\bar{n}} - {}^{A}t^{a}_{m}\,{}^{A}t^{\bar{m}}_{\bar{n}}\,{}^{A}t^{bn}_{mi} - {}^{A}t^{a}_{m}\,{}^{A}t^{b}_{m}\,{}^{A}t^{n}_{i}\,{}^{A}t^{\bar{m}}_{\bar{n}} \\
&+ {}^{A}t^{\bar{b}}_{\bar{i}}\,{}^{A}t^{n\bar{a}}_{m\bar{n}} + {}^{A}t^{\bar{b}}_{\bar{i}}\,{}^{A}t^{\bar{a}}_{\bar{n}}\,{}^{A}t^{n}_{m} - {}^{A}t^{b}_{i}\,{}^{A}t^{n\bar{a}}_{m\bar{n}} - {}^{A}t^{b}_{i}\,{}^{A}t^{\bar{a}}_{\bar{n}}\,{}^{A}t^{n}_{m}] \\
&+ \delta(\bar{n},\bar{i})\,\delta(\bar{m},\bar{b})\,[+ {}^{A}t^{a}_{j}\,{}^{A}t^{\bar{m}}_{\bar{n}} - {}^{A}t^{\bar{m}}_{\bar{n}}\,{}^{A}t^{\bar{a}}_{\bar{n}}\,{}^{A}t^{n\bar{m}}_{m\bar{j}} - {}^{A}t^{\bar{m}}_{\bar{n}}\,{}^{A}t^{n}_{m}\,{}^{A}t^{\bar{a}\bar{m}}_{\bar{n}\bar{j}} - {}^{A}t^{\bar{m}}_{\bar{n}}\,{}^{A}t^{\bar{m}}_{\bar{j}}\,{}^{A}t^{n\bar{a}}_{m\bar{n}} + {}^{A}t^{\bar{m}}_{\bar{n}}\,{}^{A}t^{\bar{m}}_{\bar{n}}\,{}^{A}t^{n\bar{a}}_{m\bar{j}} \\
&- {}^{A}t^{\bar{m}}_{\bar{n}}\,{}^{A}t^{\bar{a}}_{\bar{n}}\,{}^{A}t^{n}_{m}\,{}^{A}t^{\bar{m}}_{\bar{j}} - {}^{A}t^{\bar{a}}_{\bar{j}}\,{}^{A}t^{\bar{m}}_{\bar{n}}] \\
&+ \delta(\bar{m},\bar{b})\,\delta(n,a)\,[- {}^{A}t^{n}_{j}\,{}^{A}t^{n\bar{m}}_{i\bar{n}} - {}^{A}t^{n}_{j}\,{}^{A}t^{n}_{i}\,{}^{A}t^{\bar{m}}_{\bar{n}}] \\
&+ \delta(\bar{n},\bar{i})\,\delta(n,a)\,[+ {}^{A}t^{n}_{j}\,{}^{A}t^{b\bar{m}}_{m\bar{n}} + {}^{A}t^{n}_{j}\,{}^{A}t^{b}_{m}\,{}^{A}t^{\bar{m}}_{\bar{n}} - {}^{A}t^{\bar{b}}_{\bar{n}}\,{}^{A}t^{n\bar{m}}_{m\bar{j}} - {}^{A}t^{\bar{b}}_{\bar{n}}\,{}^{A}t^{n}_{m}\,{}^{A}t^{\bar{m}}_{\bar{j}}] \\
&+ \delta(m,j)\,\delta(\bar{m},\bar{b})\,[- {}^{A}t^{a}_{m}\,{}^{A}t^{n\bar{m}}_{i\bar{n}} - {}^{A}t^{a}_{m}\,{}^{A}t^{n}_{i}\,{}^{A}t^{\bar{m}}_{\bar{n}} + {}^{A}t^{\bar{m}}_{\bar{i}}\,{}^{A}t^{n\bar{a}}_{m\bar{n}} + {}^{A}t^{\bar{m}}_{\bar{i}}\,{}^{A}t^{\bar{a}}_{\bar{n}}\,{}^{A}t^{n}_{m}] \\
&+ \delta(m,j)\,\delta(\bar{n},\bar{i})\,[+ {}^{A}t^{a}_{m}\,{}^{A}t^{b\bar{m}}_{m\bar{n}} + {}^{A}t^{a}_{m}\,{}^{A}t^{b}_{m}\,{}^{A}t^{\bar{m}}_{\bar{n}}] \\
&+ \delta(m,j)\,\delta(n,a)\,[- {}^{A}t^{n}_{m}\,{}^{A}t^{b}_{m}\,{}^{A}t^{n\bar{m}}_{i\bar{n}} - {}^{A}t^{n}_{m}\,{}^{A}t^{n}_{i}\,{}^{A}t^{b\bar{m}}_{m\bar{n}} + {}^{A}t^{n}_{m}\,{}^{A}t^{n}_{m}\,{}^{A}t^{b\bar{m}}_{i\bar{n}} - {}^{A}t^{n}_{m}\,{}^{A}t^{\bar{m}}_{\bar{n}}\,{}^{A}t^{bn}_{mi} - {}^{A}t^{n}_{m}\,{}^{A}t^{b}_{m}\,{}^{A}t^{n}_{i}\,{}^{A}t^{\bar{m}}_{\bar{n}} \\
&+ {}^{A}t^{\bar{b}}_{\bar{i}}\,{}^{A}t^{n}_{m} - {}^{A}t^{b}_{i}\,{}^{A}t^{n}_{m}] \\
&+ \delta(n,a)\,\delta(\bar{m},\bar{b})\,[- {}^{A}t^{\bar{m}}_{\bar{i}}\,{}^{A}t^{n\bar{m}}_{m\bar{j}} - {}^{A}t^{\bar{m}}_{\bar{i}}\,{}^{A}t^{n}_{m}\,{}^{A}t^{\bar{m}}_{\bar{j}}] \\
&+ \delta(\bar{n},\bar{i})\,\delta(m,j)\,[+ {}^{A}t^{\bar{b}}_{\bar{n}}\,{}^{A}t^{n\bar{a}}_{m\bar{n}} + {}^{A}t^{\bar{b}}_{\bar{n}}\,{}^{A}t^{\bar{a}}_{\bar{n}}\,{}^{A}t^{n}_{m}] \\
&+ \delta(\bar{n},\bar{i})\,\delta(n,a)\,\delta(\bar{m},\bar{b})\,[+ {}^{A}t^{n}_{j}\,{}^{A}t^{\bar{m}}_{\bar{n}}] \\
&+ \delta(m,j)\,\delta(\bar{m},\bar{b})\,\delta(\bar{n},\bar{i})\,[+ {}^{A}t^{a}_{m}\,{}^{A}t^{\bar{m}}_{\bar{n}}] \\
&+ \delta(m,j)\,\delta(n,a)\,\delta(\bar{m},\bar{b})\,[- {}^{A}t^{n}_{m}\,{}^{A}t^{n\bar{m}}_{i\bar{n}} - {}^{A}t^{n}_{m}\,{}^{A}t^{n}_{i}\,{}^{A}t^{\bar{m}}_{\bar{n}}] \\
&+ \delta(m,j)\,\delta(n,a)\,\delta(\bar{n},\bar{i})\,[+ {}^{A}t^{n}_{m}\,{}^{A}t^{b\bar{m}}_{m\bar{n}} + {}^{A}t^{n}_{m}\,{}^{A}t^{b}_{m}\,{}^{A}t^{\bar{m}}_{\bar{n}}] \\
&+ \delta(m,j)\,\delta(\bar{m},\bar{b})\,\delta(n,a)\,[+ {}^{A}t^{\bar{m}}_{\bar{i}}\,{}^{A}t^{n}_{m}] \\
&+ \delta(\bar{n},\bar{i})\,\delta(n,a)\,\delta(m,j)\,[+ {}^{A}t^{\bar{b}}_{\bar{n}}\,{}^{A}t^{n}_{m}] \\
&+ \delta(\bar{n},\bar{i})\,\delta(\bar{m},\bar{b})\,\delta(n,a)\,[- {}^{A}t^{\bar{m}}_{\bar{n}}\,{}^{A}t^{n\bar{m}}_{m\bar{j}} - {}^{A}t^{\bar{m}}_{\bar{n}}\,{}^{A}t^{n}_{m}\,{}^{A}t^{\bar{m}}_{\bar{j}}] \\
&+ \delta(\bar{n},\bar{i})\,\delta(\bar{m},\bar{b})\,\delta(m,j)\,[+ {}^{A}t^{\bar{m}}_{\bar{n}}\,{}^{A}t^{n\bar{a}}_{m\bar{n}} + {}^{A}t^{\bar{m}}_{\bar{n}}\,{}^{A}t^{\bar{a}}_{\bar{n}}\,{}^{A}t^{n}_{m}] \\
&+ \delta(m,j)\,\delta(n,a)\,\delta(\bar{m},\bar{b})\,\delta(\bar{n},\bar{i})\,[+ {}^{A}t^{n}_{m}\,{}^{A}t^{\bar{m}}_{\bar{n}}] \\
&+ \delta(\bar{n},\bar{i})\,\delta(\bar{m},\bar{b})\,\delta(n,a)\,\delta(m,j)\,[+ {}^{A}t^{\bar{m}}_{\bar{n}}\,{}^{A}t^{n}_{m}]
\end{aligned}
\tag{S66}
$$

$$
\begin{aligned}
M^{\bar{a}b}_{\bar{i}j} =&[+ {}^{A}t^{\bar{a}}_{\bar{i}}\, {}^{A}t^{\bar{b}}_{\bar{n}}\, {}^{A}t^{n\bar{m}}_{m\bar{j}} + {}^{A}t^{\bar{a}}_{\bar{i}}\, {}^{A}t^{n}_{m}\, {}^{A}t^{\bar{b}\bar{m}}_{\bar{n}\bar{j}} + {}^{A}t^{\bar{a}}_{\bar{i}}\, {}^{A}t^{\bar{m}}_{\bar{j}}\, {}^{A}t^{n\bar{b}}_{m\bar{n}} - {}^{A}t^{\bar{a}}_{\bar{i}}\, {}^{A}t^{\bar{m}}_{\bar{n}}\, {}^{A}t^{n\bar{b}}_{m\bar{j}} \\
&+ {}^{A}t^{\bar{a}}_{\bar{i}}\, {}^{A}t^{\bar{b}}_{\bar{n}}\, {}^{A}t^{n}_{m}\, {}^{A}t^{\bar{m}}_{\bar{j}} + {}^{A}t^{b}_{j}\, {}^{A}t^{a}_{m}\, {}^{A}t^{n\bar{m}}_{i\bar{n}} + {}^{A}t^{b}_{j}\, {}^{A}t^{n}_{i}\, {}^{A}t^{a\bar{m}}_{m\bar{n}} - {}^{A}t^{b}_{j}\, {}^{A}t^{n}_{m}\, {}^{A}t^{a\bar{m}}_{i\bar{n}} + {}^{A}t^{b}_{j}\, {}^{A}t^{\bar{m}}_{\bar{n}}\, {}^{A}t^{an}_{mi} \\
&+ {}^{A}t^{b}_{j}\, {}^{A}t^{a}_{m}\, {}^{A}t^{n}_{i}\, {}^{A}t^{\bar{m}}_{\bar{n}} - {}^{A}t^{a}_{i}\, {}^{A}t^{\bar{b}}_{\bar{n}}\, {}^{A}t^{n\bar{m}}_{m\bar{j}} - {}^{A}t^{a}_{i}\, {}^{A}t^{n}_{m}\, {}^{A}t^{\bar{b}\bar{m}}_{\bar{n}\bar{j}} - {}^{A}t^{a}_{i}\, {}^{A}t^{\bar{m}}_{\bar{j}}\, {}^{A}t^{n\bar{b}}_{m\bar{n}} + {}^{A}t^{a}_{i}\, {}^{A}t^{\bar{m}}_{\bar{n}}\, {}^{A}t^{n\bar{b}}_{m\bar{j}} \\
&- {}^{A}t^{a}_{i}\, {}^{A}t^{\bar{b}}_{\bar{n}}\, {}^{A}t^{n}_{m}\, {}^{A}t^{\bar{m}}_{\bar{j}} - {}^{A}t^{\bar{b}}_{\bar{j}}\, {}^{A}t^{a}_{m}\, {}^{A}t^{n\bar{m}}_{i\bar{n}} - {}^{A}t^{\bar{b}}_{\bar{j}}\, {}^{A}t^{n}_{i}\, {}^{A}t^{a\bar{m}}_{m\bar{n}} + {}^{A}t^{\bar{b}}_{\bar{j}}\, {}^{A}t^{n}_{m}\, {}^{A}t^{a\bar{m}}_{i\bar{n}} \\
&- {}^{A}t^{\bar{b}}_{\bar{j}}\, {}^{A}t^{\bar{m}}_{\bar{n}}\, {}^{A}t^{an}_{mi} - {}^{A}t^{\bar{b}}_{\bar{j}}\, {}^{A}t^{a}_{m}\, {}^{A}t^{n}_{i}\, {}^{A}t^{\bar{m}}_{\bar{n}}] \\
&+ \delta(n,b)\, [+ {}^{A}t^{\bar{a}}_{\bar{i}}\, {}^{A}t^{n\bar{m}}_{m\bar{j}} + {}^{A}t^{\bar{a}}_{\bar{i}}\, {}^{A}t^{n}_{m}\, {}^{A}t^{\bar{m}}_{\bar{j}} + {}^{A}t^{n}_{j}\, {}^{A}t^{a}_{m}\, {}^{A}t^{n\bar{m}}_{i\bar{n}} + {}^{A}t^{n}_{j}\, {}^{A}t^{n}_{i}\, {}^{A}t^{a\bar{m}}_{m\bar{n}} - {}^{A}t^{n}_{j}\, {}^{A}t^{n}_{m}\, {}^{A}t^{a\bar{m}}_{i\bar{n}} \\
&+ {}^{A}t^{n}_{j}\, {}^{A}t^{\bar{m}}_{\bar{n}}\, {}^{A}t^{an}_{mi} + {}^{A}t^{n}_{j}\, {}^{A}t^{a}_{m}\, {}^{A}t^{n}_{i}\, {}^{A}t^{\bar{m}}_{\bar{n}} - {}^{A}t^{a}_{i}\, {}^{A}t^{n\bar{m}}_{m\bar{j}} - {}^{A}t^{a}_{i}\, {}^{A}t^{n}_{m}\, {}^{A}t^{\bar{m}}_{\bar{j}}] \\
&+ \delta(m,j)\, [- {}^{A}t^{\bar{a}}_{\bar{i}}\, {}^{A}t^{n\bar{b}}_{m\bar{n}} - {}^{A}t^{\bar{a}}_{\bar{i}}\, {}^{A}t^{\bar{b}}_{\bar{n}}\, {}^{A}t^{n}_{m} + {}^{A}t^{b}_{m}\, {}^{A}t^{a}_{m}\, {}^{A}t^{n\bar{m}}_{i\bar{n}} + {}^{A}t^{b}_{m}\, {}^{A}t^{n}_{i}\, {}^{A}t^{a\bar{m}}_{m\bar{n}} - {}^{A}t^{b}_{m}\, {}^{A}t^{n}_{m}\, {}^{A}t^{a\bar{m}}_{i\bar{n}} \\
&+ {}^{A}t^{b}_{m}\, {}^{A}t^{\bar{m}}_{\bar{n}}\, {}^{A}t^{an}_{mi} + {}^{A}t^{b}_{m}\, {}^{A}t^{a}_{m}\, {}^{A}t^{n}_{i}\, {}^{A}t^{\bar{m}}_{\bar{n}} + {}^{A}t^{a}_{i}\, {}^{A}t^{n\bar{b}}_{m\bar{n}} + {}^{A}t^{a}_{i}\, {}^{A}t^{\bar{b}}_{\bar{n}}\, {}^{A}t^{n}_{m}] \\
&+ \delta(\bar{m},\bar{a})\, [+ {}^{A}t^{\bar{m}}_{\bar{i}}\, {}^{A}t^{\bar{b}}_{\bar{n}}\, {}^{A}t^{n\bar{m}}_{m\bar{j}} + {}^{A}t^{\bar{m}}_{\bar{i}}\, {}^{A}t^{n}_{m}\, {}^{A}t^{\bar{b}\bar{m}}_{\bar{n}\bar{j}} + {}^{A}t^{\bar{m}}_{\bar{i}}\, {}^{A}t^{\bar{m}}_{\bar{j}}\, {}^{A}t^{n\bar{b}}_{m\bar{n}} - {}^{A}t^{\bar{m}}_{\bar{i}}\, {}^{A}t^{\bar{m}}_{\bar{n}}\, {}^{A}t^{n\bar{b}}_{m\bar{j}} \\
&+ {}^{A}t^{\bar{m}}_{\bar{i}}\, {}^{A}t^{\bar{b}}_{\bar{n}}\, {}^{A}t^{n}_{m}\, {}^{A}t^{\bar{m}}_{\bar{j}} + {}^{A}t^{b}_{j}\, {}^{A}t^{n\bar{m}}_{i\bar{n}} + {}^{A}t^{b}_{j}\, {}^{A}t^{n}_{i}\, {}^{A}t^{\bar{m}}_{\bar{n}} - {}^{A}t^{\bar{b}}_{\bar{j}}\, {}^{A}t^{n\bar{m}}_{i\bar{n}} - {}^{A}t^{\bar{b}}_{\bar{j}}\, {}^{A}t^{n}_{i}\, {}^{A}t^{\bar{m}}_{\bar{n}}] \\
&+ \delta(\bar{n},\bar{i})\, [+ {}^{A}t^{\bar{a}}_{\bar{n}}\, {}^{A}t^{\bar{b}}_{\bar{n}}\, {}^{A}t^{n\bar{m}}_{m\bar{j}} + {}^{A}t^{\bar{a}}_{\bar{n}}\, {}^{A}t^{n}_{m}\, {}^{A}t^{\bar{b}\bar{m}}_{\bar{n}\bar{j}} + {}^{A}t^{\bar{a}}_{\bar{n}}\, {}^{A}t^{\bar{m}}_{\bar{j}}\, {}^{A}t^{n\bar{b}}_{m\bar{n}} - {}^{A}t^{\bar{a}}_{\bar{n}}\, {}^{A}t^{\bar{m}}_{\bar{n}}\, {}^{A}t^{n\bar{b}}_{m\bar{j}} \\
&+ {}^{A}t^{\bar{a}}_{\bar{n}}\, {}^{A}t^{\bar{b}}_{\bar{n}}\, {}^{A}t^{n}_{m}\, {}^{A}t^{\bar{m}}_{\bar{j}} - {}^{A}t^{b}_{j}\, {}^{A}t^{a\bar{m}}_{m\bar{n}} - {}^{A}t^{b}_{j}\, {}^{A}t^{a}_{m}\, {}^{A}t^{\bar{m}}_{\bar{n}} + {}^{A}t^{\bar{b}}_{\bar{j}}\, {}^{A}t^{a\bar{m}}_{m\bar{n}} + {}^{A}t^{\bar{b}}_{\bar{j}}\, {}^{A}t^{a}_{m}\, {}^{A}t^{\bar{m}}_{\bar{n}}] \\
&+ \delta(m,j)\, \delta(n,b)\, [- {}^{A}t^{\bar{a}}_{\bar{i}}\, {}^{A}t^{n}_{m} + {}^{A}t^{n}_{m}\, {}^{A}t^{a}_{m}\, {}^{A}t^{n\bar{m}}_{i\bar{n}} + {}^{A}t^{n}_{m}\, {}^{A}t^{n}_{i}\, {}^{A}t^{a\bar{m}}_{m\bar{n}} - {}^{A}t^{n}_{m}\, {}^{A}t^{n}_{m}\, {}^{A}t^{a\bar{m}}_{i\bar{n}} + {}^{A}t^{n}_{m}\, {}^{A}t^{\bar{m}}_{\bar{n}}\, {}^{A}t^{an}_{mi} + {}^{A}t^{n}_{m}\, {}^{A}t^{a}_{m}\, {}^{A}t^{n}_{i}\, {}^{A}t^{\bar{m}}_{\bar{n}} \\
&+ {}^{A}t^{a}_{i}\, {}^{A}t^{n}_{m}] \\
&+ \delta(n,b)\, \delta(\bar{m},\bar{a})\, [+ {}^{A}t^{\bar{m}}_{\bar{i}}\, {}^{A}t^{n\bar{m}}_{m\bar{j}} + {}^{A}t^{\bar{m}}_{\bar{i}}\, {}^{A}t^{n}_{m}\, {}^{A}t^{\bar{m}}_{\bar{j}}] \\
&+ \delta(m,j)\, \delta(\bar{m},\bar{a})\, [- {}^{A}t^{\bar{m}}_{\bar{i}}\, {}^{A}t^{n\bar{b}}_{m\bar{n}} - {}^{A}t^{\bar{m}}_{\bar{i}}\, {}^{A}t^{\bar{b}}_{\bar{n}}\, {}^{A}t^{n}_{m} + {}^{A}t^{b}_{m}\, {}^{A}t^{n\bar{m}}_{i\bar{n}} + {}^{A}t^{b}_{m}\, {}^{A}t^{n}_{i}\, {}^{A}t^{\bar{m}}_{\bar{n}}] \\
&+ \delta(\bar{n},\bar{i})\, \delta(n,b)\, [+ {}^{A}t^{\bar{a}}_{\bar{n}}\, {}^{A}t^{n\bar{m}}_{m\bar{j}} + {}^{A}t^{\bar{a}}_{\bar{n}}\, {}^{A}t^{n}_{m}\, {}^{A}t^{\bar{m}}_{\bar{j}} - {}^{A}t^{n}_{j}\, {}^{A}t^{a\bar{m}}_{m\bar{n}} - {}^{A}t^{n}_{j}\, {}^{A}t^{a}_{m}\, {}^{A}t^{\bar{m}}_{\bar{n}}] \\
&+ \delta(\bar{n},\bar{i})\, \delta(m,j)\, [- {}^{A}t^{\bar{a}}_{\bar{n}}\, {}^{A}t^{n\bar{b}}_{m\bar{n}} - {}^{A}t^{\bar{a}}_{\bar{n}}\, {}^{A}t^{\bar{b}}_{\bar{n}}\, {}^{A}t^{n}_{m}] \\
&+ \delta(\bar{n},\bar{i})\, \delta(\bar{m},\bar{a})\, [+ {}^{A}t^{\bar{m}}_{\bar{n}}\, {}^{A}t^{\bar{b}}_{\bar{n}}\, {}^{A}t^{n\bar{m}}_{m\bar{j}} + {}^{A}t^{\bar{m}}_{\bar{n}}\, {}^{A}t^{n}_{m}\, {}^{A}t^{\bar{b}\bar{m}}_{\bar{n}\bar{j}} + {}^{A}t^{\bar{m}}_{\bar{n}}\, {}^{A}t^{\bar{m}}_{\bar{j}}\, {}^{A}t^{n\bar{b}}_{m\bar{n}} - {}^{A}t^{\bar{m}}_{\bar{n}}\, {}^{A}t^{\bar{m}}_{\bar{n}}\, {}^{A}t^{n\bar{b}}_{m\bar{j}} \\
&+ {}^{A}t^{\bar{m}}_{\bar{n}}\, {}^{A}t^{\bar{b}}_{\bar{n}}\, {}^{A}t^{n}_{m}\, {}^{A}t^{\bar{m}}_{\bar{j}} - {}^{A}t^{b}_{j}\, {}^{A}t^{\bar{m}}_{\bar{n}} + {}^{A}t^{\bar{b}}_{\bar{j}}\, {}^{A}t^{\bar{m}}_{\bar{n}}] \\
&+ \delta(\bar{m},\bar{a})\, \delta(n,b)\, [+ {}^{A}t^{n}_{j}\, {}^{A}t^{n\bar{m}}_{i\bar{n}} + {}^{A}t^{n}_{j}\, {}^{A}t^{n}_{i}\, {}^{A}t^{\bar{m}}_{\bar{n}}] \\
&+ \delta(m,j)\, \delta(\bar{n},\bar{i})\, [- {}^{A}t^{b}_{m}\, {}^{A}t^{a\bar{m}}_{m\bar{n}} - {}^{A}t^{b}_{m}\, {}^{A}t^{a}_{m}\, {}^{A}t^{\bar{m}}_{\bar{n}}] \\
&+ \delta(m,j)\, \delta(\bar{m},\bar{a})\, \delta(n,b)\, [- {}^{A}t^{\bar{m}}_{\bar{i}}\, {}^{A}t^{n}_{m}] \\
&+ \delta(\bar{n},\bar{i})\, \delta(n,b)\, \delta(m,j)\, [- {}^{A}t^{\bar{a}}_{\bar{n}}\, {}^{A}t^{n}_{m}] \\
&+ \delta(\bar{n},\bar{i})\, \delta(\bar{m},\bar{a})\, \delta(n,b)\, [+ {}^{A}t^{\bar{m}}_{\bar{n}}\, {}^{A}t^{n\bar{m}}_{m\bar{j}} + {}^{A}t^{\bar{m}}_{\bar{n}}\, {}^{A}t^{n}_{m}\, {}^{A}t^{\bar{m}}_{\bar{j}}] \\
&+ \delta(\bar{n},\bar{i})\, \delta(\bar{m},\bar{a})\, \delta(m,j)\, [- {}^{A}t^{\bar{m}}_{\bar{n}}\, {}^{A}t^{n\bar{b}}_{m\bar{n}} - {}^{A}t^{\bar{m}}_{\bar{n}}\, {}^{A}t^{\bar{b}}_{\bar{n}}\, {}^{A}t^{n}_{m}] \\
&+ \delta(\bar{n},\bar{i})\, \delta(n,b)\, \delta(\bar{m},\bar{a})\, [- {}^{A}t^{n}_{j}\, {}^{A}t^{\bar{m}}_{\bar{n}}] \\
&+ \delta(m,j)\, \delta(\bar{m},\bar{a})\, \delta(\bar{n},\bar{i})\, [- {}^{A}t^{b}_{m}\, {}^{A}t^{\bar{m}}_{\bar{n}}] \\
&+ \delta(m,j)\, \delta(n,b)\, \delta(\bar{m},\bar{a})\, [+ {}^{A}t^{n}_{m}\, {}^{A}t^{n\bar{m}}_{i\bar{n}} + {}^{A}t^{n}_{m}\, {}^{A}t^{n}_{i}\, {}^{A}t^{\bar{m}}_{\bar{n}}] \\
&+ \delta(m,j)\, \delta(n,b)\, \delta(\bar{n},\bar{i})\, [- {}^{A}t^{n}_{m}\, {}^{A}t^{a\bar{m}}_{m\bar{n}} - {}^{A}t^{n}_{m}\, {}^{A}t^{a}_{m}\, {}^{A}t^{\bar{m}}_{\bar{n}}] \\
&+ \delta(\bar{n},\bar{i})\, \delta(\bar{m},\bar{a})\, \delta(n,b)\, \delta(m,j)\, [- {}^{A}t^{\bar{m}}_{\bar{n}}\, {}^{A}t^{n}_{m}] \\
&+ \delta(m,j)\, \delta(n,b)\, \delta(\bar{m},\bar{a})\, \delta(\bar{n},\bar{i})\, [- {}^{A}t^{n}_{m}\, {}^{A}t^{\bar{m}}_{\bar{n}}]
\end{aligned}
\tag{S67}
$$

$$
M^{\bar{a}\bar{b}}_{\bar{i}j} = 0 \tag{S68}
$$

$$
M^{ab}_{\bar{i}\bar{j}} = 0 \tag{S69}
$$

$$
M^{a\bar{b}}_{\bar{i}\bar{j}} = 0 \tag{S70}
$$

$$M^{\bar{a}b}_{\bar{i}\bar{j}} = 0 \tag{S71}$$

$$
\begin{aligned}
M^{\bar{a}\bar{b}}_{\bar{i}\bar{j}} =\Big[&+ {}^{A}t^{\bar{a}}_{\bar{i}}\, {}^{A}t^{b}_{m}\, {}^{A}t^{n\bar{m}}_{j\bar{n}} + {}^{A}t^{\bar{a}}_{\bar{i}}\, {}^{A}t^{n}_{j}\, {}^{A}t^{b\bar{m}}_{m\bar{n}} - {}^{A}t^{\bar{a}}_{\bar{i}}\, {}^{A}t^{n}_{m}\, {}^{A}t^{b\bar{m}}_{j\bar{n}} + {}^{A}t^{\bar{a}}_{\bar{i}}\, {}^{A}t^{\bar{m}}_{\bar{n}}\, {}^{A}t^{bn}_{mj} + {}^{A}t^{\bar{a}}_{\bar{i}}\, {}^{A}t^{b}_{m}\, {}^{A}t^{n}_{j}\, {}^{A}t^{\bar{m}}_{\bar{n}} \\
&- {}^{A}t^{\bar{a}}_{\bar{j}}\, {}^{A}t^{b}_{m}\, {}^{A}t^{n\bar{m}}_{i\bar{n}} - {}^{A}t^{\bar{a}}_{\bar{j}}\, {}^{A}t^{n}_{i}\, {}^{A}t^{b\bar{m}}_{m\bar{n}} + {}^{A}t^{\bar{a}}_{\bar{j}}\, {}^{A}t^{n}_{m}\, {}^{A}t^{b\bar{m}}_{i\bar{n}} - {}^{A}t^{\bar{a}}_{\bar{j}}\, {}^{A}t^{\bar{m}}_{\bar{n}}\, {}^{A}t^{bn}_{mi} - {}^{A}t^{\bar{a}}_{\bar{j}}\, {}^{A}t^{b}_{m}\, {}^{A}t^{n}_{i}\, {}^{A}t^{\bar{m}}_{\bar{n}} \\
&- {}^{A}t^{\bar{b}}_{\bar{i}}\, {}^{A}t^{a}_{m}\, {}^{A}t^{n\bar{m}}_{j\bar{n}} - {}^{A}t^{\bar{b}}_{\bar{i}}\, {}^{A}t^{n}_{j}\, {}^{A}t^{a\bar{m}}_{m\bar{n}} + {}^{A}t^{\bar{b}}_{\bar{i}}\, {}^{A}t^{n}_{m}\, {}^{A}t^{a\bar{m}}_{j\bar{n}} - {}^{A}t^{\bar{b}}_{\bar{i}}\, {}^{A}t^{\bar{m}}_{\bar{n}}\, {}^{A}t^{an}_{mj} - {}^{A}t^{\bar{b}}_{\bar{i}}\, {}^{A}t^{a}_{m}\, {}^{A}t^{n}_{j}\, {}^{A}t^{\bar{m}}_{\bar{n}} \\
&+ {}^{A}t^{\bar{b}}_{\bar{j}}\, {}^{A}t^{a}_{m}\, {}^{A}t^{n\bar{m}}_{i\bar{n}} + {}^{A}t^{\bar{b}}_{\bar{j}}\, {}^{A}t^{n}_{i}\, {}^{A}t^{a\bar{m}}_{m\bar{n}} - {}^{A}t^{\bar{b}}_{\bar{j}}\, {}^{A}t^{n}_{m}\, {}^{A}t^{a\bar{m}}_{i\bar{n}} + {}^{A}t^{\bar{b}}_{\bar{j}}\, {}^{A}t^{\bar{m}}_{\bar{n}}\, {}^{A}t^{an}_{mi} + {}^{A}t^{\bar{b}}_{\bar{j}}\, {}^{A}t^{a}_{m}\, {}^{A}t^{n}_{i}\, {}^{A}t^{\bar{m}}_{\bar{n}} \\
&- {}^{A}t^{a}_{i}\, {}^{A}t^{b}_{m}\, {}^{A}t^{n\bar{m}}_{j\bar{n}} - {}^{A}t^{a}_{i}\, {}^{A}t^{n}_{j}\, {}^{A}t^{b\bar{m}}_{m\bar{n}} + {}^{A}t^{a}_{i}\, {}^{A}t^{n}_{m}\, {}^{A}t^{b\bar{m}}_{j\bar{n}} - {}^{A}t^{a}_{i}\, {}^{A}t^{\bar{m}}_{\bar{n}}\, {}^{A}t^{bn}_{mj} - {}^{A}t^{a}_{i}\, {}^{A}t^{b}_{m}\, {}^{A}t^{n}_{j}\, {}^{A}t^{\bar{m}}_{\bar{n}} \\
&+ {}^{A}t^{a}_{j}\, {}^{A}t^{b}_{m}\, {}^{A}t^{n\bar{m}}_{i\bar{n}} + {}^{A}t^{a}_{j}\, {}^{A}t^{n}_{i}\, {}^{A}t^{b\bar{m}}_{m\bar{n}} - {}^{A}t^{a}_{j}\, {}^{A}t^{n}_{m}\, {}^{A}t^{b\bar{m}}_{i\bar{n}} + {}^{A}t^{a}_{j}\, {}^{A}t^{\bar{m}}_{\bar{n}}\, {}^{A}t^{bn}_{mi} + {}^{A}t^{a}_{j}\, {}^{A}t^{b}_{m}\, {}^{A}t^{n}_{i}\, {}^{A}t^{\bar{m}}_{\bar{n}} \\
&+ {}^{A}t^{b}_{i}\, {}^{A}t^{a}_{m}\, {}^{A}t^{n\bar{m}}_{j\bar{n}} + {}^{A}t^{b}_{i}\, {}^{A}t^{n}_{j}\, {}^{A}t^{a\bar{m}}_{m\bar{n}} - {}^{A}t^{b}_{i}\, {}^{A}t^{n}_{m}\, {}^{A}t^{a\bar{m}}_{j\bar{n}} + {}^{A}t^{b}_{i}\, {}^{A}t^{\bar{m}}_{\bar{n}}\, {}^{A}t^{an}_{mj} + {}^{A}t^{b}_{i}\, {}^{A}t^{a}_{m}\, {}^{A}t^{n}_{j}\, {}^{A}t^{\bar{m}}_{\bar{n}} \\
&- {}^{A}t^{b}_{j}\, {}^{A}t^{a}_{m}\, {}^{A}t^{n\bar{m}}_{i\bar{n}} - {}^{A}t^{b}_{j}\, {}^{A}t^{n}_{i}\, {}^{A}t^{a\bar{m}}_{m\bar{n}} + {}^{A}t^{b}_{j}\, {}^{A}t^{n}_{m}\, {}^{A}t^{a\bar{m}}_{i\bar{n}} - {}^{A}t^{b}_{j}\, {}^{A}t^{\bar{m}}_{\bar{n}}\, {}^{A}t^{an}_{mi} - {}^{A}t^{b}_{j}\, {}^{A}t^{a}_{m}\, {}^{A}t^{n}_{i}\, {}^{A}t^{\bar{m}}_{\bar{n}}\Big] \\
&+ \delta(\bar{m},\bar{b})\,\Big[+ {}^{A}t^{\bar{a}}_{\bar{i}}\, {}^{A}t^{n\bar{m}}_{j\bar{n}} + {}^{A}t^{\bar{a}}_{\bar{i}}\, {}^{A}t^{n}_{j}\, {}^{A}t^{\bar{m}}_{\bar{n}} - {}^{A}t^{\bar{a}}_{\bar{j}}\, {}^{A}t^{n\bar{m}}_{i\bar{n}} - {}^{A}t^{\bar{a}}_{\bar{j}}\, {}^{A}t^{n}_{i}\, {}^{A}t^{\bar{m}}_{\bar{n}} - {}^{A}t^{\bar{m}}_{\bar{i}}\, {}^{A}t^{a}_{m}\, {}^{A}t^{n\bar{m}}_{j\bar{n}} \\
&- {}^{A}t^{\bar{m}}_{\bar{i}}\, {}^{A}t^{n}_{j}\, {}^{A}t^{a\bar{m}}_{m\bar{n}} + {}^{A}t^{\bar{m}}_{\bar{i}}\, {}^{A}t^{n}_{m}\, {}^{A}t^{a\bar{m}}_{j\bar{n}} - {}^{A}t^{\bar{m}}_{\bar{i}}\, {}^{A}t^{\bar{m}}_{\bar{n}}\, {}^{A}t^{an}_{mj} - {}^{A}t^{\bar{m}}_{\bar{i}}\, {}^{A}t^{a}_{m}\, {}^{A}t^{n}_{j}\, {}^{A}t^{\bar{m}}_{\bar{n}} \\
&+ {}^{A}t^{\bar{m}}_{\bar{j}}\, {}^{A}t^{a}_{m}\, {}^{A}t^{n\bar{m}}_{i\bar{n}} + {}^{A}t^{\bar{m}}_{\bar{j}}\, {}^{A}t^{n}_{i}\, {}^{A}t^{a\bar{m}}_{m\bar{n}} - {}^{A}t^{\bar{m}}_{\bar{j}}\, {}^{A}t^{n}_{m}\, {}^{A}t^{a\bar{m}}_{i\bar{n}} + {}^{A}t^{\bar{m}}_{\bar{j}}\, {}^{A}t^{\bar{m}}_{\bar{n}}\, {}^{A}t^{an}_{mi} + {}^{A}t^{\bar{m}}_{\bar{j}}\, {}^{A}t^{a}_{m}\, {}^{A}t^{n}_{i}\, {}^{A}t^{\bar{m}}_{\bar{n}} \\
&- {}^{A}t^{a}_{i}\, {}^{A}t^{n\bar{m}}_{j\bar{n}} - {}^{A}t^{a}_{i}\, {}^{A}t^{n}_{j}\, {}^{A}t^{\bar{m}}_{\bar{n}} + {}^{A}t^{a}_{j}\, {}^{A}t^{n\bar{m}}_{i\bar{n}} + {}^{A}t^{a}_{j}\, {}^{A}t^{n}_{i}\, {}^{A}t^{\bar{m}}_{\bar{n}}\Big] \\
&+ \delta(\bar{n},\bar{j})\,\Big[- {}^{A}t^{\bar{a}}_{\bar{i}}\, {}^{A}t^{b\bar{m}}_{m\bar{n}} - {}^{A}t^{\bar{a}}_{\bar{i}}\, {}^{A}t^{b}_{m}\, {}^{A}t^{\bar{m}}_{\bar{n}} - {}^{A}t^{\bar{a}}_{\bar{n}}\, {}^{A}t^{b}_{m}\, {}^{A}t^{n\bar{m}}_{i\bar{n}} - {}^{A}t^{\bar{a}}_{\bar{n}}\, {}^{A}t^{n}_{i}\, {}^{A}t^{b\bar{m}}_{m\bar{n}} + {}^{A}t^{\bar{a}}_{\bar{n}}\, {}^{A}t^{n}_{m}\, {}^{A}t^{b\bar{m}}_{i\bar{n}} \\
&- {}^{A}t^{\bar{a}}_{\bar{n}}\, {}^{A}t^{\bar{m}}_{\bar{n}}\, {}^{A}t^{bn}_{mi} - {}^{A}t^{\bar{a}}_{\bar{n}}\, {}^{A}t^{b}_{m}\, {}^{A}t^{n}_{i}\, {}^{A}t^{\bar{m}}_{\bar{n}} + {}^{A}t^{\bar{b}}_{\bar{i}}\, {}^{A}t^{a\bar{m}}_{m\bar{n}} + {}^{A}t^{\bar{b}}_{\bar{i}}\, {}^{A}t^{a}_{m}\, {}^{A}t^{\bar{m}}_{\bar{n}} + {}^{A}t^{\bar{b}}_{\bar{n}}\, {}^{A}t^{a}_{m}\, {}^{A}t^{n\bar{m}}_{i\bar{n}} \\
&+ {}^{A}t^{\bar{b}}_{\bar{n}}\, {}^{A}t^{n}_{i}\, {}^{A}t^{a\bar{m}}_{m\bar{n}} - {}^{A}t^{\bar{b}}_{\bar{n}}\, {}^{A}t^{n}_{m}\, {}^{A}t^{a\bar{m}}_{i\bar{n}} + {}^{A}t^{\bar{b}}_{\bar{n}}\, {}^{A}t^{\bar{m}}_{\bar{n}}\, {}^{A}t^{an}_{mi} + {}^{A}t^{\bar{b}}_{\bar{n}}\, {}^{A}t^{a}_{m}\, {}^{A}t^{n}_{i}\, {}^{A}t^{\bar{m}}_{\bar{n}} \\
&+ {}^{A}t^{a}_{i}\, {}^{A}t^{b\bar{m}}_{m\bar{n}} + {}^{A}t^{a}_{i}\, {}^{A}t^{b}_{m}\, {}^{A}t^{\bar{m}}_{\bar{n}} - {}^{A}t^{b}_{i}\, {}^{A}t^{a\bar{m}}_{m\bar{n}} - {}^{A}t^{b}_{i}\, {}^{A}t^{a}_{m}\, {}^{A}t^{\bar{m}}_{\bar{n}}\Big] \\
&+ \delta(\bar{m},\bar{a})\,\Big[+ {}^{A}t^{\bar{m}}_{\bar{i}}\, {}^{A}t^{b}_{m}\, {}^{A}t^{n\bar{m}}_{j\bar{n}} + {}^{A}t^{\bar{m}}_{\bar{i}}\, {}^{A}t^{n}_{j}\, {}^{A}t^{b\bar{m}}_{m\bar{n}} - {}^{A}t^{\bar{m}}_{\bar{i}}\, {}^{A}t^{n}_{m}\, {}^{A}t^{b\bar{m}}_{j\bar{n}} + {}^{A}t^{\bar{m}}_{\bar{i}}\, {}^{A}t^{\bar{m}}_{\bar{n}}\, {}^{A}t^{bn}_{mj} + {}^{A}t^{\bar{m}}_{\bar{i}}\, {}^{A}t^{b}_{m}\, {}^{A}t^{n}_{j}\, {}^{A}t^{\bar{m}}_{\bar{n}} \\
&- {}^{A}t^{\bar{m}}_{\bar{j}}\, {}^{A}t^{b}_{m}\, {}^{A}t^{n\bar{m}}_{i\bar{n}} - {}^{A}t^{\bar{m}}_{\bar{j}}\, {}^{A}t^{n}_{i}\, {}^{A}t^{b\bar{m}}_{m\bar{n}} + {}^{A}t^{\bar{m}}_{\bar{j}}\, {}^{A}t^{n}_{m}\, {}^{A}t^{b\bar{m}}_{i\bar{n}} - {}^{A}t^{\bar{m}}_{\bar{j}}\, {}^{A}t^{\bar{m}}_{\bar{n}}\, {}^{A}t^{bn}_{mi} - {}^{A}t^{\bar{m}}_{\bar{j}}\, {}^{A}t^{b}_{m}\, {}^{A}t^{n}_{i}\, {}^{A}t^{\bar{m}}_{\bar{n}} \\
&- {}^{A}t^{\bar{b}}_{\bar{i}}\, {}^{A}t^{n\bar{m}}_{j\bar{n}} - {}^{A}t^{\bar{b}}_{\bar{i}}\, {}^{A}t^{n}_{j}\, {}^{A}t^{\bar{m}}_{\bar{n}} + {}^{A}t^{\bar{b}}_{\bar{j}}\, {}^{A}t^{n\bar{m}}_{i\bar{n}} + {}^{A}t^{\bar{b}}_{\bar{j}}\, {}^{A}t^{n}_{i}\, {}^{A}t^{\bar{m}}_{\bar{n}} + {}^{A}t^{b}_{i}\, {}^{A}t^{n\bar{m}}_{j\bar{n}} + {}^{A}t^{b}_{i}\, {}^{A}t^{n}_{j}\, {}^{A}t^{\bar{m}}_{\bar{n}} \\
&- {}^{A}t^{b}_{j}\, {}^{A}t^{n\bar{m}}_{i\bar{n}} - {}^{A}t^{b}_{j}\, {}^{A}t^{n}_{i}\, {}^{A}t^{\bar{m}}_{\bar{n}}\Big] \\
&+ \delta(\bar{n},\bar{i})\,\Big[+ {}^{A}t^{\bar{a}}_{\bar{n}}\, {}^{A}t^{b}_{m}\, {}^{A}t^{n\bar{m}}_{j\bar{n}} + {}^{A}t^{\bar{a}}_{\bar{n}}\, {}^{A}t^{n}_{j}\, {}^{A}t^{b\bar{m}}_{m\bar{n}} - {}^{A}t^{\bar{a}}_{\bar{n}}\, {}^{A}t^{n}_{m}\, {}^{A}t^{b\bar{m}}_{j\bar{n}} + {}^{A}t^{\bar{a}}_{\bar{n}}\, {}^{A}t^{\bar{m}}_{\bar{n}}\, {}^{A}t^{bn}_{mj} + {}^{A}t^{\bar{a}}_{\bar{n}}\, {}^{A}t^{b}_{m}\, {}^{A}t^{n}_{j}\, {}^{A}t^{\bar{m}}_{\bar{n}} \\
&+ {}^{A}t^{\bar{a}}_{\bar{j}}\, {}^{A}t^{b\bar{m}}_{m\bar{n}} + {}^{A}t^{\bar{a}}_{\bar{j}}\, {}^{A}t^{b}_{m}\, {}^{A}t^{\bar{m}}_{\bar{n}} - {}^{A}t^{\bar{b}}_{\bar{n}}\, {}^{A}t^{a}_{m}\, {}^{A}t^{n\bar{m}}_{j\bar{n}} - {}^{A}t^{\bar{b}}_{\bar{n}}\, {}^{A}t^{n}_{j}\, {}^{A}t^{a\bar{m}}_{m\bar{n}} + {}^{A}t^{\bar{b}}_{\bar{n}}\, {}^{A}t^{n}_{m}\, {}^{A}t^{a\bar{m}}_{j\bar{n}} \\
&- {}^{A}t^{\bar{b}}_{\bar{n}}\, {}^{A}t^{\bar{m}}_{\bar{n}}\, {}^{A}t^{an}_{mj} - {}^{A}t^{\bar{b}}_{\bar{n}}\, {}^{A}t^{a}_{m}\, {}^{A}t^{n}_{j}\, {}^{A}t^{\bar{m}}_{\bar{n}} - {}^{A}t^{\bar{b}}_{\bar{j}}\, {}^{A}t^{a\bar{m}}_{m\bar{n}} - {}^{A}t^{\bar{b}}_{\bar{j}}\, {}^{A}t^{a}_{m}\, {}^{A}t^{\bar{m}}_{\bar{n}} - {}^{A}t^{a}_{j}\, {}^{A}t^{b\bar{m}}_{m\bar{n}} \\
&- {}^{A}t^{a}_{j}\, {}^{A}t^{b}_{m}\, {}^{A}t^{\bar{m}}_{\bar{n}} + {}^{A}t^{b}_{j}\, {}^{A}t^{a\bar{m}}_{m\bar{n}} + {}^{A}t^{b}_{j}\, {}^{A}t^{a}_{m}\, {}^{A}t^{\bar{m}}_{\bar{n}}\Big] \\
&+ \delta(\bar{n},\bar{j})\,\delta(\bar{m},\bar{b})\,\Big[- {}^{A}t^{\bar{a}}_{\bar{i}}\, {}^{A}t^{\bar{m}}_{\bar{n}} - {}^{A}t^{\bar{a}}_{\bar{n}}\, {}^{A}t^{n\bar{m}}_{i\bar{n}} - {}^{A}t^{\bar{a}}_{\bar{n}}\, {}^{A}t^{n}_{i}\, {}^{A}t^{\bar{m}}_{\bar{n}} + {}^{A}t^{\bar{m}}_{\bar{i}}\, {}^{A}t^{a\bar{m}}_{m\bar{n}} + {}^{A}t^{\bar{m}}_{\bar{i}}\, {}^{A}t^{a}_{m}\, {}^{A}t^{\bar{m}}_{\bar{n}} \\
&+ {}^{A}t^{\bar{m}}_{\bar{n}}\, {}^{A}t^{a}_{m}\, {}^{A}t^{n\bar{m}}_{i\bar{n}} + {}^{A}t^{\bar{m}}_{\bar{n}}\, {}^{A}t^{n}_{i}\, {}^{A}t^{a\bar{m}}_{m\bar{n}} - {}^{A}t^{\bar{m}}_{\bar{n}}\, {}^{A}t^{n}_{m}\, {}^{A}t^{a\bar{m}}_{i\bar{n}} + {}^{A}t^{\bar{m}}_{\bar{n}}\, {}^{A}t^{\bar{m}}_{\bar{n}}\, {}^{A}t^{an}_{mi} + {}^{A}t^{\bar{m}}_{\bar{n}}\, {}^{A}t^{a}_{m}\, {}^{A}t^{n}_{i}\, {}^{A}t^{\bar{m}}_{\bar{n}} \\
&+ {}^{A}t^{a}_{i}\, {}^{A}t^{\bar{m}}_{\bar{n}}\Big] \\
&+ \delta(\bar{n},\bar{j})\,\delta(\bar{m},\bar{a})\,\Big[- {}^{A}t^{\bar{m}}_{\bar{i}}\, {}^{A}t^{b\bar{m}}_{m\bar{n}} - {}^{A}t^{\bar{m}}_{\bar{i}}\, {}^{A}t^{b}_{m}\, {}^{A}t^{\bar{m}}_{\bar{n}} - {}^{A}t^{\bar{m}}_{\bar{n}}\, {}^{A}t^{b}_{m}\, {}^{A}t^{n\bar{m}}_{i\bar{n}} - {}^{A}t^{\bar{m}}_{\bar{n}}\, {}^{A}t^{n}_{i}\, {}^{A}t^{b\bar{m}}_{m\bar{n}} + {}^{A}t^{\bar{m}}_{\bar{n}}\, {}^{A}t^{n}_{m}\, {}^{A}t^{b\bar{m}}_{i\bar{n}} \\
&- {}^{A}t^{\bar{m}}_{\bar{n}}\, {}^{A}t^{\bar{m}}_{\bar{n}}\, {}^{A}t^{bn}_{mi} - {}^{A}t^{\bar{m}}_{\bar{n}}\, {}^{A}t^{b}_{m}\, {}^{A}t^{n}_{i}\, {}^{A}t^{\bar{m}}_{\bar{n}} + {}^{A}t^{\bar{b}}_{\bar{i}}\, {}^{A}t^{\bar{m}}_{\bar{n}} + {}^{A}t^{\bar{b}}_{\bar{n}}\, {}^{A}t^{n\bar{m}}_{i\bar{n}} + {}^{A}t^{\bar{b}}_{\bar{n}}\, {}^{A}t^{n}_{i}\, {}^{A}t^{\bar{m}}_{\bar{n}} \\
&- {}^{A}t^{b}_{i}\, {}^{A}t^{\bar{m}}_{\bar{n}}\Big] \\
&+ \delta(\bar{n},\bar{i})\,\delta(\bar{m},\bar{b})\,\Big[+ {}^{A}t^{\bar{a}}_{\bar{n}}\, {}^{A}t^{n\bar{m}}_{j\bar{n}} + {}^{A}t^{\bar{a}}_{\bar{n}}\, {}^{A}t^{n}_{j}\, {}^{A}t^{\bar{m}}_{\bar{n}} + {}^{A}t^{\bar{a}}_{\bar{j}}\, {}^{A}t^{\bar{m}}_{\bar{n}} - {}^{A}t^{\bar{m}}_{\bar{n}}\, {}^{A}t^{a}_{m}\, {}^{A}t^{n\bar{m}}_{j\bar{n}} - {}^{A}t^{\bar{m}}_{\bar{n}}\, {}^{A}t^{n}_{j}\, {}^{A}t^{a\bar{m}}_{m\bar{n}} \\
&+ {}^{A}t^{\bar{m}}_{\bar{n}}\, {}^{A}t^{n}_{m}\, {}^{A}t^{a\bar{m}}_{j\bar{n}} - {}^{A}t^{\bar{m}}_{\bar{n}}\, {}^{A}t^{\bar{m}}_{\bar{n}}\, {}^{A}t^{an}_{mj} - {}^{A}t^{\bar{m}}_{\bar{n}}\, {}^{A}t^{a}_{m}\, {}^{A}t^{n}_{j}\, {}^{A}t^{\bar{m}}_{\bar{n}} - {}^{A}t^{\bar{m}}_{\bar{j}}\, {}^{A}t^{a\bar{m}}_{m\bar{n}} - {}^{A}t^{\bar{m}}_{\bar{j}}\, {}^{A}t^{a}_{m}\, {}^{A}t^{\bar{m}}_{\bar{n}} \\
&- {}^{A}t^{a}_{j}\, {}^{A}t^{\bar{m}}_{\bar{n}}\Big] \\
&+ \delta(\bar{n},\bar{i})\,\delta(\bar{m},\bar{a})\,\Big[+ {}^{A}t^{\bar{m}}_{\bar{n}}\, {}^{A}t^{b}_{m}\, {}^{A}t^{n\bar{m}}_{j\bar{n}} + {}^{A}t^{\bar{m}}_{\bar{n}}\, {}^{A}t^{n}_{j}\, {}^{A}t^{b\bar{m}}_{m\bar{n}} - {}^{A}t^{\bar{m}}_{\bar{n}}\, {}^{A}t^{n}_{m}\, {}^{A}t^{b\bar{m}}_{j\bar{n}} + {}^{A}t^{\bar{m}}_{\bar{n}}\, {}^{A}t^{\bar{m}}_{\bar{n}}\, {}^{A}t^{bn}_{mj} + {}^{A}t^{\bar{m}}_{\bar{n}}\, {}^{A}t^{b}_{m}\, {}^{A}t^{n}_{j}\, {}^{A}t^{\bar{m}}_{\bar{n}} \\
&+ {}^{A}t^{\bar{m}}_{\bar{j}}\, {}^{A}t^{b\bar{m}}_{m\bar{n}} + {}^{A}t^{\bar{m}}_{\bar{j}}\, {}^{A}t^{b}_{m}\, {}^{A}t^{\bar{m}}_{\bar{n}} - {}^{A}t^{\bar{b}}_{\bar{n}}\, {}^{A}t^{n\bar{m}}_{j\bar{n}} - {}^{A}t^{\bar{b}}_{\bar{n}}\, {}^{A}t^{n}_{j}\, {}^{A}t^{\bar{m}}_{\bar{n}} - {}^{A}t^{\bar{b}}_{\bar{j}}\, {}^{A}t^{\bar{m}}_{\bar{n}} \\
&+ {}^{A}t^{b}_{j}\, {}^{A}t^{\bar{m}}_{\bar{n}}\Big]
\end{aligned}
\tag{S72}
$$
